# Supplementary material for: Multiple-Valued Logic Circuit Design and Data Transmission Intended for Embedded Systems
Source: arXiv:2211.04542 source file (2022-11-08)
Supplement: Supplementary file 1 [file CascadingTHA_TMUX.pdf]

Microelectronics Journal 96 (2020) 104698

Contents lists available at ScienceDirect

Microelectronics Journal

journal homepage: www.elsevier.com/locate/mejo

# CNFET-based designs of Ternary Half-Adder using a novel "decoder-less" ternary multiplexer based on unary operators

Ramzi A. Jaber [a,*], Ahmad M. El-Hajj [a], Abdallah Kassem [b], Lina A. Nimri [c], Ali M. Haidar [a]

[a] *Depart. of Electrical & Computer Eng., Beirut Arab University (BAU), Debbieh, Lebanon*
[b] *Depart. of Electrical & Computer Eng., Notre Dame University (NDU), Louaize, Lebanon*
[c] *Department of Business Computer, Lebanese University, Beirut, Lebanon*

ARTICLE INFO

*Keywords:*
Carbon Nano-Tube Field Effect Transistors (CNFET)
Combinational logic circuit
Multi-Valued Logic (MVL)
Noise immunity curve
Process variations
Ternary MUX
Unary operators
VLSI

ABSTRACT

Multi-valued logic (MVL) has more than two-valued logic to decrease the interconnections and energy consumption. Also, the market has seen a significant increase in portable electronics and embedded systems, which depend on batteries. Therefore, this paper proposes 32 nm channel CNFET-Based a Ternary Half Adder (THA) and a "decoder-less" Ternary Multiplexer (TMUX) using the proposed Unary Operator aiming to decrease the power-delay product (PDP) to preserve battery consumption; Simulations performed using the HSPICE simulator for voltage variation, temperature variation, and frequency variation. The results demonstrate the advantage of proposed models with a reduction of 46.4% in transistors count for the THA and 57.3%, and 99.3% in energy consumption (PDP) for the TMUX, and THA, respectively. Moreover, the noise immunity curve (NIC) and Monte Carlo analysis for major process variations (TOX, CNT Diameter, CNT's Count, and Channel length) were studied. The results confirmed that the proposed THA had higher robustness and higher noise tolerance, among other designs.

## 1. Introduction

Binary circuits suffer from high-power consumption because of a massive number of interconnections that increase power consumption. Whereas, Multi-Valued Logic (MVL) circuits have more than two-valued logic to reduce interconnections, chip area, and power consumption [1].

In addition, the authors of [2] has proven that the ternary system is the most efficient in circuit complexity and cost compared to other bases.

MVL has attracted researchers' concern over binary logic. MVL can be implemented in communication system [3], cloud vehicular networks [4], wireless sensor networks [5], circuit designs such as Logic Gates, Memory, Memristor circuit [6–8], and software (algorithm) [9,10].

Carbon Nano-Tube Field Effect Transistors (CNFET) provides the best trade-off in terms of energy efficiency and circuit speed [11] compared to CMOS [12,13], and FinFet [14].

Thus, this paper uses CNFET technology to design the ternary combinational logic circuits and will compare to the CNFET-based designs in Refs. [15–18].

In particular, compared to our previous work in Ref. [16], the proposed ternary half adder (THA) significantly reduces the energy consumption (PDP) by adopting a new design paradigm relying on cascading of the proposed ternary multiplexer (TMUX) rather than utilizing a ternary decoder and basic logic gates as was done in Ref. [16].

In Ref. [15], presented CNFET-based ternary decoder (TDecoder) with 16 transistors, and ternary half adder (THA) with 136 CNFETs whereas in our previous work [16], proposed a novel TDecoder with 9 CNFETs, and THA with 85 CNFETs. Both papers [15,16], use TDecoder and basic logic gates like AND, OR, and NAND to design their THA.

However, in Ref. [17], the (3:1) ternary multiplexer (TMUX) based on a TDecoder proposed with 28 CNFETs, and THA with 168 CNFETs using cascading TMUXs while in Ref. [18], presented the (3:1) ternary multiplexer without using TDecoder with 18 CNFETs.

The above existing designs suffer from high-energy consumption either due to a large number of transistors [15,17,18] or transistor arrangement [16].

* Corresponding author.
*E-mail address:* r.jaber@ieee.org (R.A. Jaber).

https://doi.org/10.1016/j.mejo.2019.104698
Received 1 August 2019; Received in revised form 13 December 2019; Accepted 29 December 2019
Available online XXX
0026-2692/© 2019 Published by Elsevier Ltd.

Thus, this paper proposes a novel "decoder-less" (3:1) TMUX with 15 CNFETs using unary operators of Ternary system, and THA with 90 CNFETs.

The new designs offer a considerable gain in terms of system performance compared to the designs in Refs. [15–18], as shown in the HSPICE-based simulation results and get the lowest PDP.

The rest of the paper is organized as follows: Section 2 provides a background of CNFETs and Unary Operators, while Section 3 and Section 4 describes the proposed Unary Operator and the proposed combinational logic circuits, respectively. Section 5 discusses the simulation results and comparisons, followed by the Conclusion.

## 2. Background

### 2.1. CNFET design

Details about the Stanford CNFET model used in this work can be found in Refs. [19–21]. However, it merits referencing that the CNFETs use a semiconducting single-walled CNT as a channel for conduction. Also, "CNFET demonstrates better performance based on the intrinsic CV/I gate-delay metric, fourteen times for P-FET, and six times for N-FET than the MOSFET, even with device nonidealities. Compared to CMOS circuits, the CNFET circuits with one to ten CNTs per device is about two to ten times faster, the energy consumption per cycle is about seven to two times lower, considering the realistic layout pattern and the interconnect capacitance."

The angle of atom arrangement along the tube in a single-walled CNT (SWCNT) is a chirality vector represented by the integer pair $(i, j)$. This chirality vector measures if the CNT is metallic or semiconducting; if $i = j$ or $i–j = 3t$, where $t$ is an integer, then the nanotube is metallic else it is semiconducting.

The CNFET diameter can be calculated from the equation in (1):

$$D_{\text{cnt}} = \frac{\sqrt{3} \cdot a_0}{\pi} \sqrt{i^2 + j^2 + ij} \tag{1}$$

Where $a_0 = 0.142$ nm is the inter-atomic distance between each carbon atom and its neighbor, and the integer pair ($i$, $j$) represents the chirality vector. The characteristics of the CNFET model are identical to MOSFETs. Except for the threshold voltage, which is calculated by the following equation (2):

$$V_{\text{th}} = \frac{E_g}{2 \cdot e} = \frac{\sqrt{3}}{3} \frac{a \cdot V\pi}{e \cdot Dcnt} \tag{2}$$

Where $a = 2.49$ Å is the carbon to carbon atom distance, $V\pi = 3.033$ eV is the carbon bond energy in the tight binding model, $e$ is the electron charge unit, and $Dcnt$ is the CNT diameter.

In general, three chiralities can be used in the ternary system. The relationship between the chirality, diameter, and threshold voltage are shown in Table 1.

### 2.2. Unary operators of ternary systems

To the best of our knowledge, the literature review about unary operators of MVL is limited. It was formally defined in Ref. [22] as the number of one-place, or unary, functions of a $p$-valued logic system is $p^p$.

**Table 1**
The relation between the chirality, diameter, and threshold voltage, as calculated in Refs.: [15,16].

| Chirality | CNT diameter | Threshold voltage N-CNFET | Threshold voltage P-CNFET |
|---|---|---|---|
| (19,0) | 1.487 nm | 0.289 V | - 0.289 V |
| (13,0) | 1.018 nm | 0.428 V | - 0.428 V |
| (10,0) | 0.783 nm | 0.559 V | - 0.559 V |

For binary systems where $p = 2$, there are only four unary functions, the identity "01", negation "10", and the two constant functions "00" and "11". Whereas, for ternary systems where $p = 3$, there are twenty-seven ($3^3$) unary functions.

Ternary logic systems can be represented in two ways: balanced (−1, 0, 1) corresponding to (-Vdd, 0, Vdd), and standard (0, 1, 2) corresponding to (0, Vdd/2, Vdd).

The selected four unary operators are described in Table 2 and derived from (3) to be used later for designing TMUX in Section IV-A.

**Table 2**
Truth table of the selected Unary Operators.

| Ternary Input $A$ | PTI $A_p$ | NTI $A_n$ | STI $\overline{A}$ | $A_1$ |
|---|---|---|---|---|
| Logic 0 (0 V) | 2 | 2 | 2 | 0 |
| Logic 1 (0.45 V) | 2 | 0 | 1 | 2 |
| Logic 2 (0.9 V) | 0 | 0 | 0 | 0 |

**Table 3**
The Chirality, diameter, and threshold voltage of the CNTs used in the proposed Unary Operator.

| CNFET Type | Chirality | Diameter | $V_{th}$ |
|---|---|---|---|
| P-CNFET (T1) | (19,0) | 1.487 nm | - 0.289 V |
| N-CNFET (T2) | (19,0) | 1.487 nm | 0.289 V |
| N-CNFET (T3) | (10,0) | 0.783 nm | 0.559 V |

The first three unary functions are three types of ternary inverters, the first is a positive ternary inverter (PTI), $A_p$, the second is a negative ternary inverter (NTI), $A_n$, and the third one is a standard ternary inverter (STI), which is the complement of $A$, $\overline{A}$. The fourth function is the Decisive literal, $A_1$.

$$\begin{aligned} A_p &= \begin{cases} 2, & if A \neq 2 \\ 0, & if A = 2 \end{cases} \\ A_n &= \begin{cases} 2, & if A = 0 \\ 0, & if A \neq 0 \end{cases} \\ \overline{A} &= \quad 2 - A \\ A_1 &= \begin{cases} 2, & if A = 1 \\ 0, & if A \neq 1 \end{cases} \end{aligned} \tag{3}$$

where $A \in \{0, 1, 2\}$.

## 3. Proposed unary operators of ternary systems

The existing Unary Operators designs in Ref. [15] is shown in Fig. 1. It shows three types of ternary inverters circuits and the three outputs of the proposed Ternary Decoder: $A_p$, $A_n$, $\overline{A}$, $A_0 = A_n$, $A_1$, and $A_2$.

This paper will not use $\overline{A}$, and $A_2$, we will focus on $A_1$, which generates from Ternary NOR with ten transistors, as shown in Fig. 1.

This section proposes a new design for $A_1$ with only three transistors, as shown in Fig. 2 with the transistor level design.

The chirality, diameter, and threshold voltage ($V_{th}$) of the CNFETs used in Fig. 2 are shown in Table 3.

When the voltage of the gate varies (0 V, 0.45 V, 0.9 V), then the transistor will be turned ON or OFF. It depends on the type and the diameter of CNFET. The operation of CNFETs transistor for D1 = 1.487 nm and D2 = 0.78 nm describes in Table 4.

The operations of the proposed unary operators are summarised in Table 5.

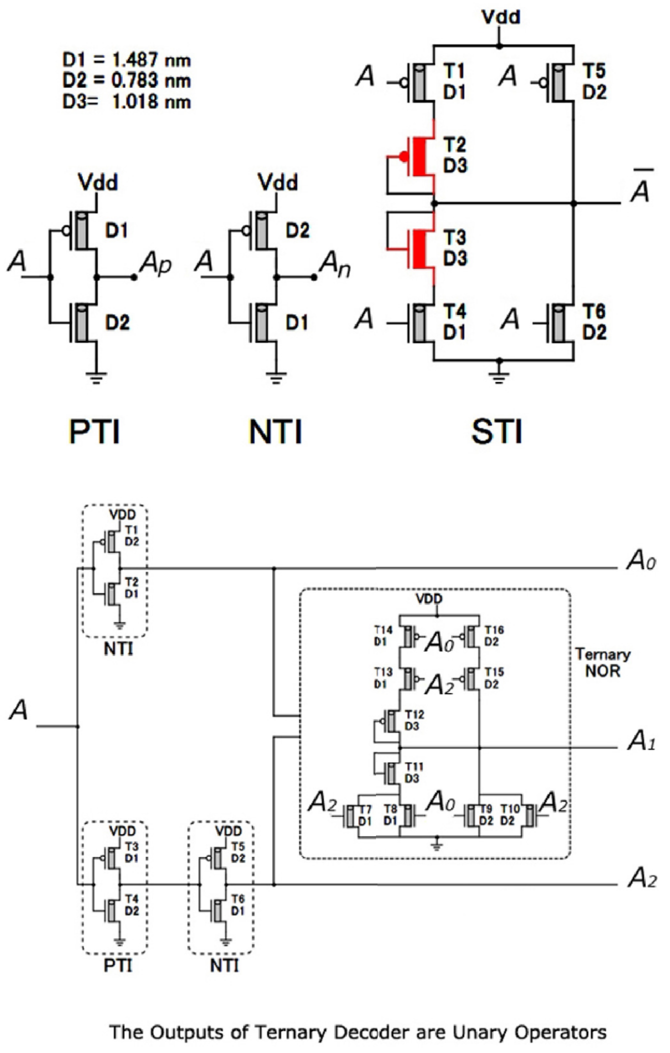


**Fig. 1.** Existing unary operators in Ref. [15]: $A_p$, $A_n$, $\overline{A}$, $A_0$, $A_1$, and $A_2$.

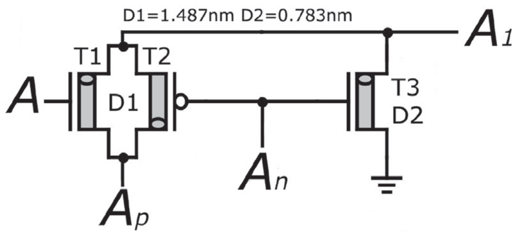


**Fig. 2.** The Transistor Level of the proposed Unary Operator $A_1$.

## 4. Proposed combinational circuits

This paper proposes some of the combinational circuits like TMUX and THA.

**Table 4**
The State of CNFETs with D1 = 1.487 nm and D2 = 0.783 nm.

| CNFET Type | Diameter | Voltage Gate 0 (0 V) | 1 (0.45 V) | 2 (0.9 V) |
|---|---|---|---|---|
| P-CNFET | D2 | ON | OFF | OFF |
| | D1 | ON | ON | OFF |
| N-CNFET | D2 | OFF | OFF | ON |
| | D1 | OFF | ON | ON |

**Table 5**
Operation of the proposed unary operator $A_1$.

| $A$ | $A_n$ | $A_p$ | Transistors Turned ON | OFF | Output $A_1$ |
|---|---|---|---|---|---|
| 0 | 2 | 2 | T3 | T1,T2 | 0 |
| 1 | 0 | 2 | T1,T2 | T3 | $A_p = 2$ |
| 2 | 0 | 0 | T1,T2 | T3 | $A_p = 0$ |

### 4.1. Proposed ternary multiplexer

A Multiplexer (MUX) can select between several analog or digital input signals and forward it to a single output line.

The (3:1) Ternary Multiplexer (TMUX) is introduced with the general model as represented in Fig. 3, it has three inputs ($I_0$, $I_1$, $I_2$), one selection ($S$), and one output ($Z$) which depends on ($S$) as described in Equations (4) and (5).

$$Z = I_0.S_0 + I_1.S_1 + I_2.S_2 \tag{4}$$

$$Z = \begin{cases} I_0, & if \quad S = 0 \\ I_1, & if \quad S = 1 \\ I_2, & if \quad S = 2 \end{cases} \tag{5}$$

The existing (3:1) TMUX in Ref. [17], and [18] are shown in Fig. 4. Fig. 4 (a) shows the TMUX of [17] with 28 transistors, using the Ternary Decoder of [15] and Fig. 4 (b) shows the TMUX of [18] with 18 transistors without using the Ternary Decoder.

This section proposes the "decoder-less" (3:1) TMUX as shown in Fig. 5 with 15 transistors using unary operators, $S_n$, $S_p$, $S_1$, and the complement of $S_1$, $\overline{S_1}$. D1 and D2 are the selected diameters of CNTs used in the design.

The first nine transistors are: $S_n$ (2 transistors), $S_p$ (2 transistors), $S_1$ (3 transistors), and $\overline{S_1}$ (2 transistors), as described in Section 2 and Section 3. The detailed operation of the proposed (3:1) TMUX is shown in Table 6.

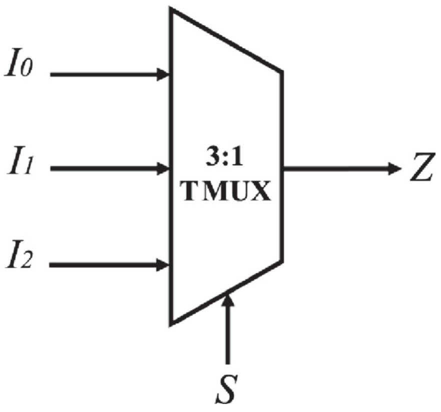


**Fig. 3.** The model of (3:1) TMUX.

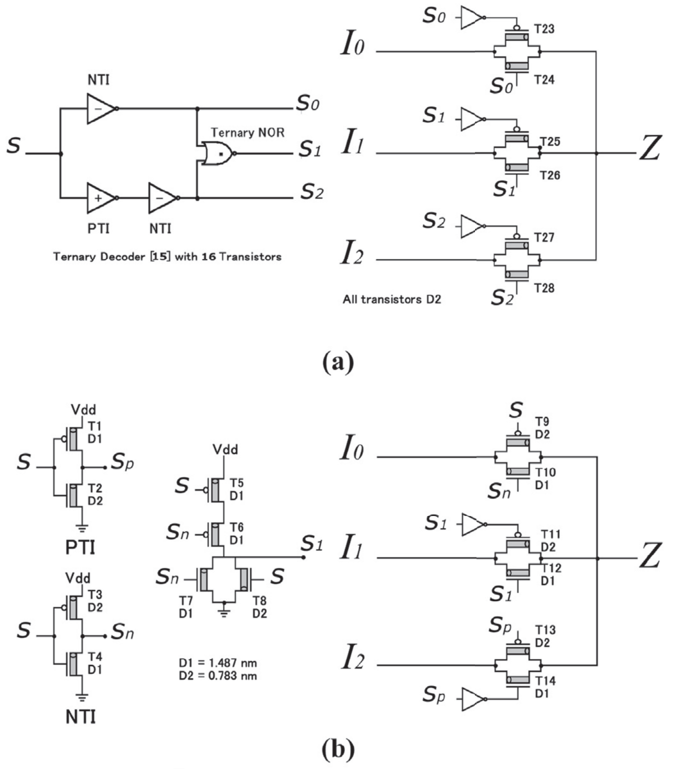


**Fig. 4.** Existing 3:1 TMUX: (a) In Ref. [17] with 28 transistors, (b) in Ref. [18] with 18 transistors.

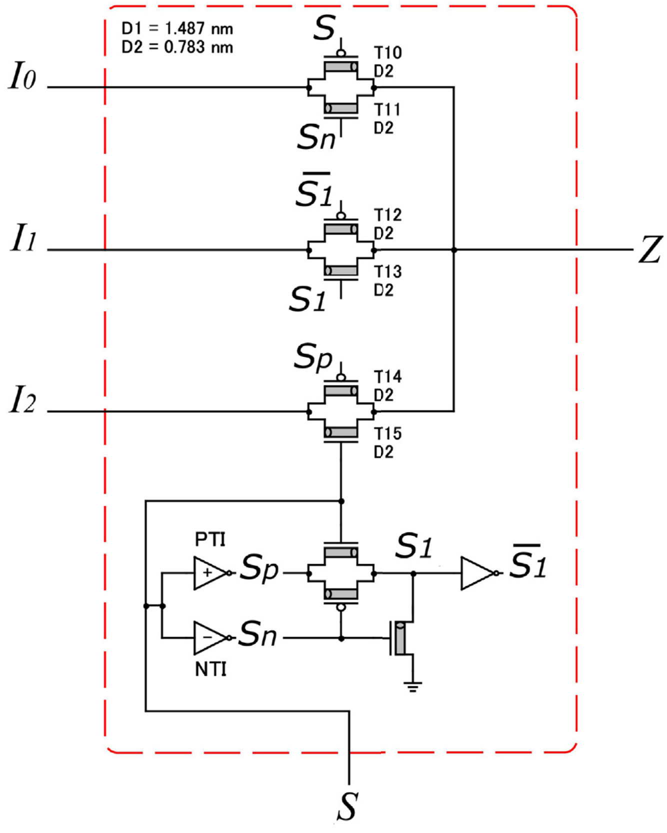


**Fig. 5.** Transistor Level of the proposed (3:1) TMUX with 15 CNFETs.

**Table 6**
The operation of the proposed (3:1) TMUX.

| Selection ($S$) | | 0 | 1 | 2 |
|---|---|---|---|---|
| $S_p$ | | 2 | 2 | 0 |
| $S_n$ | See Section 2 & 3 | 2 | 0 | 0 |
| $S_1$ | | 0 | 2 | 0 |
| $\overline{S_1}$ | | 2 | 0 | 2 |
| P-CNFET T10 | | ON | OFF | OFF |
| N-CNFET T11 | | ON | OFF | OFF |
| P-CNFET T12 | | OFF | ON | OFF |
| N-CNFET T13 | | OFF | ON | OFF |
| P-CNFET T14 | | OFF | OFF | ON |
| N-CNFET T15 | | OFF | OFF | ON |
| **Output ($Z$)** | | $I_0$ | $I_1$ | $I_2$ |

**Table 7**
Truth table of THA.

| A/B | $B_0(0)$ | $B_1(1)$ | $B_2(2)$ |
|---|---|---|---|
| | | Sum | |
| $A_0(0)$ | 0 | 1 | 2 |
| $A_1(1)$ | 1 | 2 | 0 |
| $A_2(2)$ | 2 | 0 | 1 |
| | | Carry | |
| A/B | $B_0(0)$ | $B_1(1)$ | $B_2(2)$ |
| $A_0(0)$ | 0 | 0 | 0 |
| $A_1(1)$ | 0 | 0 | 1 |
| $A_2(2)$ | 0 | 1 | 1 |

When the selection $S$ is logic 0 (0 V), then transistors (T10, T11) are turned ON, and (T12, T13, T14, T15) are turned OFF. Therefore, the output $Z$ is equal to the value of the input $I_0$.

When the selection $S$ is logic 1 (0.45 V), then transistors (T12, T13) are turned ON, and (T10, T11, T14, T15) are turned OFF. Therefore, the output $Z$ is equal to the value of the input $I_1$.

Finally, when the selection $S$ is logic 2 (0.9 V), then transistors (T14, T15) are turned ON, and (T10, T11, T12, T13) are turned OFF. Therefore, the output $Z$ is equal to the value of the input $I_2$.

### 4.2. Proposed ternary half adder

THA can add two ternary inputs and provides two outputs: the Sum and the Carry, as shown in Table 7.

The equations of the Sum and the Carry derived from Table 7 to design THA are:

1. Conventional design in Refs. [15,16] which uses Equation (6).
2. Cascading TMUXs design in Ref. [17] and in this work which uses Equation (7).

$$\begin{aligned} Sum &= 2 \bullet (A_0B_2 + A_1B_1 + A_2B_0) \\ &\quad +1 \bullet (A_0B_1 + A_1B_0 + A_2B_2) \\ Carry &= 1 \bullet (A_1B_2 + A_2B_1 + A_2B_2) \end{aligned} \tag{6}$$

$$\begin{aligned} Sum &= A.B_0 + (1.A_0 + 2.A_1 + 0.A_2).B_1 \\ &\quad +(2.A_0 + 0.A_1 + 1.A_2).B_2 \\ Carry &= 0.B_0 + (0.A_0 + 0.A_1 + 1.A_2).B_1 \\ &\quad +(0.A_0 + 1.A_1 + 1.A_2).B_2 \end{aligned} \tag{7}$$

To derive equation (7), we start with equation (6), which is the conventional implementation of a Ternary Half-Adder:

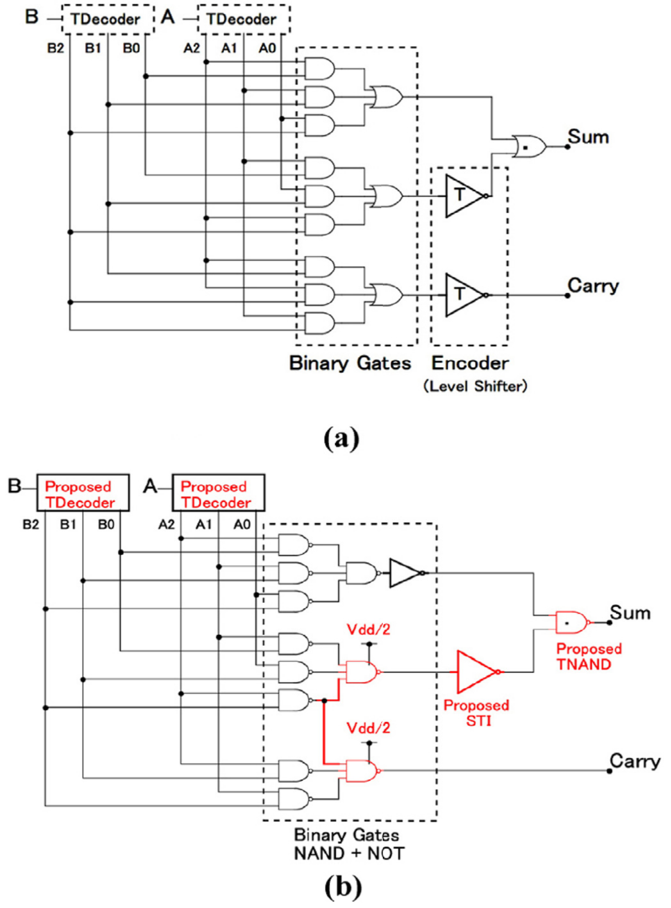


**Fig. 6.** Existing THA: (a) In Ref. [15] with 136 transistors, and (b) in Ref. [16] with 85 transistors.

$$Sum = 2.A_0B_2 + 2.A_1B_1 + 2.A_2B_0 + 1.A_0B_1 + 1.A_1B_0 + 1.A_2B_2$$
$$= B_0(1.A_1 + 2.A_2) + B_1(1.A_0 + 2.A_1) + B_2(2.A_0 + 1.A_2)$$
$$= B_0(0.A_0 + 1.A_1 + 2.A_2) + B_1(1.A_0 + 2.A_1 + 0.A_2)$$
$$+ B_2(2.A_0 + 0.A_1 + 1.A_2)$$
$$Carry = 1.A_1B_2 + 1.A_2B_1 + 1.A_2B_2$$
$$= B_0(0) + B_1(0.A_0 + 0.A_1 + 1.A_2) + B_2(0.A_0 + 1.A_1 + 1.A_2)$$

Where $A_k$ and $B_k$, $k \in \{0,1,2\}$, are the outputs of the Ternary Decoder from the inputs $A$ and $B$.

The existing THAs in Refs. [15,16] are shown in Fig. 6 with 136, and 85, respectively.

Fig. 6 (a) shows the THA of [15] contains TDecoder (16 transistors), binary AND, binary OR, ternary encoder, and ternary OR.

Fig. 6 (b) shows the THA of [16] contains proposed TDecoder (9 transistors), binary NAND, binary Inverter, proposed STI, and proposed TNAND using De Morgan's Law and dual power supply (Vdd and Vdd/2).

This section proposes THA using cascading proposed (3:1) TMUX with 90 (6∗15) transistors, as shown in Fig. 7.

The Existing THA design in Ref. [17] with 168 (6∗28) transistors is the same as Fig. 7 but with TMUX equals to 28 transistors;

The operation of the proposed THA in Fig. 7: Two ternary inputs $A$ and $B$ used as selection for the proposed TMUX.

When the selection $B$ is logic 0, the output Sum will be equal to the values of $A$ (0, 1, 2), and the output Carry will be equal to logic 0 for $A$ (0, 1, 2), respectively.

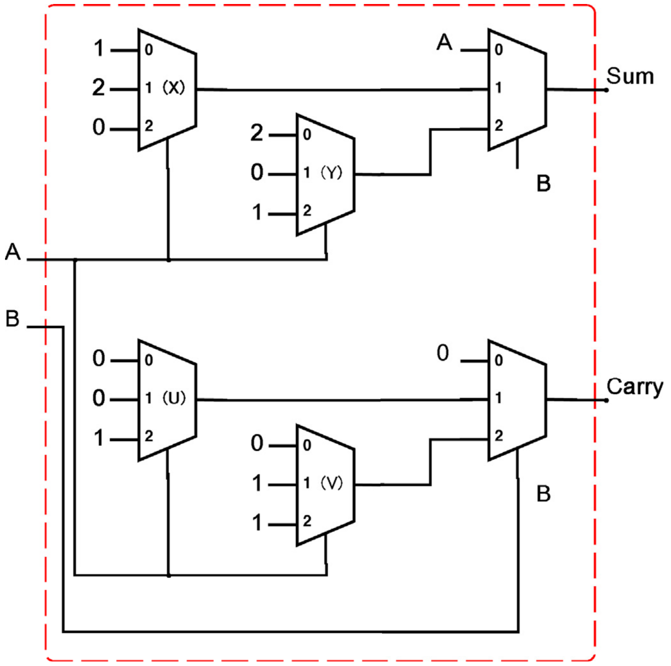


**Fig. 7.** Proposed THA with 90 transistors using proposed TMUX.

When the selection $B$ is logic 1, the output Sum will be equal to the output of (X) TMUX (1, 2, 0) for $A$ (0, 1, 2), respectively. The output Carry will be equal to the output of (U) TMUX (0, 0, 1) for $A$ (0, 1, 2), respectively.

Finally, when the selection $B$ is logic 2, the output Sum will be equal to the output of (Y) TMUX (2, 0, 1) for $A$ (0, 1, 2), respectively. The output Carry will be equal to the output of (V) TMUX (0, 1, 1) for $A$ (0, 1, 2), respectively.

The advantages of the proposed THA are:

1. The design does not use Ternary Decoder and basic logic gates such as "AND", "OR", and "NAND".
2. The design use the proposed Unary Operators and the proposed (3:1) TMUX.

All these advantages can reduce the transistors count and energy consumption.

## 5. Simulation results and comparisons

As mentioned in Section 1 that CNFET provides better energy efficiency compared to CMOS, FinFET, and other transistor technologies [11].

Therefore, the proposed (3:1) TMUX and THA are simulated and compared to CNFET-Based ternary circuits in Refs. [15–18].

Table 8 shows some essential parameters of the CNFET model used in all the circuits with brief descriptions.

The proposed THA are extensively simulated and tested using the HSPICE simulator with 32-nm channel length for power supply variation (from 0.8 V to 1 V), temperature variation (from 0 °C to 70 °C), frequency variation (from 0.5 GHz to 2 GHz), and manufacturing process variations (CNT diameter, CNT's count, Tox, and channel length) by using Monte Carlo analysis.

All input signals have a fall and rise time of 15 ps The average power consumption, maximum propagation delay, and maximum PDP are obtained for all circuits.

The performance of the proposed circuits will be compared to other designs for the PDP (energy consumption).

**Table 8**
Some of CNFET Model Parameters [19].

| | Description | Value |
|---|---|---|
| $L_{ch}$ | Physical channel length | 32 nm |
| $L_{geff}$ | The mean free path in the intrinsic CNT | 100 nm |
| $L_{ss}$ ($L_{dd}$) | The length of doped CNT source-side (drain-side) extension region | 10 nm |
| *Efi* | The Fermi level of the doped tube | 0.6 eV |
| $K_{gate}$ | The dielectric constant of high-k top gate dielectric material (planer gate) | 4 |
| $T_{ox}$ | The thickness of the high-k top gate dielectric material ($HfO_2$) | 1 nm |
| *Pitch* | The distance between two adjacent CNTs within the same device | 20 nm |
| *Tubes* | The number of tubes | 1 |

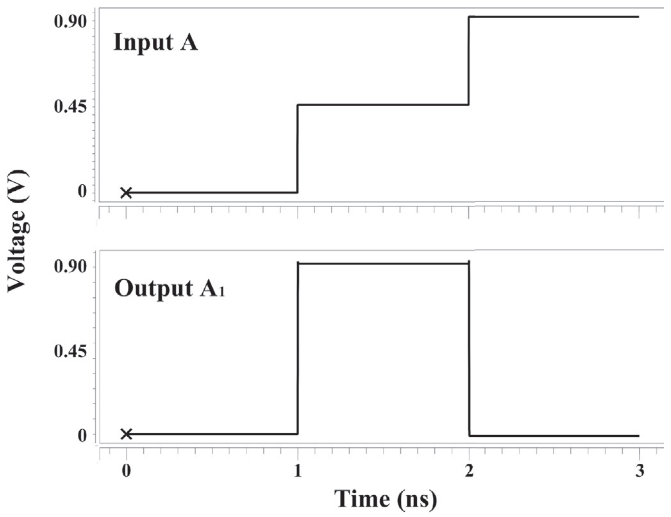


**Fig. 8.** Transient analysis of the proposed $A_1$.

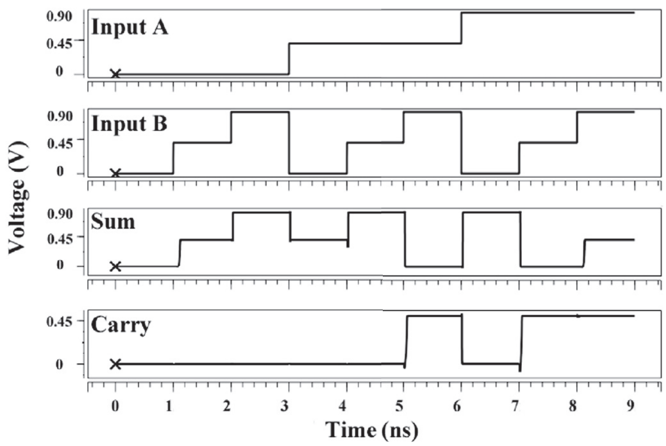


**Fig. 9.** Transient analysis of the proposed THA.

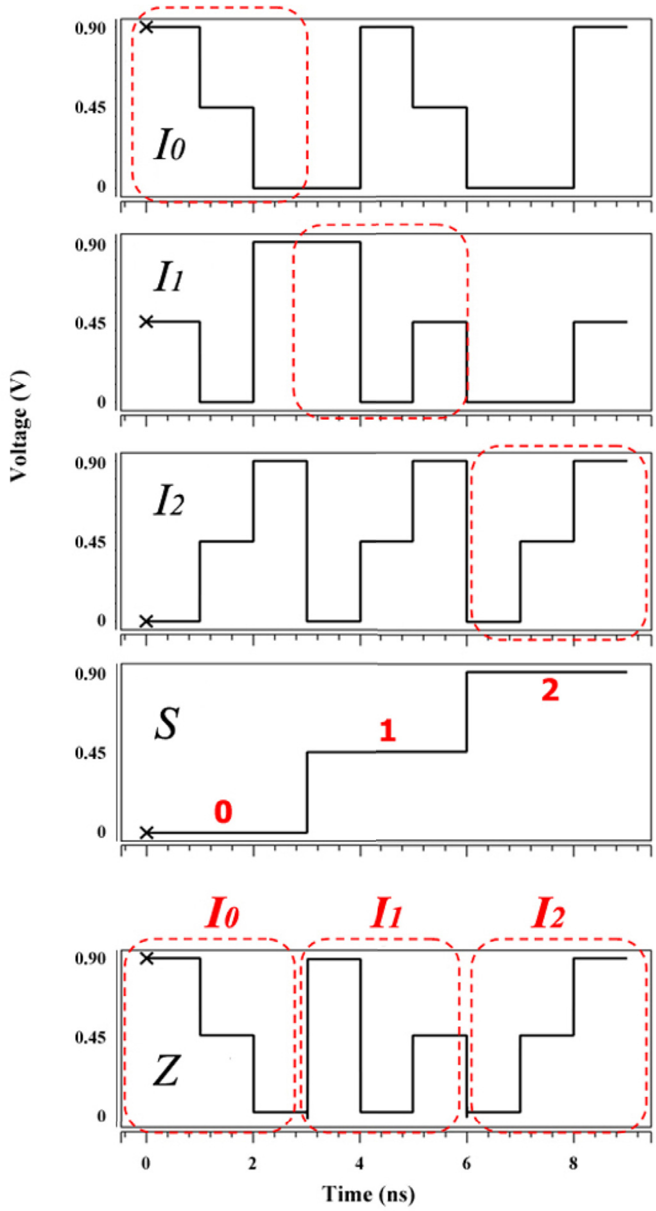


**Fig. 10.** Transient analysis of the proposed (3:1) TMUX (dotted rectangle corresponds to input selected according to S).

Fig. 8 and 9 illustrate the transient analysis of the proposed Unary Operator and THA.

### 5.1. Comparison of ternary multiplexers

The proposed TMUX is compared to the TMUX in Refs. [17,18]. The three circuits are simulated and tested using the HSPICE simulator with a frequency of 1 GHz, room temperature 27 °C, and a supply voltage 0.9 V (Vdd).

For a fair comparison, the three circuits are simulated using the same software, implementation techniques, CNFET model parameters, and the same values of ($I_0$, $I_1$, $I_2$, $S$) as follows:

$I_0 = (210021002)_3$, $I_1 = (102201001)_3$, $I_2 = (012012012)_3$ and $S = (000111222)_3$.

Fig. 10 illustrates the transient analysis of the proposed (3:1) TMUX. The dotted rectangle for each of the three inputs ($I_0$, $I_1$, $I_2$) is selected according to the ternary selection ($S$) to get the output ($Z$).

**Table 9**
Comparison of 3 TMUXs in terms of the transistors count at Vdd (0.9 V), temperature (27 °C), and frequency (1 GHz).

| | CNFETs | Power ($\mu$W) | Delay (ps) | | PDP (x10−20 J) | |
|---|---|---|---|---|---|---|
| | No. | AVG. | AVG. | Max. | AVG. | Max. |
| TMUX [17] | 28 | 67.3 | 2.35 | 14.3 | 15.8 | 96.3 |
| TMUX [18] | 18 | 60.1 | 1.76 | 9.64 | 10.57 | 57.9 |
| **Proposed TMUX** | **15** | **48.4** | **1.62** | **8.5** | **7.8** | **41.1** |

**Table 10**
Comparison of transistors count.

| | THA |
|---|---|
| [15] Using TDecoder and Basic Logic Gates | 136 |
| [16] Using De Morgan's Law | 85 |
| [17] Using Cascading TMUXs | 168 |
| **Proposed** Using Cascading TMUXs | **90** |

Table 9 shows the comparison between the three TMUXs in terms of the transistors count, average power consumption, (average & maximum) propagation delay, and (average & maximum) PDP.

This comparison of the proposed "decoder-less" TMUX demonstrates a notable reduction in transistors count around 46.43%, and 16.67% compared to TMUX in Refs. [17,18], respectively. Also, a notable reduction in PDP of around 57.32%, and 29.02% compared to Ref. [17], and [18], respectively.

### 5.2. Comparison of transistors count for THAs

Albeit not being the only factor, minimizing the transistors' count is a good metric to compare different circuit implementations.

Table 10 shows the comparison of transistors count for the THA of [15–17].

The proposed THA has a notable reduction in transistors count. Around 33.82%, −5.88%, and 46.43% compared to THA in Refs. [15–17], respectively.

### 5.3. Comparison of different THA circuits

#### 5.3.1. Voltage variation

The effect of power supply variation (from 0.8 V to 1 V) on the performance metrics of all proposed circuits is studied.

Fig. 11 shows the comparison to the existing THA in Refs. [15–17] in terms of the average power consumption as shown in Fig. 11(a), maximum propagation delay as shown in Fig. 11(b), and maximum PDP as shown in Fig. 11(c) for a fixed frequency of 1 GHz, temperature of 27 °C, and by varying the supply voltages (from 0.8 V to 1 V).

The comparison of the proposed THA demonstrates a notable reduction in PDP, as shown in Fig. 11(c). For Vdd = 0.8 V, around 99.33%, 95.11%, and 95.54% compared to Refs. [15–17], respectively. For Vdd = 0.9 V, around 98.45%, 94.39%, and 94.67% compared to Refs. [15–17], respectively. For Vdd = 1 V, around 96.69%, 85.71%, and 88.53% compared to Refs. [15–17], respectively.

#### 5.3.2. Temperature variation

Temperature noise is one of the most critical issues which negatively affect the performance of the circuit.

The effect of temperature variation (from 0 °C to 70 °C) on the performance metrics of all proposed circuits is studied.

Fig. 12 shows the comparison to the existing THA in Refs. [15–17] in terms of the average power consumption as shown in Fig. 12(a), maximum propagation delay as shown in Fig. 12(b), and maximum PDP as shown in Fig. 12(c) for a fixed frequency of 1 GHz, supply voltage of 0.9 V, and by varying the temperatures (from 0 °C to 70 °C).

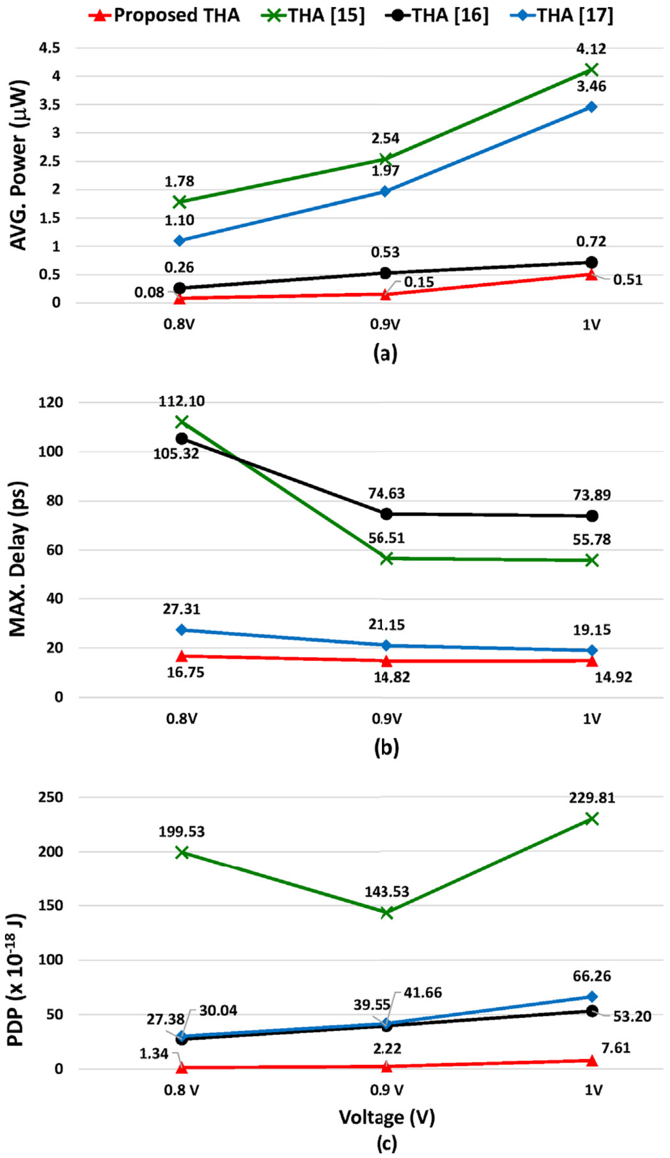


**Fig. 11.** Voltage variation of All THAs: (a) For Average Power, (b) for Maximum Delay, and (c) for PDP.

The comparison of the proposed THA demonstrates a notable reduction in PDP, as shown in Fig. 12(c). For Temperature = 0 °C, around 97.7%, 94.4%, and 91.96% compared to Refs. [15–17], respectively. For Temperature = 10 °C, around 98.2%, 94.15%, and 93.66% compared to Refs. [15–17], respectively. For Temperature = 27 °C, around 98.45%, 94.39%, and 94.67% compared to Refs. [15–17], respectively. For Temperature = 50 °C, around 98.26%, 94.27%, and 93.99% compared to Refs. [15–17], respectively. For Temperature = 70 °C, around 98.19%, 94%, and 93.45% compared to Refs. [15–17], respectively.

#### 5.3.3. Frequency variation

Electronic circuits behave very differently at high frequencies due to a change in the behavior of passive components (resistors, inductors, and capacitors) and parasitic effects on active components and PCB tracks.

The effect of frequency variation (from 0.5 GHz to 2 GHz) on the performance metrics of all proposed circuits is studied.

Fig. 13 shows the comparison to the existing THA in Refs. [15–17] in terms of the average power consumption as shown in Fig. 13(a), maximum propagation delay as shown in Fig. 13(b), and maximum PDP

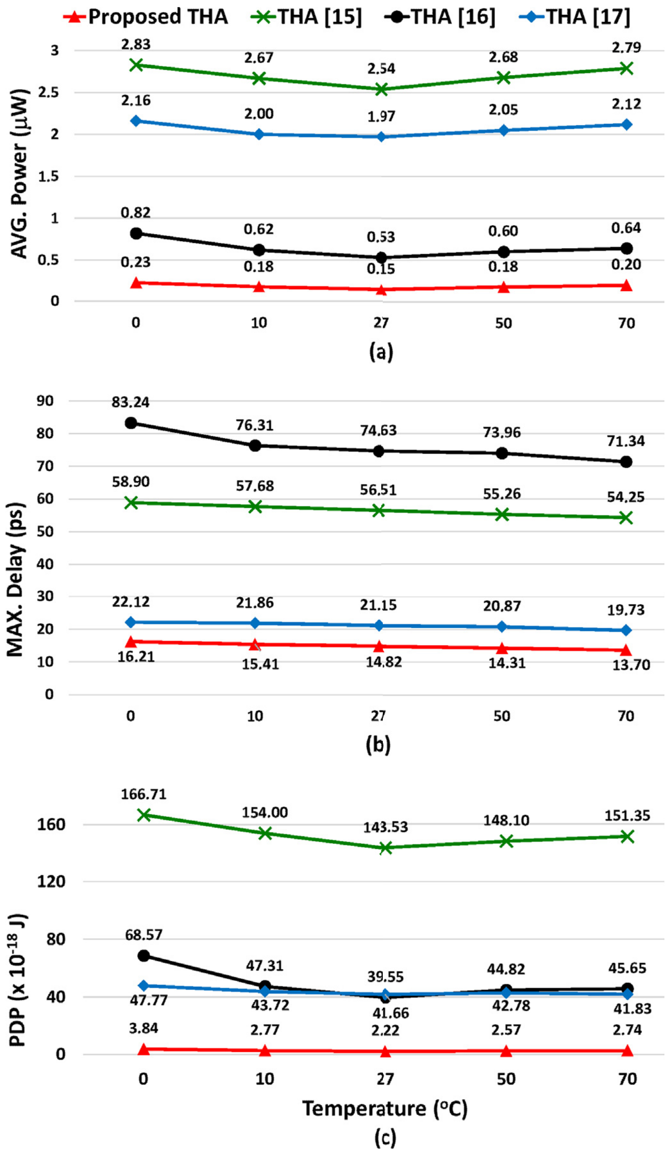


**Fig. 12.** Temperature variation of all THAs: (a) For average power, (b) for maximum delay, and (c) for PDP.

as shown in Fig. 13(c) for a fixed supply voltage of 0.9 V, temperature of 27 °C, and by varying the frequencies (from 0.5 GHz to 2 GHz).

The comparison of the proposed THA demonstrates a notable reduction in PDP, as shown in Fig. 13(c). For frequency = 0.5 GHz, around 98.8%, 95.23%, and 96.01% compared to Refs. [15–17], respectively. For frequency = 1 GHz, around 98.45%, 94.39%, and 94.67% compared to Refs. [15–17], respectively. For frequency = 2 GHz, around 97.76%, 91.94%, and 92.46% compared to Refs. [15–17], respectively.

### 5.3.4. Process variations

Process variations have a great impact on the performance and robustness of nanoscale devices and circuits. Hence, all THA circuits are tested in the presence of major process variations: TOX, CNT diameter, CNT's count, and channel length [23] (see Fig. 14).

TOX.

In the Stanford CNFET model, TOX is the oxide thickness of the Gate Dielectric $k_1$ material ($HfO_2$), as shown in 14. The variation in TOX will lead to leakage current. By decreasing TOX, the leakage current will increase, then the PDP will also increase and Vise Versa.

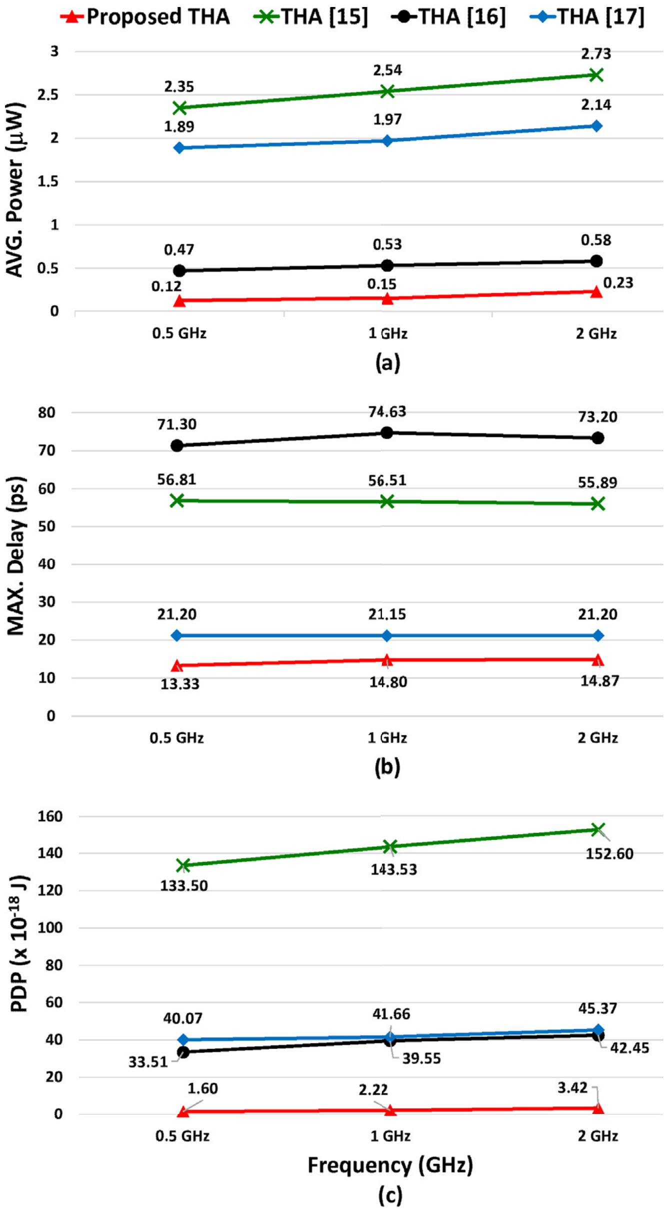


**Fig. 13.** Frequency variation of all THAs: (a) For average power, (b) for maximum delay, and (c) for PDP.

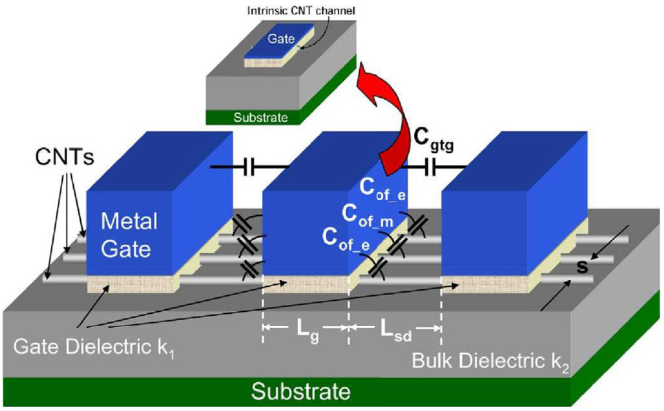


**Fig. 14.** Stanford CNFET model.

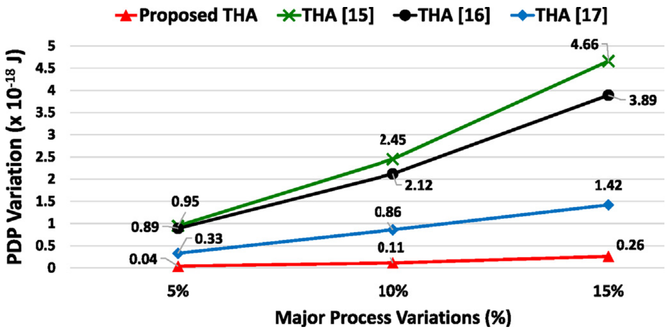


**Fig. 15.** Major Process Variations: TOX, CNT Diameter, CNT's Count, and Channel length.

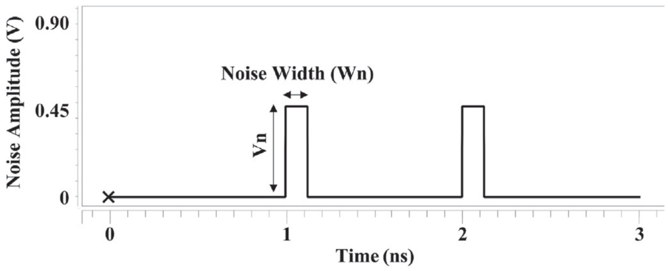


**Fig. 16.** Noise signal.

CNT Diameter.

The CNT diameter variation is one of the multiple problems of CNFET imperfections caused due to nonidealities in the CNT synthesis process, which negatively affects the performance of CNFET circuits because this variation will lead to variation in threshold voltage. This problem has more impact on MVL designs where transistors with different threshold voltages are applied.

CNT's Count.

Variation in the count of CNTs leads to a change in circuit parameters because it changes the output current of the transistor, which may cause a problem in the circuit functionality.

Channel Length.

Variation in channel length will lead to the variation of the channel between drain and source, which negatively affects the performance of CNFET circuits.

Therefore, this paper uses Monte Carlo analysis based on the Gaussian distributions with 5%, 10%, and 15% variations at the $\pm 3\ \sigma$ level with the number of simulation running is equal to 1000.

Monte Carlo analysis is based on statistical distributions. It realistically simulates mismatching and process variations. In each simulation run, it calculates every parameter randomly according to a statistical distribution model.

The energy variations of all THA circuits in the presence of the major process variations are shown in Fig. 15.

As shown in Fig. 15, The proposed THA has lower sensitivity to process variations and is more robust in comparison with the other designs because the graph of the proposed THA is under all the investigated circuits.

### 5.3.5. *Noise effect*

Digital circuits are inherently noise-tolerant, and they are only affected by noises with high amplitude and wide width.

The Noise Immunity Curve (NIC) is used to determine the impact of noisy inputs on all THAs circuits.

The noise signal, Fig. 16, is injected into inputs of THAs.

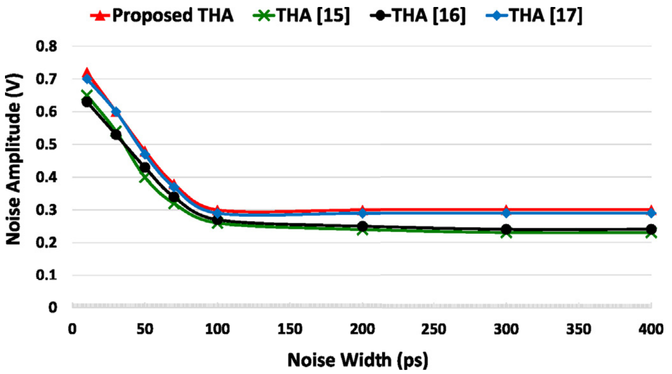


**Fig. 17.** Noise immunity curve (NIC).

As shown in Fig. 16, the noise signal has pulse width ($W_n$) and pulse amplitude ($V_n$).

Each point on the NIC curve is a pair of ($W_n$, $V_n$). Above that point, the circuit will produce an error on the output. The region above the NIC curve is an unsafe zone, whereas the region below the NIC curve is a safe zone against noise pulses.

Therefore, any circuit with higher NIC demonstrates a more noise-tolerant circuit [24].

As shown in Fig. 17, The proposed THA and the THA of [17] show higher noise immunity compared to our previous THA in Ref. [16] and the THA in Ref. [15] because their graphs are above of the others.

## 6. Conclusion

This paper proposed a Ternary Half Adder based on a proposed (3:1) Ternary Multiplexer using 32 nm channel CNFET, which aims to optimize the trade-off between performance and energy efficiency.

The comparison of the proposed approach to existing designs demonstrates notable performance gains for different simulation environments using HSPICE simulator with voltage variation, temperature variation, and frequency variation. Moreover, Monte Carlo analysis for major process variations (TOX, CNT Diameter, CNT's Count, and Channel length) was studied for all THAs models. The results confirmed that the proposed THA had higher robustness, among other designs. In addition, the noise immunity curve (NIC) showed that the proposed THA had a higher noise tolerance than other models.

Therefore, the proposed circuits can be implemented in low-power portable electronics and embedded systems to preserve battery consumption.

## Declaration of competing interest

None.

## Appendix A. Supplementary data

Supplementary data to this article can be found online at https://doi.org/10.1016/j.mejo.2019.104698.

## References

[1] S. Hosseini, S. Etezadi, A novel very low-complexity multi-valued logic comparator in nanoelectronics, Springer Circuits, Systems, and Signal Processing 2 (June 2019) 1–22, https://doi.org/10.1007/s00034-019-01158-2.

[2] S. Hurst, S. Etezadi, Multiple-valued logic its status and its future, IEEE Trans. Comput. 133 (1) (Dec. 1984) 1160–1179, https://doi.org/10.1109/TC.1984.1676392.

[3] M. Abdelaziz, T. Gulliver, Ternary trellis coded modulation, IEEE Access 7 (April 2019) 49027–49038, https://doi.org/10.1109/ACCESS.2019.2909707.

[4] Q. Yanq, B. Zhu, S. Wu, An architecture of cloud-assisted information dissemination in vehicular networks, IEEE Access 4 (May 2016) 2764–2770, https://doi.org/10.1109/ACCESS.2016.2572206.

[5] N. Saleh, A. Kassem, A. Haidar, Energy-efficient architecture for wireless sensor networks in healthcare applications, IEEE Access 6 (Jan. 2018) 6478–6486, https://doi.org/10.1109/ACCESS.2018.2789918.

[6] L. Sardinha, D. Silva, M. Vieira, L. Vieira, O. Neto, Tcam/cam-qca: (ternary) content addressable memory using quantum-dot cellular automata, Microelectron. J. 46 (7) (July 2015) 563–571, https://doi.org/10.1016/j.mejo.2015.03.020.

[7] N. Soliman, M. Fouda, A. Alhurbi, L. Said, A. Madian, A. Radwan, Ternary functions design using memristive threshold logic, IEEE Access 7 (April 2019) 48371–48381, https://doi.org/10.1109/ACCESS.2019.2909500.

[8] N. Soliman, M. Fouda, A. Radwan, Memristor-cntfet based ternary logic gates, Microelectron. J. 72 (Feb. 2018) 74–85, https://doi.org/10.1016/j.mejo.2017.12.008.

[9] A spectral algorithm for ternary function classification; vol. 1 of *1*, in: D. Miller, M. Soeken (Eds.), IEEE 48th Int. Symp. On Multiple-Valued Logic (ISMVL), IEEE, Linz, Austria, 2018.

[10] A. Basiri, S. Mahammad, High speed multiplexer design using tree based decomposition algorithm, Microelectron. J. 51 (May 2016) 99–111, https://doi.org/10.1016/j.mejo.2016.02.009.

[11] G. Hills, M. Bardon, G. Doornbos, D. Yakimets, P. Schuddinck, R. Baert, D. Jang, L. Mattii, S. Sherazi, D. Rodopoulos, R. Ritzenthaler, C.S. Lee, A. Thean, I. Radu, A. Spessot, P. Debacker, F. Catthoor, P. Raghavan, M. Shulaker, H.S. Philip Wong, S. Mitra, Understanding energy efficiency benefits of carbon nanotube field-effect transistors for digital vlsi, IEEE Trans. Nanotechnol. 17 (6) (Nov. 2018) 1259–1269, https://doi.org/10.1109/TNANO.2018.2871841.

[12] A Novel implementation of ternary decoder using CMOS DPL binary gates, in: R. Jaber, A. El-Hajj, L. Nimri, A. Haidar (Eds.), 2018 Int. Arab Conf. On Information Technology (ACIT), IEEE, Werdanye, Lebanon, 2018https://doi.org/10.1109/ACIT.2018.8672698.

[13] M. Jahangir, J. Mounika, Design and simulation of an innovative cmos ternary 3 to 1 multiplexer and the design of ternary half adder using ternary 3 to 1 multiplexer, Microelectron. J. 90 (Aug. 2019) 82–87, https://doi.org/10.1016/j.mejo.2019.05.007.

[14] D. Kundu, S. Guin, G. Jyothi, S. Sridevi (Eds.), High Speed FinFET Traff Comparator Based Function Generator. Chennai, India: 2018 International Conference on Computation of Power, Energy, Information and Communication (ICCPEIC), 2018.

[15] S. Lin, Y. Kim, F. Lombardi, Cntfet-based design of ternary logic gates and arithmetic circuits, IEEE Trans. Nanotechnol. 10 (March 2011) 217–225, https://doi.org/10.1109/TNANO.2009.2036845.

[16] R. Jaber, A. Kassem, A. El-Hajj, L. Nimri, A. Haidar, High-performance and energy-efficient cnfet-based designs for ternary logic circuits, IEEE Access 7 (July 2019) 93871–93886, https://doi.org/10.1109/ACCESS.2019.2928251.

[17] D. Das, A. Banerjee, V. Prasad (Eds.), Design of Ternary Logic Circuits Using CNTFET. Howrah, India: Int. Symp. On Devices, Circuits and Systems (ISDCS), March 2018.

[18] D. Das, A. Banerjee, V. Prasad, Design of ternary logic circuits using cntfet, IEEE Transactions on Circuits and Systems I: Regular Papers 64 (8) (Aug. 2017) 2146–2159.

[19] Stanford, , CA, , USA, . Stanford university cnfet model website. [online]. Accessed: July 1, 2019. .Available: http://nano.stanford.edu/model.php?id= 23

[20] J. Deng, H.S. Wong, A compact spice model for carbon-nanotube field-effect transistors including nonidealities and its application - part i: model of the intrinsic channel region, IEEE Trans. Electron Devices 54 (12) (Dec. 2007) 3186–3194, https://doi.org/10.1109/TED.2007.909030.

[21] J. Deng, H.S. Wong, A compact spice model for carbon-nanotube field-effect transistors including nonidealities and its application - part ii: full device model and circuit performance benchmarking, IEEE Trans. Electron Devices 54 (12) (Dec. 2007) 3195–3205, https://doi.org/10.1109/TED.2007.909043.

[22] D. Miller, M. Thornton, Multiple Valued Logic: Concepts and Representations. 12, Morgan & Claypool, San Rafael, CA, USA, 2008https://doi.org/10.1016/j.mejo.2019.01.013.

[23] S. Ebrahimi, M. Reshadinezhad, A. Bohlooli, A new design method for imperfection-immune cnfet-based circuit design, Microelectron. J. 85 (2019) 62–71, https://doi.org/10.1016/j.mejo.2019.01.013.

[24] G. Balamurugan, N. Shanbhag, The twin-transistor noise-tolerant dynamic circuit technique, IEEE J. Solid State Circuits 36 (2) (2001) 273–280, https://doi.org/10.1109/4.902768.
