# Supplementary material for: Multiple-Valued Logic Circuit Design and Data Transmission Intended for Embedded Systems
Source: arXiv:2211.04542 source file (2022-11-08)
Supplement: Supplementary file 2 [file TernaryDataTransmission.pdf]

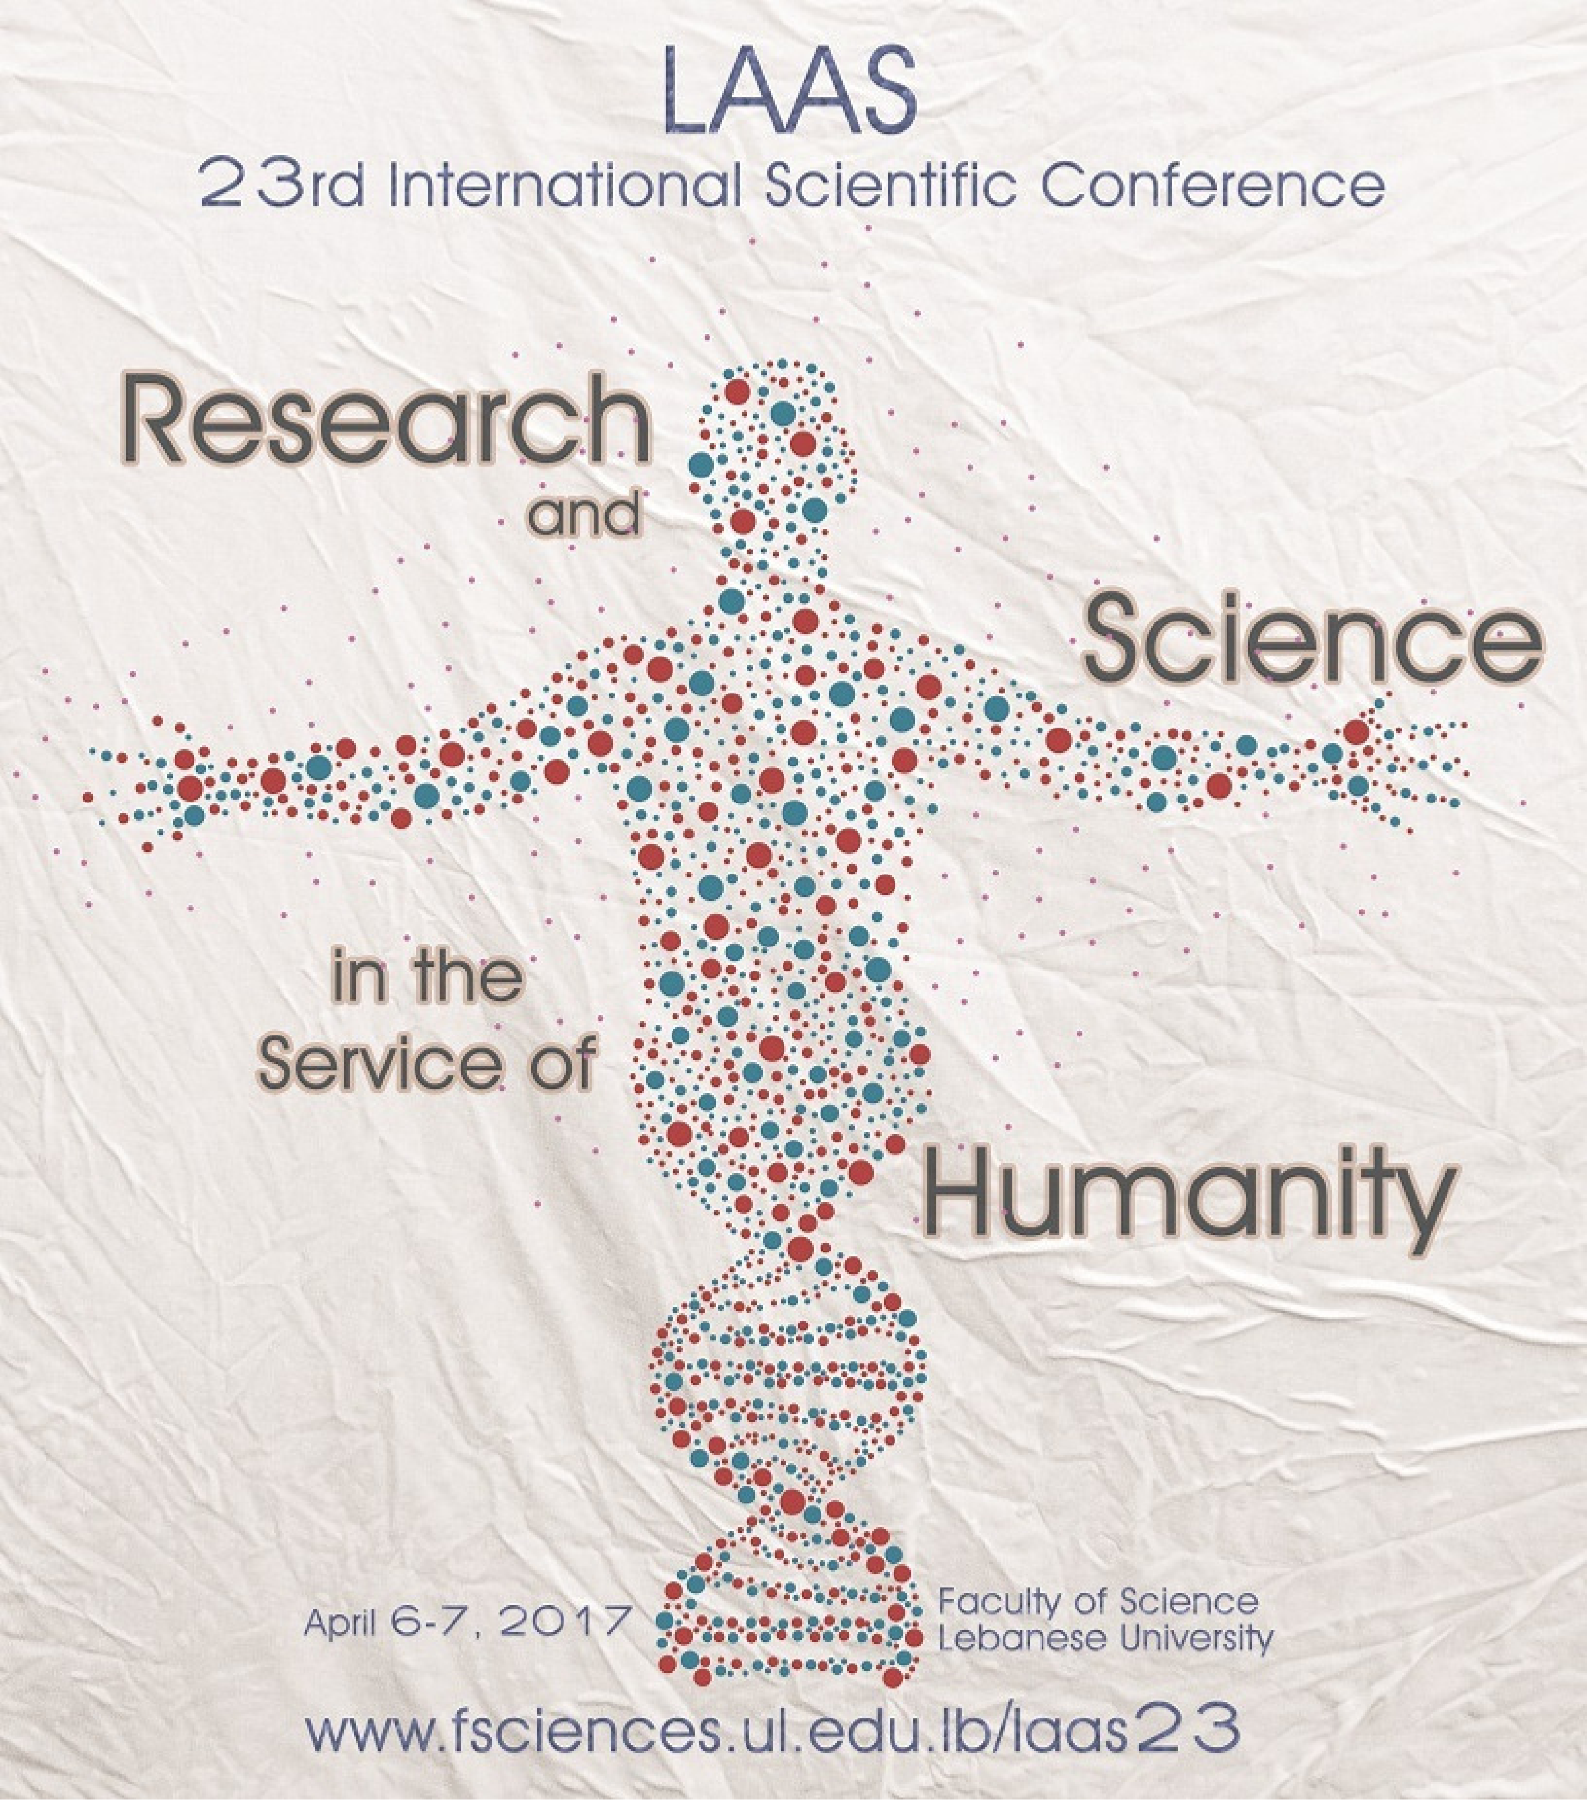
LAAS
23rd International Scientific Conference
Research
and
Science
in the
Service of
Humanity
April 6-7, 2017
Faculty of Science
Lebanese University
www.fsciences.ul.edu.lb/laas23

# Ternary Data Transmission Between Hosts


**Ramzi Ali JABER**
Depart.of Electrical & Computer Eng.
Beirut Arab University
Beirut, Lebanon
r.jaber@bau.edu.lb

**Lina Nimri**
Depart.of Business Computer
Lebanese University
Beirut, Lebanon
lnimri@ul.edu.lb

**Ali Massoud HAIDAR**
Depart.of Electrical & Computer Eng.
Beirut Arab University
Beirut, Lebanon
ari@bau.edu.lb



***Abstract*—there is limitation in Binary Data Transmission at Physical Layer in cable Connections between hosts (Computers, Hubs, Switches and Routers). In this paper we create a physical circuits to convert from Binary to Ternary and then from Ternary to Binary. After using these conversion the data is encrypted in transmission line and also the number of wires will reduce from 8 wires to 6 wires so we profit 25% from wires cost.**



***Keywords—Networking, Cabling, Physical Layer, Ternary, MVL, Multi-Valued Logic, Data Transmission.***


## I- INTRODUCTION

Intel Company & Many researchers believe that the binary logic is *already doomed* because of: 1-Moore's Law 1965 (Transistors will double every two years);2- we cannot shrink sizes of transistors indefinitely.

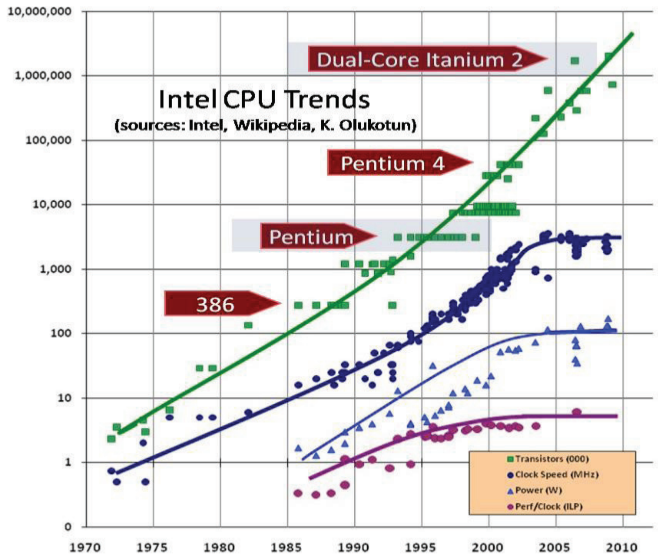


Fig.1, Limitation of Clock Speed

For that reason we want to rethink to use Multi-Valued Logic system instead of binary system if we can. We use in this paper Ternary Data transmission at physical layer between hubs, switches and routers.

## II- HOW IT WORKS

In Cat 5 cable there are four twisted pairs, two pairs for sending data and two pairs to receiving data.

### A) Sender Side:

Four wires will send the data at physical layer so we have 16 ($2^4$) combinations of binary digits : 0 for 0 volt, 1 for 5 volt.
We mapping them to Ternary trits. We use karnaugh map to design logic circuits.

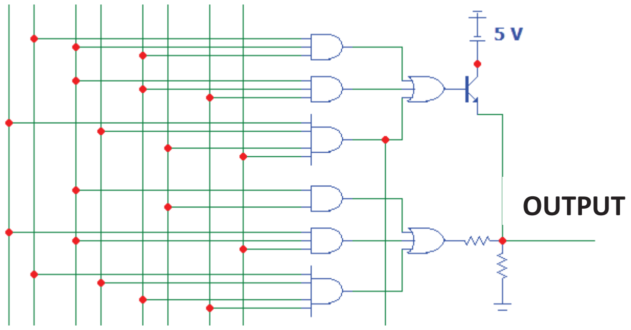


Fig. 2, portion from design model

We use 4 bits and their compliments entering logic AND Gates then OR Gates. At the above part there is transistor to pass only 5 volt state and open for 0 volt state.
At the lower part there is voltage divider to divide 5 volt into 2.5 volt. After this we will get ternary trits : **0** for 0 volt,**1** for 2.5 volt, **2** for 5 volt. So we get 3 wires instead of 4 wires.

**B) Receiver Side:**

Now at each wire will be one of three states (0 or 1 or 2) (0 volt or 2.5 volt or 5 volt).

To convert them again to binary, we must do it into two steps (ie. Two circuits).

**Step 1:**

We create a circuit to convert 3 ternary wires into 5 binary wires.

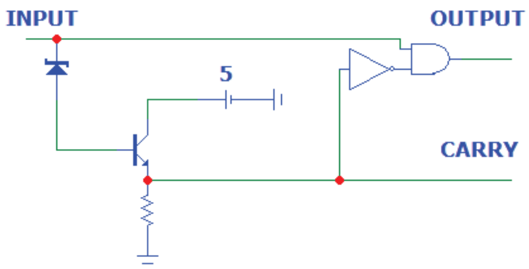


Fig. 3, Convert from ternary to binary

| Ternary Wire | Binary | |
|---|---|---|
| | Carry | Output |
| 0 (0 volt) | 0 | 0 |
| 1 (2.5 volt) | 0 | 1 (5 volt) |
| 2 (5 volt) | 1 | 0 |

TABLE 1, Conversion Table

We use 2.5 volt zener diode to filter the three voltages, when we have 0 or 2.5 volt as input the transistor will stay open so we get 0 or 5 volt at the output and if we have 5 volts as input then the transistor will operate and we get 0 for output and 5 volt for carry.

We have three wires as inputs, the first and the second wire have three states while the third wire has only two states 0 volt or 2.5 volt, so at final we will have 5 wires.

**Step 2:**

After we got 5 wires we will use five input karnaugh map to convert to 4 wires binary.

## III- Conclusion

In this paper a new concept has been proposed, Digital logic design based on binary system has been in use for long time. With phenomenal increase in circuit sizes, working with binary logic system is becoming increasingly complex. A Multiple-Valued Logic system reduces the significant amount of design effort, reduces the power consumption, increases the data transmission rate between devices and reduced the wires cost.

## REFERENCES


1. Y. Iijima and Y. Yuminaka, " Double-Rate Equalization Using Tomlinson-Harashima Precoding for Multi-Valued Data Transmission ", ISMVL 2016 -46 th IEEE International Symposium on Multiple-Valued Logic
2. Yasushi Yuminaka , Masaaki Okui, "Efficient Data Transmission Using Multiple-Valued Pulse-Position Modulation 2012 IEEE 42nd International Symposium on Multiple-Valued Logic
3. A. M. Haidar, R. Dernaika ,F. Shibani, "A Novel Ternary Quadrature Amplitude Modulation 2006 2nd IEEE International Conference on Information & Communication Technologies
4. A. M. Haidar, S. Ghabboura ; N. Ahdab, "A Novel Multi-Valued Logic QAM" 2006 2nd IEEE International Conference on Information & Communication Technologies.
