# Supplementary material for: Multiple-Valued Logic Circuit Design and Data Transmission Intended for Embedded Systems
Source: arXiv:2211.04542 source file (2022-11-08)
Supplement: Supplementary file 3 [file Ternary_Decoder.pdf]

# A Novel Implementation of Ternary Decoder Using CMOS DPL Binary Gates

**Publisher: IEEE**

**4 Author(s)** Ramzi Jaber ; Ahmad Elhajj ; Lina Nimri ; Ali Haidar **View All Authors**

1
Paper
Citation

44
Full
Text Views

**Abstract**

Document Sections

I. Introduction

II. Existing Ternary Decoder

III. Double Pass-Transistor Logic (DPL)

IV. Proposed Ternary Decoder

V. Simulation Results & Comparisons

**Abstract:**
This paper proposes a novel implementation of Ternary Decoder using CMOS DPL (Double Pass Logic) Binary logic gates, in digital CMOS technology. The physical design of the circuits is simulated and tested with Micro-Cap 10 SPICE simulator. The Proposed Ternary Decoder circuit can be used in VLSI design. The Proposed decoder circuit will be the basic circuit to create other Ternary Logic Circuits like Ternary Logic Gates, Ternary Memory, Adder, Multiplier, Multiplexer, and others. The simulation results demonstrate the merits of the approach in terms of reduced number of transistors by 25% compared to the existing ternary decoder.

**Published in:** 2018 International Arab Conference on Information Technology (ACIT)

**Date of Conference:** 28-30 Nov. 2018

**INSPEC Accession Number:** 18530437

**Date Added to IEEE *Xplore*:** 25 March 2019

**DOI:** 10.1109/ACIT.2018.8672698

# A Novel Implementation of Ternary Decoder Using CMOS DPL Binary Gates

Ramzi Jaber[a], Ahmad ElHajj[a], Lina Nimri[b], Ali Haidar [a]
[a]Depart.of Electrical & Computer Eng., Beirut Arab University
[b]Depart. of Business Computer, Lebanese University
Beirut, Lebanon
r.jaber@bau.edu.lb , a.elhajj@bau.edu.lb , lnimri@ul.edu.lb , ari@bau.edu.lb

***Abstract*—this paper proposes a novel implementation of Ternary Decoder using CMOS DPL (Double Pass Logic) Binary logic gates, in digital CMOS technology. The physical design of the circuits is simulated and tested with Micro-Cap 10 SPICE simulator. The Proposed Ternary Decoder circuit can be used in VLSI design.**

**The Proposed decoder circuit will be the basic circuit to create other Ternary Logic Circuits like Ternary Logic Gates, Ternary Memory, Adder, Multiplier, Multiplexer, and others.**

**The simulation results demonstrate the merits of the approach in terms of reduced number of transistors by 25% compared to the existing ternary decoder.**

***Keywords*— DPL, Ternary Circuit, Multi-Valued Logic, Ternary Decoder.**

## I. INTRODUCTION

Almost all the digital devices have been designed using two-valued logic till date. In binary logic, each wire can hold two states: 0 and 1. The performances of digital devices rely mostly on how quickly the states can be changed, which determines the speed of the devices. Multiple-valued logic (MVL) systems are multi-voltage levels. Therefore, MVL circuits have the following advantages over binary circuits [1- 6].

(i) In MVL circuits, as each wire can hold more information than binary logic, then the number of interconnections in the circuit is reduced and hence, the complexity of the chip is also reduced. (ii) Therefore MVL circuit provides lower power dissipation.

When using MVL in CMOS binary logic design, the performance will be better [7, 8].

Base 3 system (ternary logic) shows better results in the efficiency and the complexity as compared to higher bases [9]. Ternary logic digit (trits) has three values (0, 1, 2) corresponding to (0 volt, Vdd/2, Vdd).

For example, a decimal number 234 is 11101010 (8-bits) in binary whereas, in ternary equivalent is 22200 (5-trits). Thus the reduction in wires around 37.5% just for 8 bits, if more bits or wires the reduction will be more. That is why in the ternary circuit have lower interconnections, reducing the complexity, the power dissipation, and the propagation delay as compared to the binary circuit.

To the best of our knowledge, lot of research papers tries to design a ternary decoder using ternary logic gates like Standard Ternary Inverter (STI), Negative Ternary Inverter (NTI), Positive Ternary Inverter (PTI) and Ternary NOR logic gate [10,11,12] while the proposed Ternary Decoder only uses Binary AND logic gates, Binary NOR logic gate, MOSFET transistor , and resistor .

The Results from the proposed Ternary Decoder are less number of Transistors by 25% , therefore, gets a smaller chip area, reduced the energy consumptions, and decrease in the propagation delay.

The rest of the paper is organized as follows: Section II presents the existing Ternary Decoder, Section III presents the background of DPL, The proposed Ternary Decoder approach is presented in Section IV, Simulation results & Comparisons are discussed in Section V. Concluding remarks follow in Section VI.

## II. EXISTING TERNARY DECODER

The paper [12] presents three kinds of ternary inverters and ternary NOR to propose his Ternary Decoder. The first is Standard Ternary Inverter (STI), the second is Negative Ternary Inverter (NTI) and the third one is Positive Ternary Inverter (PTI). Table I shows their outputs.

Table I. Existing 3 ternary inverters truth table

| Ternary Input | STI | NTI | PTI |
|---|---|---|---|
| 0 | 2 | 2 | 2 |
| 1 | 1 | 0 | 2 |
| 2 | 0 | 0 | 0 |

The ternary decoder is one ternary input and three binary output circuit by generating unary functions for an input *x* is given by:

978-1-7281-0385-3/18/$31.00 ©2018 IEEE

$$X^k = \begin{cases} 2 \;\; if \; X = k \\ 0 \;\; if \; X \neq k \end{cases} \qquad (1)$$

Where k can take three logic values: logic 0, logic 1 and logic 2. The decoder outputs can take only two logic values i.e., logic 2 and logic 0, corresponding to logic 1 and logic 0 in binary logic.

The decoder consists of a PTI gate, two NTI gates, and a NOR gate, as shown in Fig. 1 and the truth table in Table II.

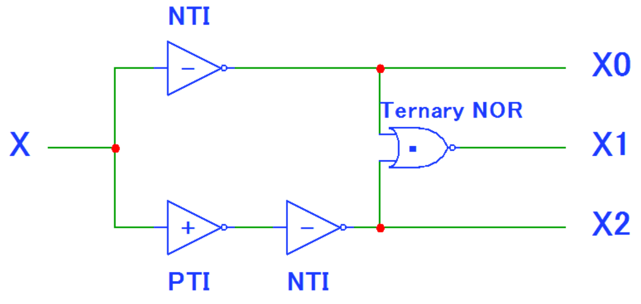


Fig. 1. Ternary Decoder [12]

Table II. The Ternary Decoder truth table

| Ternary Inputs | X0 | X1 | X2 |
|---|---|---|---|
| Logic **0** | 2 | 0 | 0 |
| Logic **1** | 0 | 2 | 0 |
| Logic **2** | 0 | 0 | 2 |

## III. Double Pass-transistor Logic (DPL)

As shown in Fig.2 [14], Double Pass-transistor Logic (DPL) is a modified version of Complementary Pass-transistor Logic (CPL) by adding PMOS transistors in parallel with the NMOS transistors to eliminate the problems of noise margin and speed degradation at reduced voltages supply associated in CPL circuits.

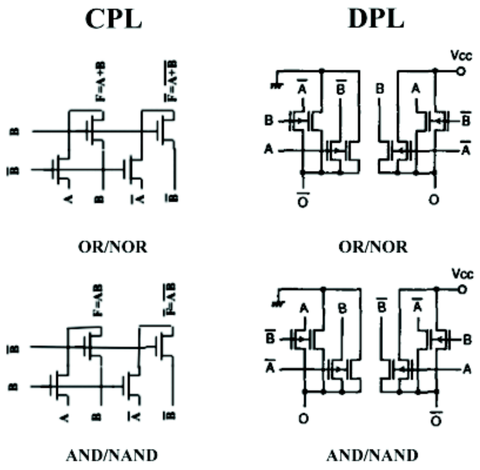


Fig.2. DPL Gates Design [14]

## IV. Proposed Ternary Decoder

As seen in section II the Ternary Decoder using Ternary logic gates is used to design Half Adder [12], Full Adder, Multiplier [12] and Multiplexer [10].

When design it with Binary Logic Gates will be faster and simpler [13].

Therefore a novel circuit is designed to implement Ternary decoder using CMOS DPL Binary logic gates with power supply VDD equals 1.8 volts which can reduce the power consumption and decrease the propagation delay.

Fig .3 represents the proposed Ternary Decoder.

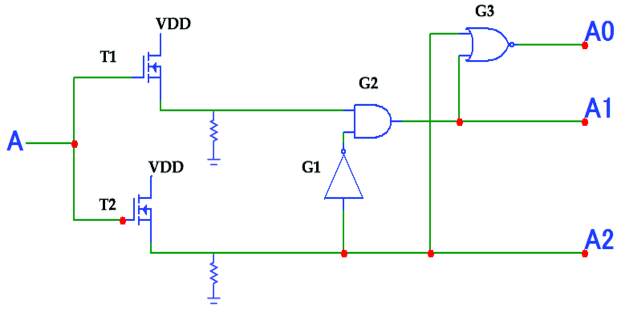


Fig. 3. The proposed Ternary Decoder

As shown in Fig.3. Two N-channels MOSFET, T1 with threshold voltage equals 0.7 volts and T2 with threshold voltage equals 1.4 volts, and three CMOS DPL Binary logic gates, G1 is “Inverter” logic gate, G2 is “AND” logic gate and G3 is “NOR” logic gate and two resistors 100 K Ω.

The explanation of Fig.3 is shown in Table III.

Table III. The proposed Ternary Decoder outputs

| **Ternary Input (A)** | **T1 Vth= 0.7v** | **T2 Vth= 1.4v** | **Binary Output** | | |
|---|---|---|---|---|---|
| | | | **A0** | **A1** | **A2** |
| Logic **0** (0v) | Open | Open | **1(1.8V)** | **0** | **0** |
| Logic **1** (0.9v) | Close | Open | **0** | **1(1.8V)** | 0 |
| Logic **2** (1.8v) | Close | Close | **0** | **0** | **1(1.8V)** |

The proposed ternary decoder can implement almost all ternary logic circuits

## V. Simulation Results & Comparisons

The proposed Ternary Decoder is analyzed using the Micro-cap 10 Spice simulator. The simulated circuits utilize an implementation of the AND and NOR DPL gates as shown in Fig.2 with a temperature 25°C, the power supply is set to 1.8 volts, the average propagation delay is 42.56 ps and the average power is 4.08 µw [16].

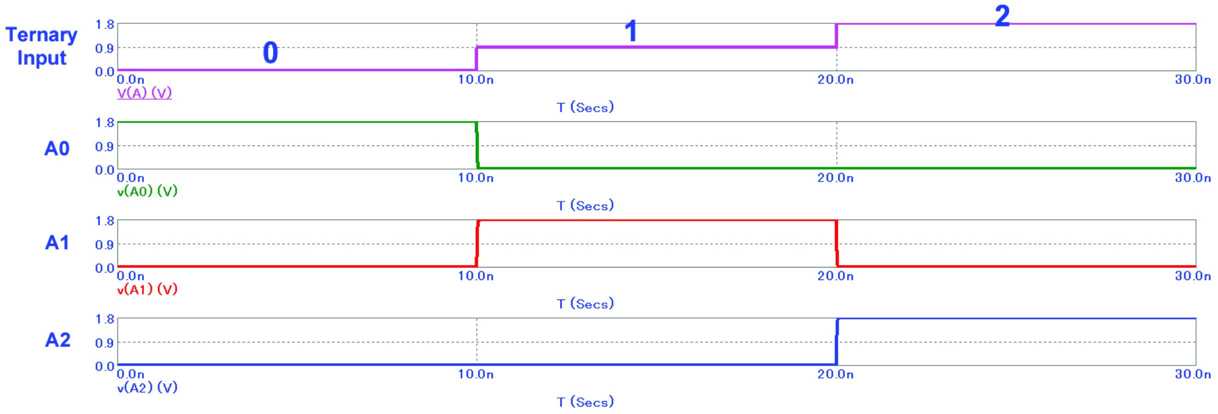


Fig.4. Transient Analysis of the Proposed Ternary Decoder

Fig. 4 shows the simulation transient analysis of the proposed circuit; The X-axis represents the time in 10 ns units and the Y-axis represents the voltage in 0.9 v units.

The Avg. power of the proposed Ternary Decoder is 13 µw and the Max. Propagation delay is 0.14 ns

The existing Ternary Decoder [12] has 16 transistors while the proposed one has 12 transistors; therefore, the improvement of the proposed ternary decoder is 25% less number of the transistor.

## VI. CONCLUSION

In this paper, a new Ternary Decoder is proposed. The proposed approach takes one Ternary Digit (trits) and produces three Binary bits using a DPL (Double Pass Logic) CMOS Binary gates to design other Ternary Logic circuits like Ternary Logic Gates, Ternary Memory, Adder, Multiplier, Multiplexer, and others.

The simulation results demonstrate the merits of the approach in terms of reduced number of transistors by 25% compared to the existing ternary decoder and using binary logic gates.

## REFERENCES

[1] M. H. Moaiyeri, K. Navi, O. Hashemipour, "Design and evaluation of CNTFET-based quaternary circuits," Circuits, Systems, and Signal Processing, vol. 31(5), pp. 16311652, Oct. 2012.

[2] Vaibhav Jane, Sanjay Tembhurne, "Design Low Power Quaternary Adder Using Multi-Value Logic," International Journal Of Advancement in Engineering Technology, Management and Applied Science (IJAETMAS), vol. 03(07), pp. 181-187, 2016.

[3] M.H Moaiyeri, A. Doostaregan, K. Navi, "Design of energy efficient and robust ternary circuits for nanotechnology," IET Circuits Devices Syst. vol. 5(4), pp. 285-296, 2011.

[4] Ramzi Jaber and Ali HAIDAR "Ternary Data Transmission between Hosts", the 23rd International Scientific Conference LAAS, 6 – 7 April 2017, Beirut, Lebanon.

[5] Oseily, H. and Haidar, A. M. "Hexadecimal to Binary Conversion Using Multi-Input Floating Gate Complementary Metal Oxide Semiconductors", the proceeding of International Conference on Applied Research in Computer Science and Engineering. ICAR 2015, 8 – 9 October 2015.

[6] Haidar, **A.**, N. El Ahdab, H. Shirahama, A. Alaeldine "Multiple-Valued Logic Neuron Clock Transformers", Proceeding of the ITC-CSCC´08 (The International Technical Conference on Circuit, Systems, Computers and Communications), Shimonoseki, Japan, July 2008.

[7] D. A. Rich, "A Survey of Multivalued Memories," IEEE Trans. Computer., vol. 35, pp. 99–106, Feb. 1986.

[8] Y. Yasuda, Y. Tokuda, S. Zaima, K. Pak, T. Nakamura, and A. Yoshida, "Realization of Quaternary Logic Circuits by n-channel MOS Devices," IEEE Journal of Solid-State Circuits, vol. 21, pp. 162–168, Feb 1986.

[9] Murotiya, S.L. and Gupta, A. (2014) 'Design of CNTFET-based 2-bit ternary ALU for nanoelectronics', *International Journal of Electronics*, Vol. 101, No. 9, pp.1244–1257

[10] Chetan Vudadhaa, M.B.Srinivasb, "Design Methodologies for Ternary Logic Circuits", 2018 IEEE 48th International Symposium on Multiple-Valued Logic, 16-18 May 2018, Linz, Austria.

[11] Debaprasad Das , Anirban Banerjee , Vikash Prasad, " Design of ternary logic circuits using CNTFET", 2018 International Symposium on Devices, Circuits and Systems (ISDCS), 29-31 March 2018, Howrah, India.

[12] S. Lin, Y. B. Kim, and F. Lombardi, "CNTFET-Based Design of Ternary Logic Gates and Arithmetic Circuits," IEEE Transactions on Nanotechnology, vol. 10, pp. 217–225, March 2011.

[13] E Danial, I Michel, "Implementation of Ternary Circuits with Binary Integrated Circuits", IEEE TRANSACTIONS ON COMPUTERS, VOL. C-26, No. 12, December 1977.

[14] M. Suzuki, N. Ohkubo, T. Shinbo, T. Yamanaka, A. Shimizu, K. Sasaki and Y. Nakagome, "A 1.5-ns 32-b CMOS ALU in Double Pass-Transistor Logic," IEEE Journal of Solid-State Circuits, vol. 28, no. 11, pp. 1145-1151, November 1993

[15] Tony R. Kuphaldt "Lessons In Electric Circuits" Volume IV – Digital 2007 https://www.allaboutcircuits.com/assets/pdf/digital.pdf.

[16] Saha Aloke, Pal Dipankar, and Chandra Mahesh. Benchmarking of DPL Based 8b×8b Novel Wave-Pipelined Multiplier. In: Int. J. of Electronics Letters (IJEL), Taylor & Francis. 2017; 5(1):115–128(doi: 10.1080/21681724.2016.1175031).
