# Supplementary material for: Multiple-Valued Logic Circuit Design and Data Transmission Intended for Embedded Systems
Source: arXiv:2211.04542 source file (2022-11-08)
Supplement: Supplementary file 4 [file Ternary_UnaryOperators.pdf]

# CNFET-Based Ternary Arithmetic Logic Unit Design Using a Combination of Novel Unary Operators and Ternary Multiplexers

Ramzi A. Jaber, Ahmad M. El-Hajj, Abdallah Kassem, Lina A. Nimri, Ali M. Haidar.

***Abstract*—This paper proposes new ternary arithmetic logic unit circuits that reduce the energy consumption in the context of low-power embedded circuits. The CNFET-based ternary half-adder and multiplier circuits utilize novel unary operator circuits, energy-efficient transistor arrangement, and apply two supply voltages (Vdd and Vdd/2) in order to reduce the transistors count and improve energy efficiency. Extensive simulations of the proposed designs, along with several benchmark designs using HSPICE, prove the merits of the proposed circuits in terms of reducing the power-delay-product, increasing the noise tolerance, and increasing the robustness to process variations (TOX, CNT Diameter, CNT's Count, and Channel length).**

***Index Terms*—Carbon Nano-Tube Field Effect Transistors (CNFET), Multi-Valued Logic (MVL), Ternary MUX, Unary Operators, VLSI.**

## I. Introduction

Binary circuits suffer from a significant drawback due to a large number of interconnections, which increase energy consumption. However, the Multi-Valued Logic (MVL) circuits reduce the interconnections, chip area, and energy consumption [1].

Also, the author of [2] has shown that ternary logic is the most efficient compared to other bases in terms of circuit complexity and cost.

Ternary logic systems can be implemented in two methodes: balanced (-1, 0, 1) equivalent to (-Vdd, 0, Vdd), and standard (0, 1, 2) equivalent to (0, Vdd/2, Vdd).

Recently, the researchers are interested in MVL over binary logic. MVL can be used in the algorithm [3], [4], wireless sensor networks for biomedical applications [5], cloud vehicular networks [6], communication systems [7], and circuit designs like Logic Gates, Memory, Memristor circuits [8]–[10].

Carbon Nano-Tube Field Effect Transistors (CNFET) provides the best trade-off in terms of performance and energy efficiency [19] compared to CMOS [11], and FinFet [12]. Thus, this paper utilizes CNFET transistors.

The authors of [13]–[15] designed their THAs and TMULs using the conventional design by utilizing the Ternary Decoder (TDecoder) and basic logic gates.

Manuscript received xxxx; revised xxxx.

R. A. Jaber, A. M. El-Hajj and A. M. Haidar are with the Department of Computer and Electrical Engineering, Beirut Arab University, Debbieh, Lebanon (e-mail: r.jaber@ieee.org; a.elhajj@bau.edu.lb; ari@bau.edu.lb).

A. Kassem is with the Department of Electrical and Computer Engineering, Notre Dame University, Louaize, Lebanon (e-mail: akassem@ndu.edu.lb) .

L. A. Nimri is with Department of Business Computer, Lebanese University, Beirut, Lebanon (e-mail: lnimri@ul.edu.lb) .

In [13], the authors presented a THA with 136 transistors, and a TMUL with 100 transistors using TDecoder with 16 transistors, AND, OR, Ternary NOR, and Ternary Encoder. While in [14], the authors designed a THA with 112 transistors, and a TMUL with 76 transistors using TDecoder with 10 transistors, NAND, Ternary NAND, and Standard Ternary Inverter (STI). Whereas in our previous work [15], we proposed a novel TDecoder with 9 transistors, a THA with 85 transistors, and a TMUL with 61 transistors using De Morgan's Law and two supply voltages (Vdd and Vdd/2).

The authors of [16], [17] designed their THAs and TMULs using cascading Multiplexers.
In [16], the authors proposed a "decoder-less" Ternary Multiplexer (TMUX) with 12 transistors and a ternary full-adder with 74 transistors using cascading TMUX and binary MUX. Whereas in [17], the authors represented a TMUX with 28 transistors, a THA with 168 transistors, and a TMUL with 112 transistors.

Finally, the authors of [18] proposed new unary operators circuits, a "decoder-less" TMUX with 18 transistors, a THA with 64 transistors, and a TMUL with 58 transistors.

### A. Contributions

The designs mentioned above suffer from many transistors count, high energy consumption, low robustness to process variations, and low noise tolerance, as summarize in Table I.

This paper proposes efficient circuit implementation of novel design unary operators combined with a "decoder-less" TMUX in [16] to design the THA with 39 CNFETs and the TMUL with 34 CNFETs.

Based on the literature review designs mentioned above, the contributions of this paper are as follow:

1) The proposed designs do not use a Ternary Decoder and basic logic gates that lead to high transistors count (compared to [13]–[15]).
2) The proposed designs use unary operators of ternary logic, which are small circuits, in designing any ternary circuit is to replace the basic logic gates and significantly reduce the number of used transistors, (more details can be found in Section III).
3) The proposed designs use two supply voltages (Vdd and Vdd/2), which are provided from the same power supply. In general, to obtain logical state 1 (Vdd/2) in the ternary circuit from one supply voltage Vdd, two Diode-connected transistors acting as resistors must be

TABLE I: Summary of literature review

| Ref. | Year | Techniques | Transistor count THA | Transistor count TMUL | Limitation |
|---|---|---|---|---|---|
| [13] | 2011 | - TDecoder (16 transistors)<br>- Basic logic gates | 136 | 100 | - High energy consumption<br>- Low robustness to process variations<br>- Low noise tolerance |
| [14] | 2017 | - TDecoder (10 transistors)<br>- Basic logic gates | 112 | 76 | - High energy consumption<br>- Low robustness to process variations<br>- Low noise tolerance |
| [15] | 2019 | - TDecoder (9 transistors)<br>- Basic logic gates<br>- De Morgan's Law<br>- Two supply voltages (Vdd and Vdd/2) | 85 | 61 | - Medium energy consumption<br>- Low robustness to process variations<br>- Low noise tolerance |
| [16] | 2017 | - Cascading TMUX (12T) and Binary MUX | 74 | | - Result of Full Adder is not accurate |
| [17] | 2018 | - Cascading TMUX (28T) | 168 | 112 | - High energy consumption<br>- Low robustness to process variations<br>- Low noise tolerance |
| [18] | 2017 | - Unary Operators<br>- TMUX (18T) | 64 | 58 | - Medium energy consumption<br>- Medium robustness to process variations<br>- Medium noise tolerance |

added. Using these two transistors is necessary to create a voltage divider to produce the ternary logical state 1 (Vdd/2), as shown in Fig. 1(b). The results show a significant increase in the static power dissipation due to the direct current from Vdd to the ground [20]. Therefore, one of the advantages of this paper is the use of Vdd/2 to eliminate these two transistors.

All these advantages can reduce the transistors count, decrease the energy consumption, increase the robustness to process variations, and increase the noise tolerance.

The proposed designs provide significant system performance gains compared to the designs in [13], [15], [18], as shown in the HSPICE-based simulation results, and the proposed designs get the lowest energy consumption (Power-Delay Product (PDP)). Also, the noise effect and Monte Carlo analysis for major process variations (TOX, CNT Diameter, CNT's Count, and Channel length) were studied. The results confirmed that the proposed TALUs had higher robustness and higher noise tolerance, among other designs.

The rest of the paper is organized as follows: Section II provides a background of CNFETs and Unary Operators, while Section III and Section IV describe the proposed novel Unary Operators and the proposed Ternary Arithmetic Logic Unit, respectively. Section V discusses the simulation results and comparisons, followed by concluding remarks in Section VI.

## II. Background

### A. CNFET Design

The CNFET transistors use an SWCNT (semiconducting single-walled CNT) as a channel for conduction, and the

TABLE II: The relationship between the chirality, diameter, and threshold voltage.

| Chirality | CNT diameter | **Threshold voltage** N-CNFET | **Threshold voltage** P-CNFET |
|---|---|---|---|
| (10,0) | 0.783nm | 0.559V | - 0.559V |
| (13,0) | 1.018nm | 0.428V | - 0.428V |
| (19,0) | 1.487nm | 0.289V | - 0.289V |

TABLE III: The State of CNFETs with D1=1.487 nm and D2=0.783 nm

| Type | Diameter | Voltage Gate 0V | Voltage Gate 0.45V | Voltage Gate 0.9V |
|---|---|---|---|---|
| P-CNFET | D2 | ON | OFF | OFF |
| | D1 | ON | ON | OFF |
| N-CNFET | D2 | OFF | OFF | ON |
| | D1 | OFF | ON | ON |

improvement of CNFET is 13 times better than the MOSFET device, for more details about the Stanford CNFET model used in this study found in [21]–[23].

The diameter of the CNFET is calculated by the following equation (1):

$$D_{\mathrm{cnt}} = \frac{\sqrt{3} \cdot a_0}{\pi} \sqrt{i^2 + j^2 + ij} \tag{1}$$

Where $a_0$ = 0.142 nm is the inter-atomic distance between each carbon atom and its neighbor, and the integer pair ($i$, $j$) represents the chirality vector, which is the angle of atom arrangement along the tube in an SWCNT.

TABLE IV: Truth table of the selected Unary Operators

| Ternary Input | PTI | NTI | STI | Cycle Operators | | | | |
|---|---|---|---|---|---|---|---|---|
| $A$ | $A_p$ | $A_n$ | $\bar{A}$ | $A^1$ | $A^2$ | $\bar{A}^2$ | $1 \cdot \bar{A}_n$ | $1 \cdot \bar{A}_p$ |
| Logic 0 (0V) | 2 | 2 | 2 | 1 | 2 | 0 | 0 | 0 |
| Logic 1 (0.45V) | 2 | 0 | 1 | 2 | 0 | 2 | 1 | 0 |
| Logic 2 (0.9V) | 0 | 0 | 0 | 0 | 1 | 1 | 1 | 1 |

The threshold voltage of the CNFET is calculated by the following equation (2):

$$V_{\text{th}} = \frac{E_g}{2 \cdot e} = \frac{\sqrt{3}}{3} \frac{d \cdot V\pi}{e \cdot Dcnt} \quad (2)$$

Where $d$ = 2.49 Å is the carbon to carbon atom distance, $V\pi$ = 3.033 eV is the carbon bond energy in the tight binding model, $e$ is the electron charge unit, and $Dcnt$ is the CNT diameter.

The relationship between the chirality, diameter, and threshold voltage are shown in Table II that used in the ternary logic design, which are calculated from the equations (1) and (2).

The operation of the CNFET transistor depends on the type and the diameter of CNFET, as described in Table III.

### B. *Unary Operators of Ternary Systems*

To the best of our knowledge, the literature about unary operators of MVL is limited. It was formally defined in [24] as the number of one-place, or unary, functions of a $p$-valued logic system, which is $p^p$.

For binary systems where $p$ = 2, there are only four unary functions, the identity "01", negation "10", and the two constant functions "00" and "11". Whereas, for ternary systems where $p$ = 3, there are twenty-seven ($3^3$) unary functions.

The selected eight unary functions are shown in Table IV and derived from the equation (3) to be used later for designing THA and TMUL in section IV.

The first three unary functions are three types of ternary inverters, the $A_p$ is PTI (positive ternary inverter), the $A_n$ is NTI (negative ternary inverter), and the $\bar{A}$ is STI (standard ternary inverter), which is the complement of A. The fourth and the fifth functions are the cycle operators, the $A^1$ is the successor of $A$ and the $A^2$ is the predecessor of $A$. The sixth is $\bar{A}^2$ the complement of $A^2$, and the last two unary functions are the two-inputs ternary AND Gate, $1 \cdot \bar{A}_n$ and $1 \cdot \bar{A}_p$.

$$\begin{aligned} A_p &= \begin{cases} 2, & if A \neq 2 \\ 0, & if A = 2 \end{cases} \\ A_n &= \begin{cases} 2, & if A = 0 \\ 0, & if A \neq 0 \end{cases} \\ \bar{A} &= 2 - A \\ A^1 &= (A+1)mod(3) \\ A^2 &= (A+2)mod(3) \\ \bar{A}^2 &= 2 - A^2 \\ 1 \cdot \bar{A}_n &= min\{1, \bar{A}_n\} \\ 1 \cdot \bar{A}_p &= min\{1, \bar{A}_p\} \end{aligned} \quad (3)$$

Where $A \in \{0, 1, 2\}$ is the ternary input.

## III. Proposed Unary Operators of Ternary Systems

The existing Unary Operators' designs in [13], and [18] are shown in Fig. 1.

Fig. 1 (a) shows three types of ternary inverters ($A_p$, $A_n$, $\bar{A}$) of [13].

Fig. 1 (b) shows the existing unary operators ($A^1$, $A^2$, $1 \cdot \bar{A}_n$, and $1 \cdot \bar{A}_p$) of [18].

This paper proposes novel designs for five unary operators in [18], as shown in Fig. 2.

Fig. 2 shows the transistor level design of the proposed Unary Operators. (a) $A^1$, (b) $A^2$, (c) $1 \cdot \bar{A}_n$, (d) $1 \cdot \bar{A}_p$, (e) $\bar{A}^2$.

The diameter, and threshold voltage (Vth) of the CNFETs used in Fig. 2 are shown in Table V.

The operations of the proposed unary operators are summarized in Table VI with the transistors count in TableVII.

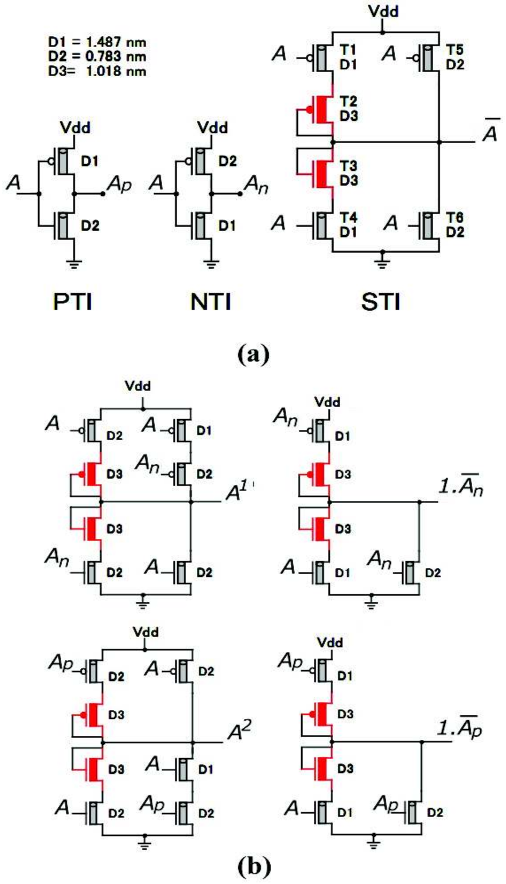


Fig. 1—Existing Unary Operators (a) in [13], $A_p$, $A_n$, and $\bar{A}$, (b) in [18], $A^1$, $A^2$, $1 \cdot \bar{A}_n$, and $1 \cdot \bar{A}_p$.

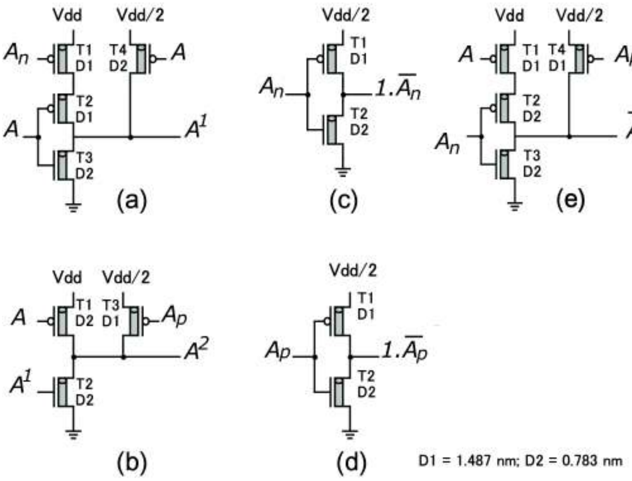


Fig. 2—The Transistor Level of the proposed Unary Operators: (a) $A^1$, (b) $A^2$, (c) $1 \cdot \bar{A}_n$, (d) $1 \cdot \bar{A}_p$, (e) $\bar{A}^2$.

TABLE V: The diameter, and threshold voltage of the CNTs used in the proposed Unary Operators.

| Type | Fig. 2 (a) | (b) | (c) | (d) | (e) | Diameter | Vth |
|---|---|---|---|---|---|---|---|
| N-CNFET | T3 | T2 | T2 | T2 | T2 | 0.783nm | 0.559V |
| P-CNFET | T4 | T1 | – | – | T1, T4 | 0.783nm | - 0.559V |
| P-CNFET | T1, T2 | T3 | T1 | T1 | T3 | 1.487nm | - 0.289V |

TABLE VI: Operation of the proposed unary operators

| Fig. 2 | $A$ | $A_n$ | $A_p$ | Transistors Turned ON | OFF | Output | |
|---|---|---|---|---|---|---|---|
| (a) | 0 | 2 | | T2,T4 | T1,T3 | 1 | |
| | 1 | 0 | | T1,T2 | T3,T4 | 2 | $\mathbf{A^1}$ |
| | 2 | 0 | | T1,T3 | T2,T4 | 0 | |
| (b) | 0 | | 2 | T1 | T2,T3 | 2 | |
| | 1 | | 2 | T2 | T1,T3 | 0 | $\mathbf{A^2}$ |
| | 2 | | 0 | T3 | T1,T2 | 1 | |
| (c) | 0 | 2 | | T2 | T1 | 0 | |
| | 1 | 0 | | T1 | T2 | 1 | $\mathbf{1 \cdot \overline{A_n}}$ |
| | 2 | 0 | | T1 | T2 | 1 | |
| (d) | 0 | | 2 | T2 | T1 | 0 | |
| | 1 | | 2 | T2 | T1 | 0 | $\mathbf{1 \cdot \overline{A_p}}$ |
| | 2 | | 0 | T1 | T2 | 1 | |
| (e) | 0 | 2 | 2 | T1,T3 | T2,T4 | 0 | |
| | 1 | 0 | 2 | T1,T2 | T3,T4 | 2 | $\mathbf{\overline{A^2}}$ |
| | 2 | 0 | 0 | T2,T4 | T1,T3 | 1 | |

TABLE VII: Transistors count comparison of unary operators

| | [18] | Proposed | Improvement |
|---|---|---|---|
| $\mathbf{A^1}$ | 7 | 4 | 42.86% |
| $\mathbf{A^2}$ | 7 | 3 | 57.14% |
| $\mathbf{\bar{A}^2}$ | 13* | 4 | 69.23% |
| $\mathbf{1 \cdot \bar{A}_n}$ | 5 | 2 | 60% |
| $\mathbf{1 \cdot \bar{A}_p}$ | 5 | 2 | 60% |

* $\bar{A}^2$ = $A^2$ (7 T) + $STI$ (6 T) = 13 Transistors

It is worth to mention the advantages of the proposed Unary Operators as follows:

1) They provide low energy consumption due to eliminating the two transistors that act as resistors in Fig. 1(b) (Transistor with diameter D3) by applying two supply voltages.
2) To get logic 1 (Vdd/2): one or two transistors must be active, as shown in Table VI, whereas in [18], four transistors in series must be active (T1, T2, T3, T4).
3) Reducing the transistors count, as shown in Table VII.

## IV. Proposed Ternary Arithmetic Logic Unit

This paper proposes a THA and a TMUL using the proposed unary operators combined with the TMUX in [16].

### A. Ternary Multiplexer

A Multiplexer (MUX) can select and forward several analog or digital input signals to a single output.

The (3:1) Ternary Multiplexer (TMUX) is introduced with the general model as represented in Fig.3, it has three inputs ($I_1$, $I_2$, $I_3$), one selection ($S$), and one output ($X$), which depends on ($S$) as described in (4).

$$X = \begin{cases} I_1, & if \quad S = 0 \\ I_2, & if \quad S = 1 \\ I_3, & if \quad S = 2 \end{cases} \tag{4}$$

In [16], the authors proposed a "decoder-less" (3:1) TMUX, as shown in Fig.4 with 12 transistors using NTI ($S_n$) and PTI ($S_p$).

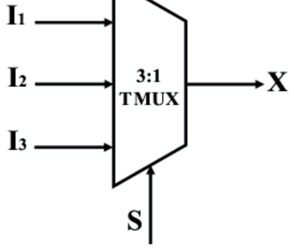


Fig. 3—The model of (3:1) TMUX

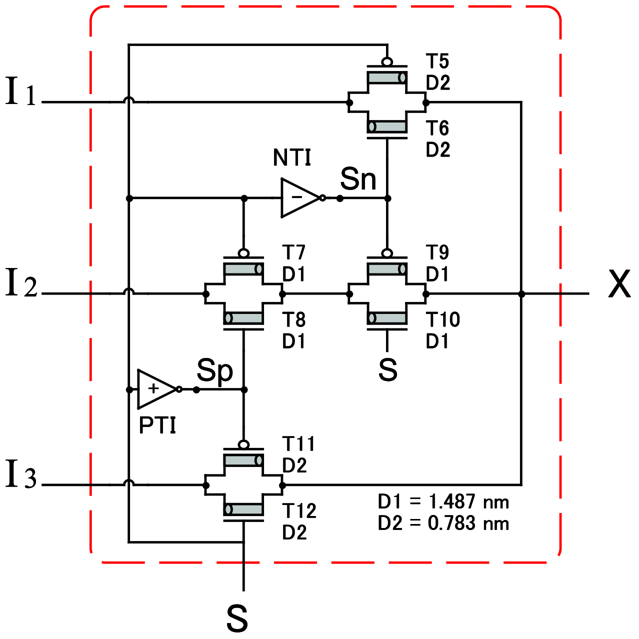


Fig. 4—Transistor Level of the (3:1) TMUX with 12 CNFETs in [16].

### B. Proposed Ternary Half Adder

The THA adds two ternary inputs ($A$ and $B$) and produces the Sum and the Carry, As shown in Table VIII.

Table VIII can derive the equations of the Sum and the Carry to lead two designs:

1) Conventional design in [13], [15] using equation (5).
2) Unary operators-based design in [18] and adopted in this paper using equation (6).

TABLE VIII: Truth table of THA

Sum

| A/B | $B_0$ (0) | $B_1$ (1) | $B_2$ (2) |
|---|---|---|---|
| $A_0$ (0) | 0 | 1 | 2 |
| $A_1$ (1) | 1 | 2 | 0 |
| $A_2$ (2) | 2 | 0 | 1 |
| | $\mathbf{A}$ | $\mathbf{A^1}$ | $\mathbf{A^2}$ |

Carry

| A/B | $B_0$ (0) | $B_1$ (1) | $B_2$ (2) |
|---|---|---|---|
| $A_0$ (0) | 0 | 0 | 0 |
| $A_1$ (1) | 0 | 0 | 1 |
| $A_2$ (2) | 0 | 1 | 1 |
| | $\mathbf{0}$ | $\mathbf{1 \cdot \overline{A_p}}$ | $\mathbf{1 \cdot \overline{A_n}}$ |

$$\begin{aligned} Sum &= 2 \bullet (A_0B_2 + A_1B_1 + A_2B_0) \\ &\quad +1 \bullet (A_0B_1 + A_1B_0 + A_2B_2) \\ Carry &= 1 \bullet (A_1B_2 + A_2B_1 + A_2B_2) \end{aligned} \tag{5}$$

$$\begin{aligned} Sum &= A.B_0 + A^1.B_1 + A^2.B_2 \\ Carry &= 0.B_0 + (1 \cdot \bar{A_p}).B_1 + (1 \cdot \bar{A_n}).B_2 \end{aligned} \tag{6}$$

Where $A_k$ and $B_k$, $k \in \{0,1,2\}$, are the outputs of the Ternary Decoder from the inputs $A$ and $B$.

The existing THA in [13], [15], and [18] are shown in Fig. 5 with 136, 85, and 64 transistors, respectively.
Fig. 5 (a) shows the THA of [13] that contains TDecoder (16 transistors), binary AND, binary OR, ternary encoder, and ternary OR.

Fig. 5 (b) shows the THA of our previous work in [15] that contains proposed TDecoder (9 transistors), binary NAND, binary Inverter, proposed STI and proposed TNAND using De Morgan's Law and two supply voltages (Vdd and Vdd/2).

Fig. 5 (c) shows the THA of [18] that contains (3:1) TMUX (18 transistors) and Unary Operators.

This paper proposes THA using proposed Unary Operators and 3:1 TMUX in [16], as shown in Fig. 6.

Table IX shows total transistors' count of the proposed THA, which is equal to 39 transistors, and its operation is described in the following paragraphs where Two $A$ and $B$ are the ternary inputs.

The input $A$ fed to $NTI$, $PTI$, and the proposed Unary Operators and produce outputs as ($A^1$, $A^2$, $1 \cdot \bar{A_p}$, $1 \cdot \bar{A_n}$ ).

The outputs ($A^1$, $A^2$) and the input $A$ are fed to the first (3:1) TMUX to get the Sum. The outputs ($1 \cdot \bar{A_p}$, $1 \cdot \bar{A_n}$) are fed to the second (3:1) TMUX to get the Carry.

The input $B$ is the selection for both TMUX.

TABLE IX: Total transistors count of the proposed THA

| | No. of Devices | No. of Transistors | Subtotal |
|---|---|---|---|
| TMUX in [16] | 2 | 12 | 24 |
| NTI ($A_n$) | 1 | 2 | 2 |
| PTI ($A_p$) | 1 | 2 | 2 |
| Proposed $A^1$ | 1 | 4 | 4 |
| Proposed $A^2$ | 1 | 3 | 3 |
| Proposed $1 \cdot \bar{A_p}$ | 1 | 2 | 2 |
| Proposed $1 \cdot \bar{A_n}$ | 1 | 2 | 2 |
| Total | | | 39 |

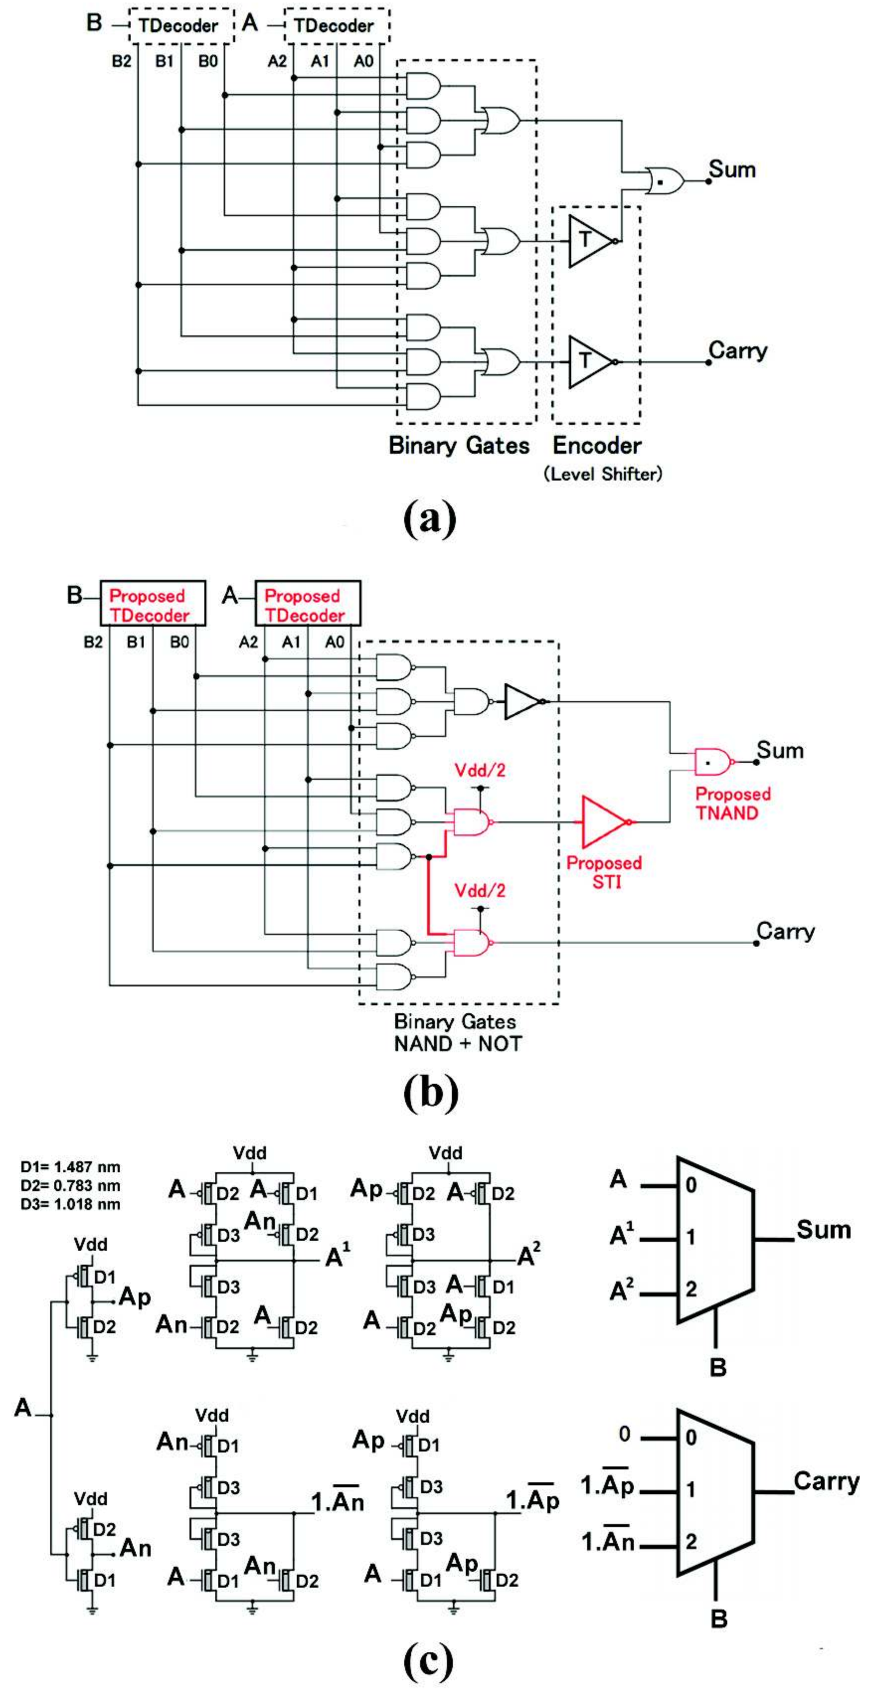


Fig. 5—Existing THA: (a) in [13] with 136 transistors, (b) in [15] with 85 transistors, and (c) in [18] with 64 transistors.

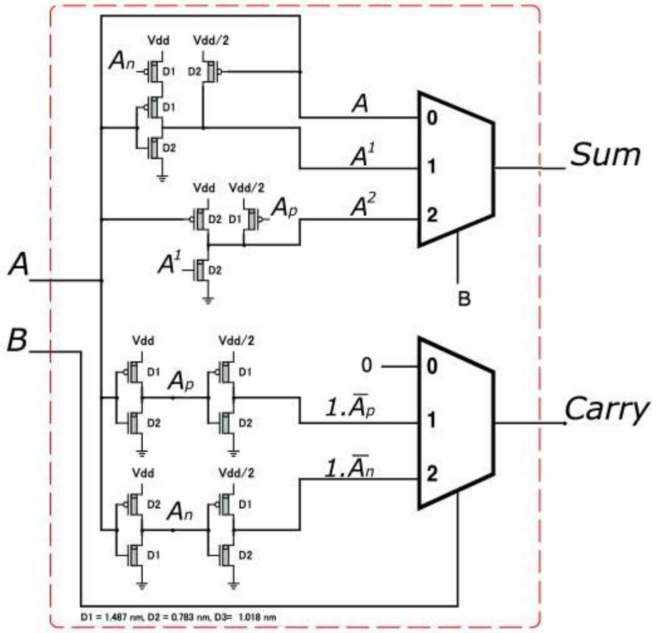


Fig. 6—Proposed THA with 39 transistors using proposed Unary Operators and TMUX in [16].

### *C. Proposed Ternary Multiplier*

The TMUL multiplies two ternary inputs ($A$ and $B$) and produces the Product and the Carry, As shown in Table X.

Table X can derive the equations of the Product and the Carry to lead two designs:

1) Conventional design in [13], [15] using equation (7)
2) Unary operators-based design in [18] and adopted in this paper using equation (8).

TABLE X: Truth table of TMUL

Product

| A/B | $B_0$ (0) | $B_1$ (1) | | $B_2$ (2) | |
|---|---|---|---|---|---|
| $A_0$ (0) | 0 | 0 | **A** | 0 | $\overline{\mathbf{A^2}}$ |
| $A_1$ (1) | 0 | 1 | | 2 | |
| $A_2$ (2) | 0 | 2 | | 1 | |

Carry

| A/B | $B_0$ (0) | $B_1$ (1) | $B_2$ (2) | |
|---|---|---|---|---|
| $A_0$ (0) | 0 | 0 | 0 | $\mathbf{1 \cdot \overline{A_p}}$ |
| $A_1$ (1) | 0 | 0 | 0 | |
| $A_2$ (2) | 0 | 0 | 1 | |

$$\begin{aligned} Product &= 2 \bullet (A_1B_2 + A_2B_1) \\ &+1 \bullet (A_1B_1 + A_2B_2) \\ Carry &= 1 \bullet A_2B_2 \end{aligned} \tag{7}$$

$$\begin{aligned} Product &= 0 \cdot B_0 + A \cdot B_1 A + \bar{A}^2 B_2 \\ Carry &= 0 \cdot B_0 + 0 \cdot B_1 + (1 \cdot \bar{A}_p) B_2 \end{aligned} \tag{8}$$

Where $A_k$ and $B_k$, $k \in \{0,1,2\}$, are the outputs of the Ternary Decoder from the inputs $A$ and $B$.

The existing TMUL in [13], [15], and [18] are shown in Fig. 7 with 100, 61, and 58 transistors, respectively.
Fig. 7 (a) shows the TMUL of [13] that contains TDecoder (16 transistors), binary AND, binary OR, ternary encoder, and ternary OR.

Fig. 7 (b) shows the TMUL of our previous work in [15] that contains proposed TDecoder (9 transistors), binary NAND, binary Inverter, proposed STI and proposed TNAND using De Morgan's Law and two supply voltages (Vdd and Vdd/2) from the same power supply.

Fig. 7 (c) shows the TMUL of [18] that contains (3:1) TMUX (18 transistors) and Unary Operators.

This paper proposes TMUL using proposed Unary Operators and 3:1 TMUX in [16], as shown in Fig. 8.

Table XI shows total transistors count of the proposed TMUL, which is equal to 34 transistors, and its operation is described in the following paragraphs where $A$ and $B$ are the ternary inputs.

The input $A$ fed to $NTI$, $PTI$, and the proposed Unary Operators and produce outputs as ($\bar{A}^2$, $1 \cdot \bar{A}_p$). The output ($\bar{A}^2$) with the input $A$ and logic 0 fed to the first proposed (3:1) TMUX to get the Product. The output ($1 \cdot \bar{A}_p$) with two logic 0s fed to the second proposed (3:1) TMUX to get the Carry.

Whereas, the input $B$ is the selection input for both TMUX.

TABLE XI: Total transistors count of the proposed TMUL

| | No. of Devices | No. of Transistors | Subtotal |
|---|---|---|---|
| TMUX | 2 | 12 | 24 |
| NTI ($A_n$) | 1 | 2 | 2 |
| PTI ($A_p$) | 1 | 2 | 2 |
| Proposed $\bar{A}^2$ | 1 | 4 | 4 |
| Proposed $1 \cdot \bar{A}_p$ | 1 | 2 | 2 |
| Total | | | 34 |

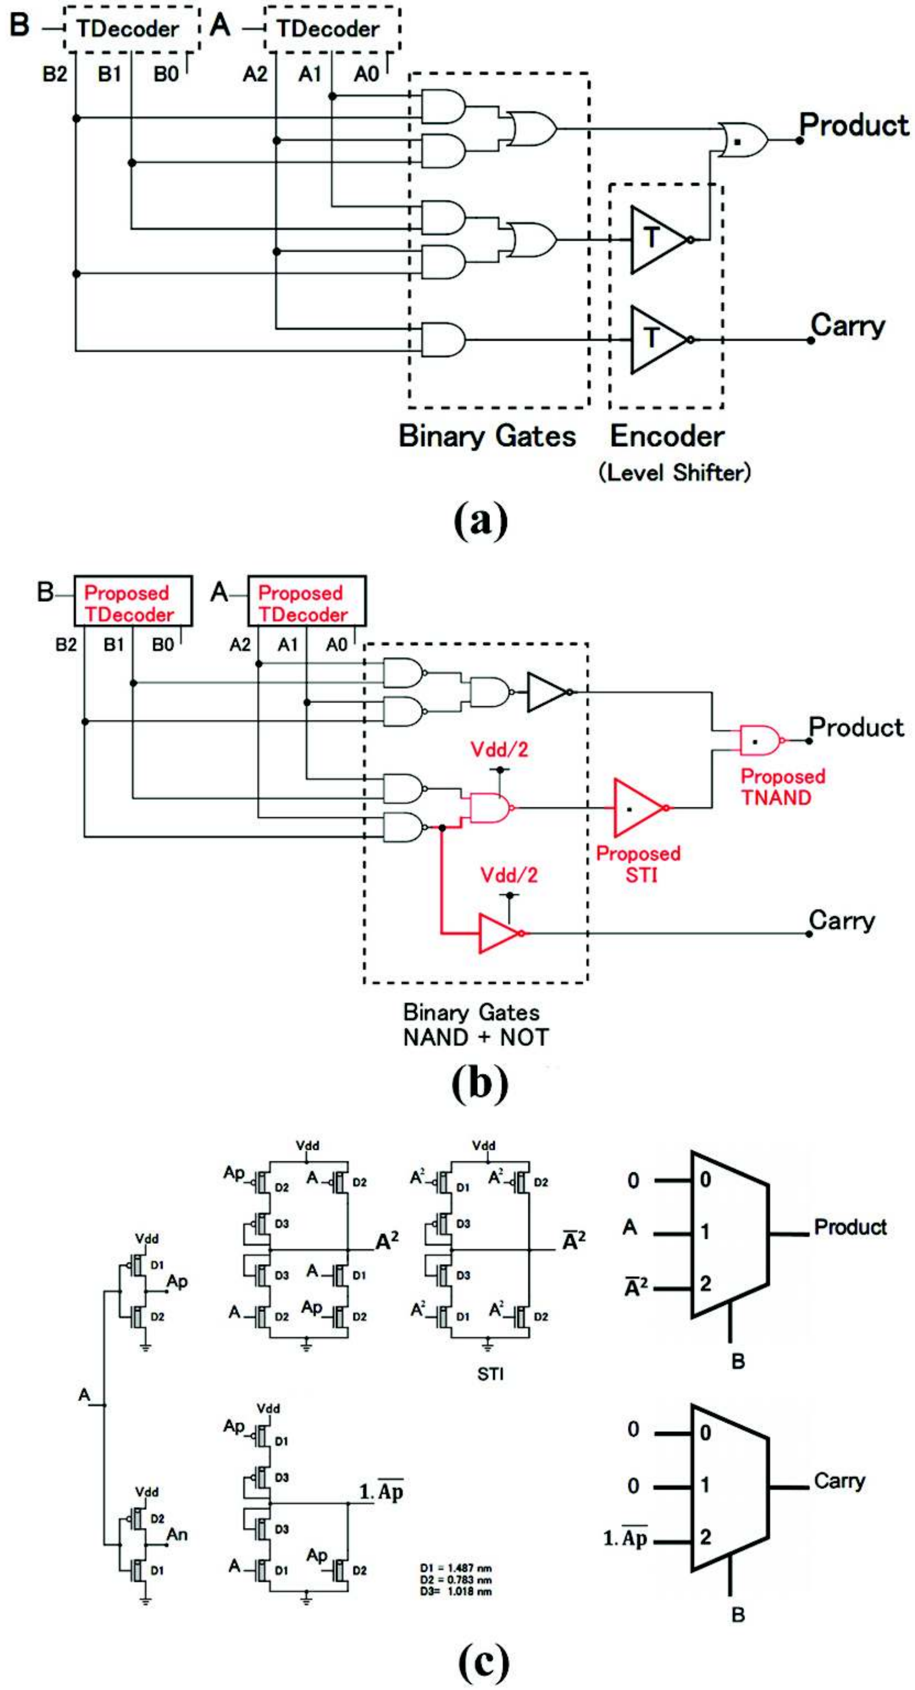


Fig. 7—Existing TMUL: (a) in [13] with 100 transistors, (b) in [15] with 61 transistors, and (c) in [18] with 58 transistors.

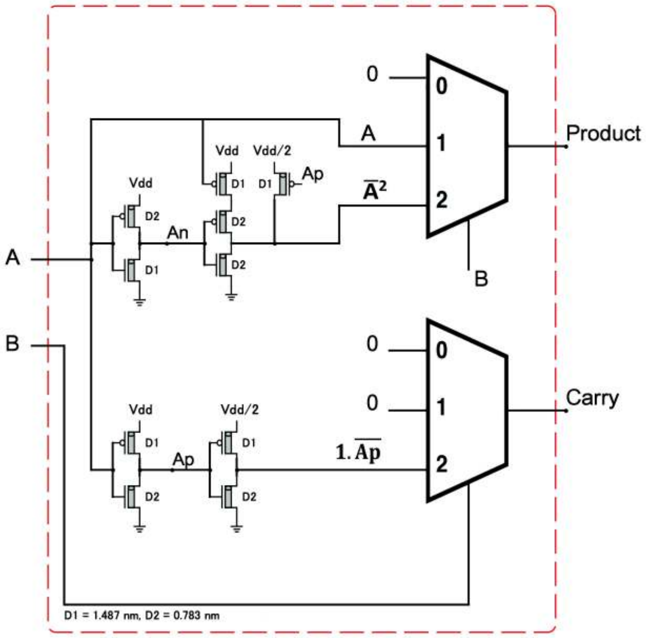


Fig. 8—Proposed TMUL with 34 transistors using proposed Unary Operators and TMUX in [16].

## V. Simulation Results and Comparisons

As mentioned in Section I, compared to CMOS, FinFET, and other transistor technologies, CNFET provides better energy efficiency [19].

Therefore, the proposed five Unary Operators, the THA, and the TMUL are simulated and compared to 32-nm CNFET-Based ternary circuits in [13], [15], [18].

The proposed circuits are extensively simulated and tested using the HSPICE simulator for power supply variation (from 0.8 V to 1 V), temperature variation (from 0°C to 70°C ), frequency variation (from 0.5 GHz to 2 GHz), Noise Immunity, and manufacturing process variations (CNT diameter, CNT's count, Tox, and channel length) by using Monte Carlo analysis.

Table XII shows some CNFET model parameters used in all circuits.

All input signals have a fall and rise time of 15 ps. The performance of the proposed designed will be compared to other designs for PDP.

TABLE XII: Some of the CNFET Model Parameters [21]

| | Description | Value |
|---|---|---|
| $L_{ch}$ | Physical channel length | 32 nm |
| $L_{ss}$ ($L_{dd}$) | The length of doped CNT source-side (drain-side) extension region | 10 nm |
| $Efi$ | The Fermi level of the doped tube | 0.6 eV |
| $T_{ox}$ | The thickness of the high-k top gate dielectric material ($HfO_2$) | 1 nm |
| $Tubes$ | The number of tubes | 1 |

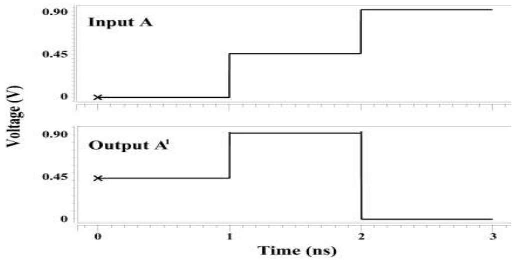


Fig. 9—Transient analysis of the proposed $A^1$.

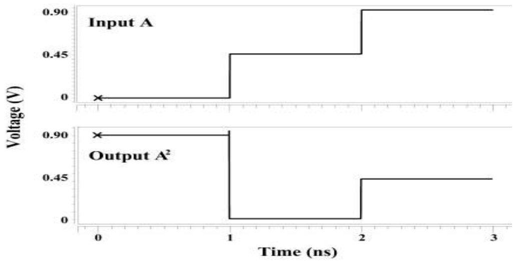


Fig. 10—Transient analysis of the proposed $A^2$.

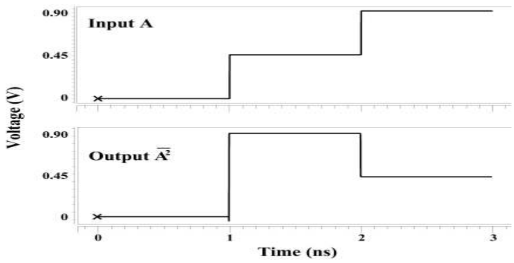


Fig. 11—Transient analysis of the proposed $\bar{A}^2$.

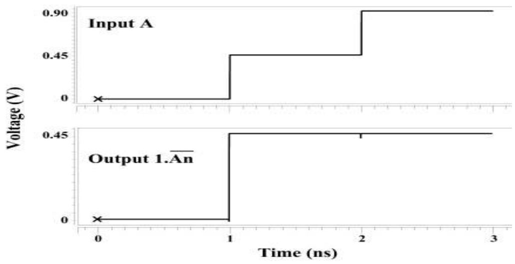


Fig. 12—Transient analysis of the proposed $1 \cdot \bar{A}_n$.

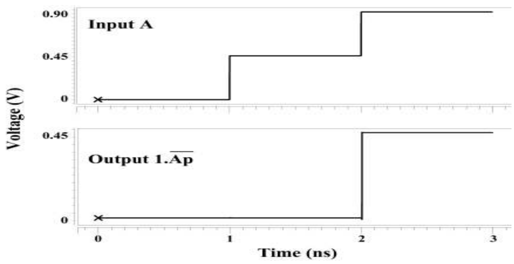


Fig. 13—Transient analysis of the proposed $1 \cdot \bar{A}_p$.

Figures 9 - 15 illustrate the transient analysis of the proposed five Unary Operators, the THA, and the TMUL.

TABLE XIII: Comparison of transistors count of THAs and TMULs

| | THA | TMUL |
|---|---|---|
| In **[13]** used TDecoder and Basic Logic Gates | 136 | 100 |
| In **[15]** used De Morgan's Law and two supply voltages | 85 | 61 |
| In **[18]** used Unary Operators, and TMUX | 64 | 58 |
| **Proposed models** use Unary Operators, TMUX, and two supply voltages | **39** | **34** |

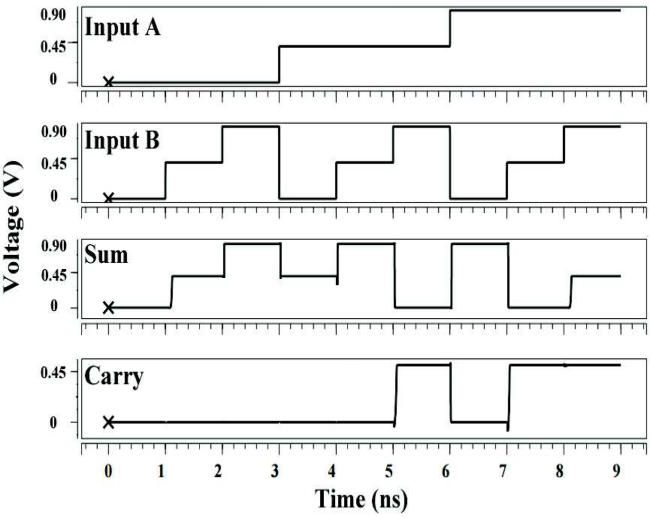


Fig. 14—Transient analysis of the proposed THA.

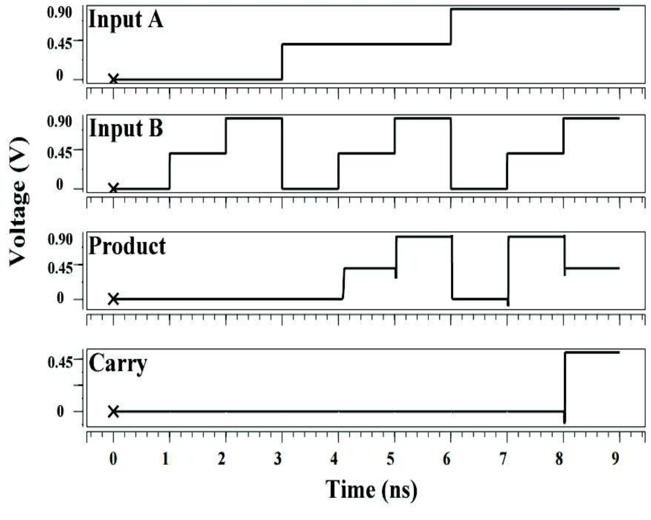


Fig. 15—Transient analysis of the proposed TMUL.

### A. Comparison of Transistors Count for all THAs and TMULs

Albeit not being the only factor, minimizing the transistors count is a good metric to decrease energy consumption.

Table XIII displays the comparison of the THA and TMUL in [13], [15], [18] in terms of transistors count.

The proposed THA has a significant reduction in transistors count 71.32%, 54.11%, and 39.1% compared to THA in [13], [15] and [18], respectively.

The proposed TMUL has a significant reduction in transistors count 66%, 44.26%, and 41.37% compared to TMUL in [13], [15] and [18], respectively.

### B. Voltage Variation of all THAs and TMULs

The impact of power supply variation (from 0.8 V to 1 V) on the performance of all circuits is studied.

Fig.16 and Fig.17 show the comparison to the existing THA and TMUL in [13], [15] and [18] in terms of the average power consumption (Fig.16(a) and 17(a)), maximum propagation delay (Fig.16(b) and 17(b)), and PDP (Fig.16(c) and 17(c)) for a fixed frequency at 1 GHz, temperature at 27°C, and by varying the supply voltages (from 0.8 V to 1 V).

As shown in Fig.16(c), the proposed THA shows a significant reduction in PDP compared to [13], [15] and [18], respectively. At Vdd = 0.8 V, 99.62%, 97.22%, and 80.1%. At Vdd = 0.9 V, 99.14%, 96.89%, and 85.41%. At Vdd = 1 V, 98.32%, 92.73%, and 85.68%.

As shown in Fig.17(c), the proposed TMUL shows a significant reduction in PDP compared to [13], [15] and [18], respectively. At Vdd = 0.8 V, 98.88%, 94.99%, and 79.10%. At Vdd = 0.9 V, 99.07%, 96.48%, and 92.39%. At Vdd = 1 V, 98.99%, 96.3%, and 93.63%.

### C. Temperature Variation of all THAs and TMULs

Temperature noise is one of the most critical issues influencing the circuit's efficiency.

The effect of temperature variation (from 10°C to 70°C) on the performance of all circuits is studied.

Fig.18 and Fig.19 show the comparison to the existing THA and TMUL in [13], [15] and [18] in terms of the average power consumption (Fig.18(a) and 19(a)), maximum propagation delay (Fig.18(b) and 19(b)), and PDP (Fig.18(c) and 19(c)) for a fixed frequency at 1 GHz, supply voltage at 0.9 V, and by varying the temperatures (from 10°C to 70°C).

As shown in Fig.18(c), the proposed THA shows a significant reduction in PDP compared to [13], [15] and [18], respectively. At Temperature = 10°C, 99.16%, 97.27%, and 83.85%. At Temperature = 27°C, 99.14%, 96.89%, and 85.41%. At Temperature = 70°C, 98.91%, 96.39%, and 84.1%.

As shown in Fig.19(c), the proposed TMUL shows a significant reduction in PDP compared to [13], [15] and [18], respectively. At Temperature = 10°C, 98.88%, 96.19%, and 89.66%. At Temperature = 27°C, 99.07%, 96.48%, and 92.39%. At Temperature = 70°C, 98.84%, 96.11%, and 91.59%.

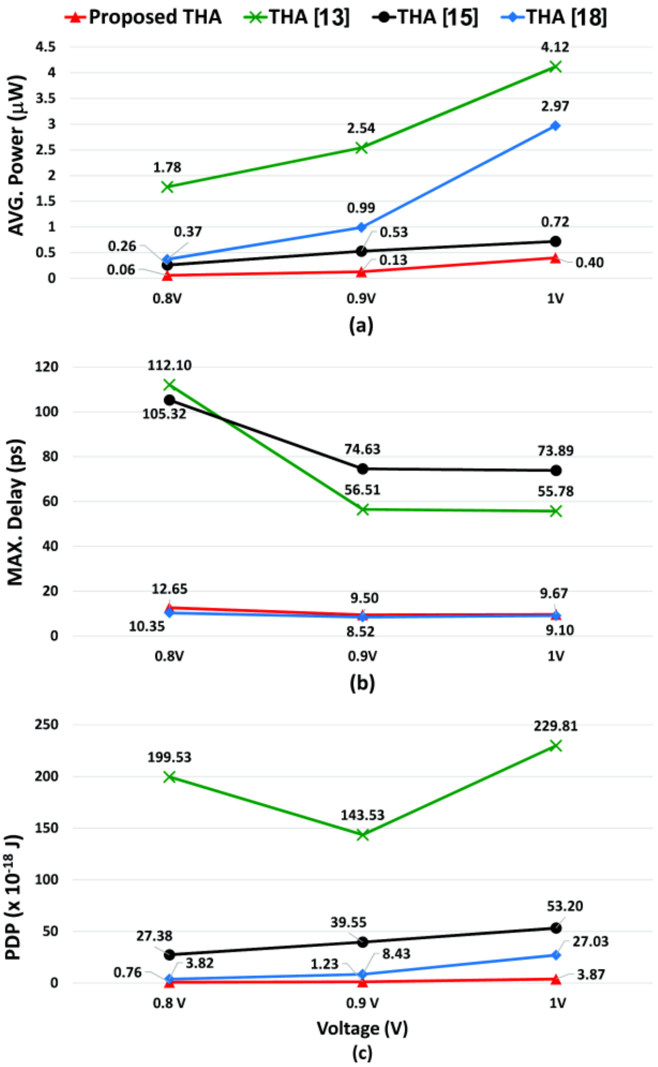


Fig. 16—Voltage variation of All THAs: (a) For Average Power, (b) for Maximum Delay, and (c) for PDP.

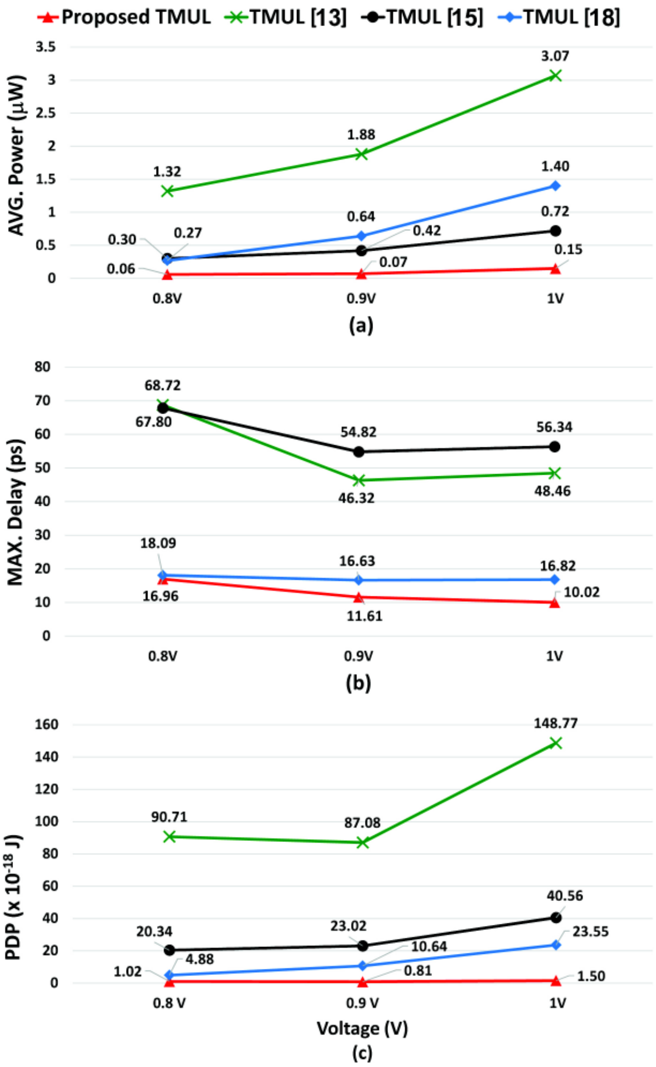


Fig. 17—Voltage variation of All TMULs: (a) For Average Power, (b) for Maximum Delay, and (c) for PDP.

### *D. Frequency Variation of all THAs and TMULs*

Electronic circuits behave very differently at high frequencies due to a change in the behavior of all circuit components.

The effect of frequency variation (from 0.5GHz to 2GHz) on the performance of all circuits is studied.

Fig.20 and Fig.21 show the comparison to the existing THA and TMUL in [13], [15] and [18] in terms of the average power consumption (Fig.20(a) and 21(a)), maximum propagation delay (Fig.20(b) and 21(b)), and PDP (Fig.20(c) and 21(c)) for a fixed supply voltage of 0.9 V, temperature of 27°C, and by varying the frequencies (from 0.5 GHz to 2 GHz).

As shown in Fig.20(c), the proposed THA shows a significant reduction in PDP compared to [13], [15] and [18], respectively. At frequency = 0.5 GHz, 99.22%, 96.9%, and 89.62%. At frequency = 1 GHz, 99.14%, 96.89%, and 85.41%. At frequency = 2 GHz, 98.94%, 96.18%, and 84.69%.

As shown in Fig.21(c), the proposed TMUL shows a significant reduction in PDP compared to [13], [15] and [18], respectively. At frequency = 0.5 GHz, 99.14%, 96.50%, and 93.33%. At frequency = 1 GHz, 99.07%, 96.48%, and 92.39%. At frequency = 2 GHz, 98.87%, 95.71%, and 81.99%.

### *E. Process Variations of all THAs and TMULs*

Process variations have a strong impact on the performance and robustness of devices and circuits. Therefore, all the THA and TMUL circuits are tested in the presence of major process variations: TOX, CNT diameter, CNT's count, and channel length [25].

TOX:

In the Stanford CNFET model, TOX is the oxide thickness of the Gate Dielectric $k_1$ material ($HfO_2$), as shown in Fig. 22. The variation in TOX will lead to leakage current. By decreasing TOX, the leakage current will increase, then the PDP will also increase and Vise Versa.

CNT Diameter:

The variance of the CNT diameter is one of the multiple problems of CNFET imperfections caused due to nonidealities

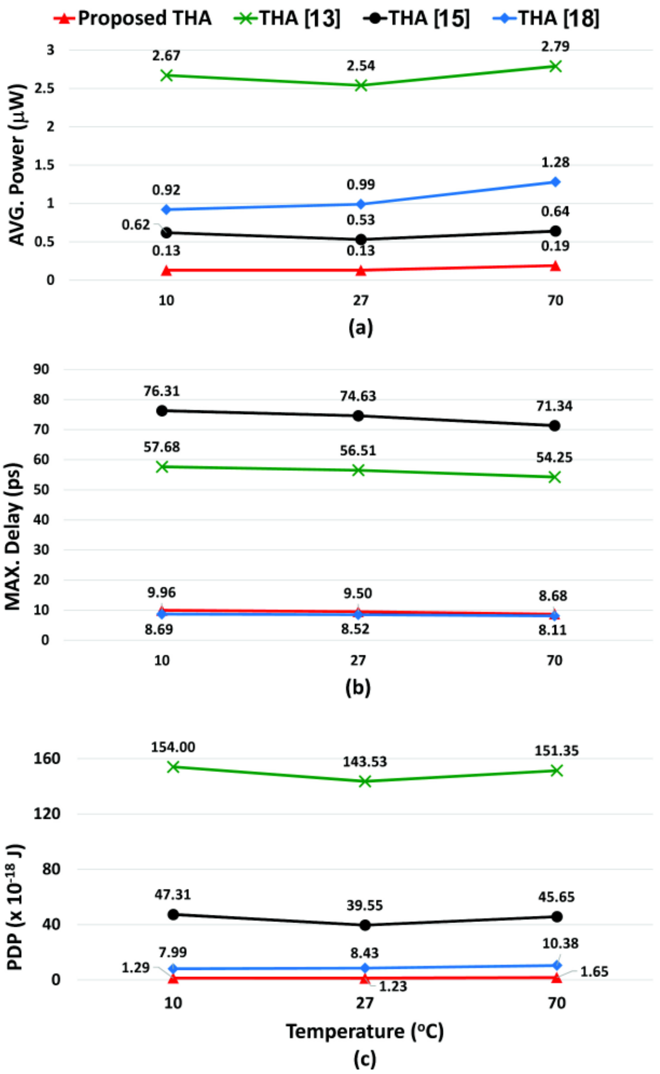


Fig. 18—Temperature Variation of All THAs: (a) For Average Power, (b) For Maximum Delay, and (c) for PDP.

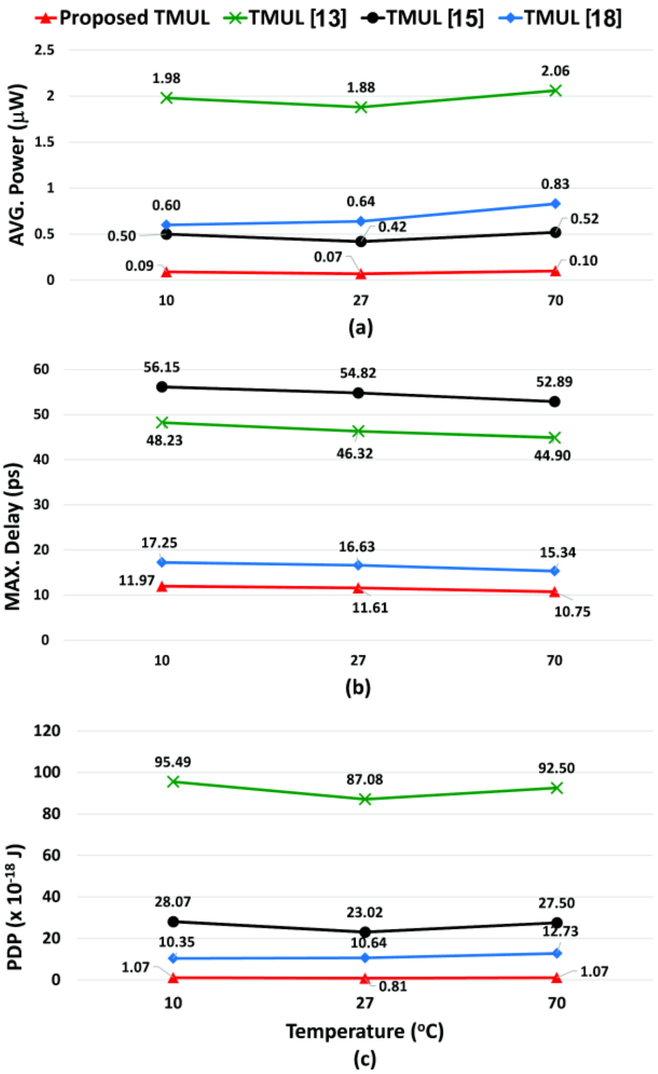


Fig. 19—Temperature Variation of All TMULs: (a) For Average Power, (b) For Maximum Delay, and (c) for PDP.

in the CNT transistors. This variation will lead to variation in threshold voltage, which negatively affects the performance of CNFET circuits. This problem has more impact on MVL circuits where transistors with different threshold voltages are used.

CNT's Count:

The variation in the CNT's count results in changing the output current of the transistor, which can cause a problem in the operation of the circuit.

Channel Length:

The variation in channel length will lead to the variation of the channel between drain and source, which affects the performance of CNFET circuits.

Monte Carlo analysis:

It is based on statistical distributions. It realistically simulates mismatching and process variations. In each simulation run, it calculates every parameter randomly according to a statistical distribution model.

Therefore, this paper uses Monte Carlo analysis based on the Gaussian distributions with ±5%, ±10%, and ±15% variations at the ±3 $\sigma$ level with the number of simulation running is equal to 1000.

The energy consumption (PDP) variations of all THA and TMUL circuits in the presence of the major process variations are shown in Fig. 23 and Fig. 24.

As shown in Fig. 23 and Fig. 24, The proposed THA and TMUL have a lower sensitivity to process variations and are more robustness compared to the other designs because their PDP variations are the smallest among all the investigated circuits.

### *F. Noise Effect of all THAs and TMULs*

Digital circuits are inherently noise-tolerant, and they are only affected by noises with high amplitude and wide width.

The Noise Immunity Curve (NIC) is used to determine the impact of noisy inputs on all THA and TMUL circuits.

The noise signal, Fig.25, is injected into inputs of THAs and TMULs.

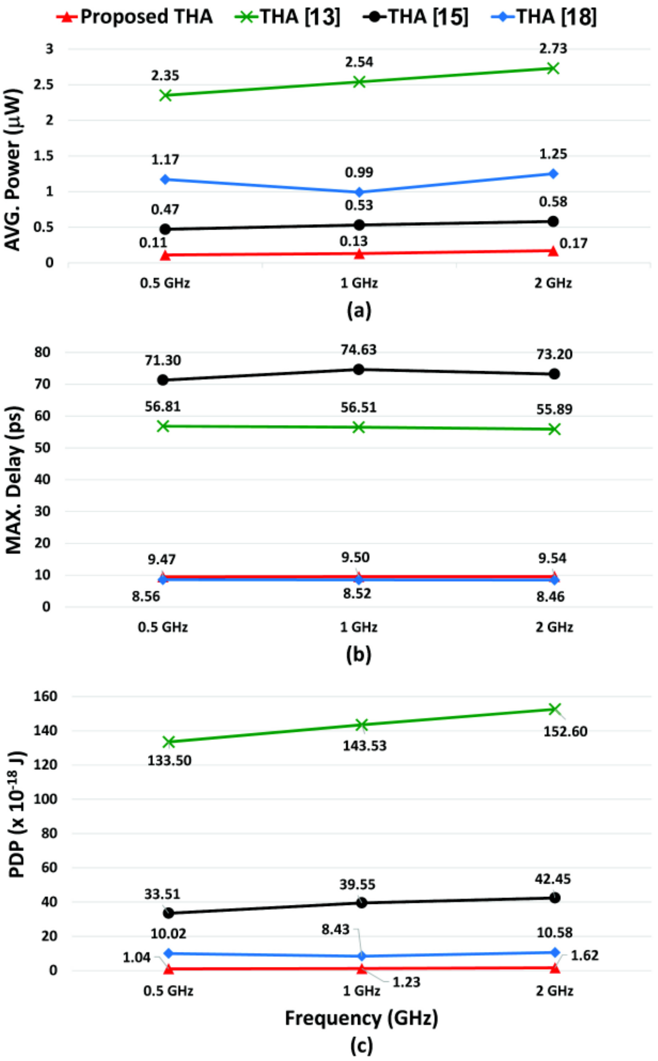


Fig. 20—Frequency Variation of All THAs: (a) For Average Power, (b) For Maximum Delay, and (c) for PDP.

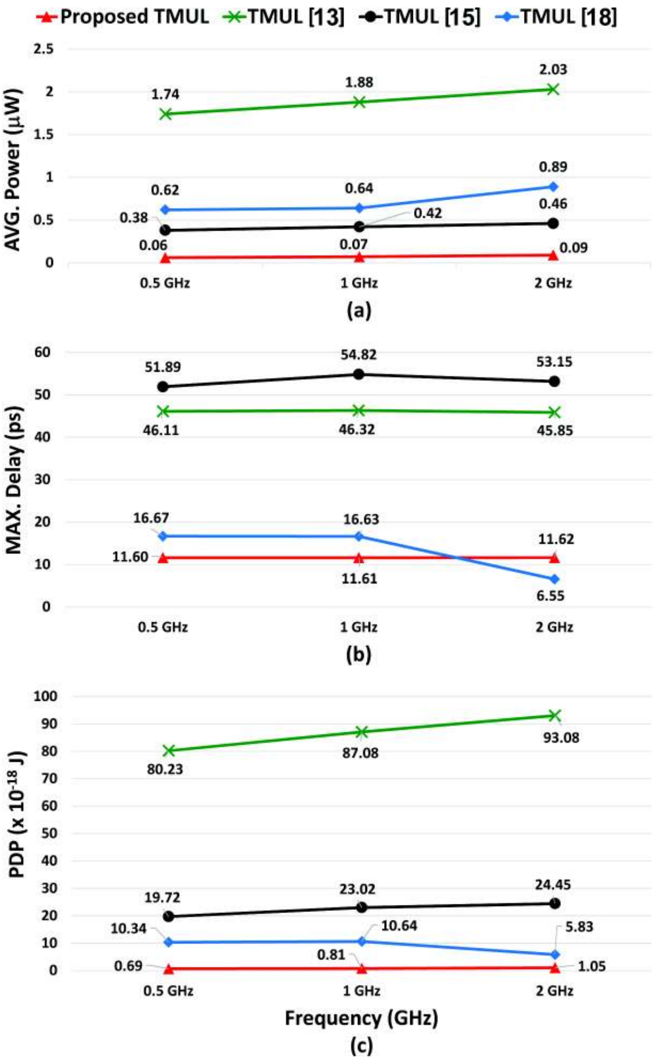


Fig. 21—Frequency Variation of All TMULs: (a) For Average Power, (b) For Maximum Delay, and (c) for PDP.

As shown in Fig.25, the noise signal has pulse width ($W_n$) and pulse amplitude ($V_n$).

Each point on the NIC curve is a pair of ($W_n$, $V_n$). Above that point, the circuit will produce an error on the output. The region above the NIC curve is an unsafe zone, whereas the region below the NIC curve is a safe zone against noise pulses.

Therefore, any circuit with higher NIC shows a more noise-tolerant circuit [26].

As shown in Fig. 26 and Fig. 27, The proposed THA and TMUL show higher noise immunity compared to the other designs.

As shown through the presented results, the proposed circuits achieve the lowest PDP among all the considered implementation for different simulation parameters (voltage, temperature, frequency). This is aligned with the main purpose of this work, which consists of designing an energy-efficient implementation suitable for low-power portable electronics and embedded systems to preserve battery consumption.

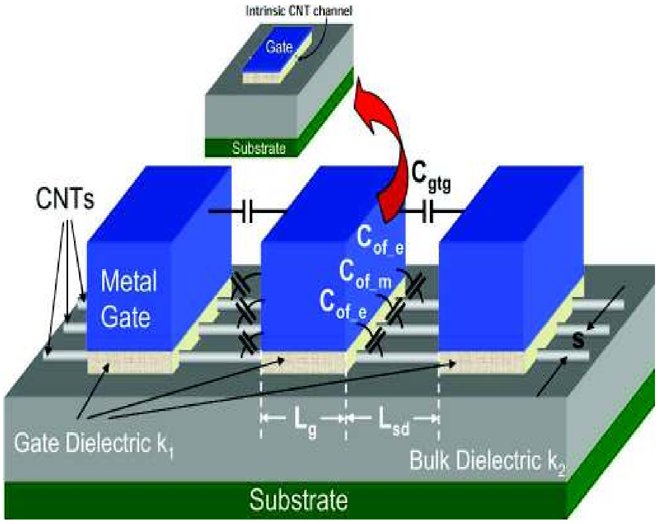


Fig. 22—Stanford CNFET Model.

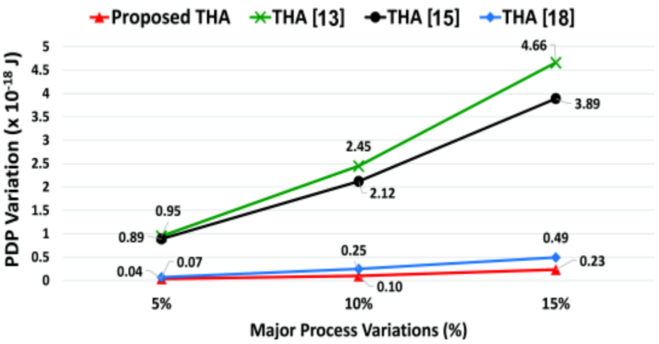


Fig. 23—THA Major Process Variations: TOX, CNT Diameter, CNT's Count, and Channel length.

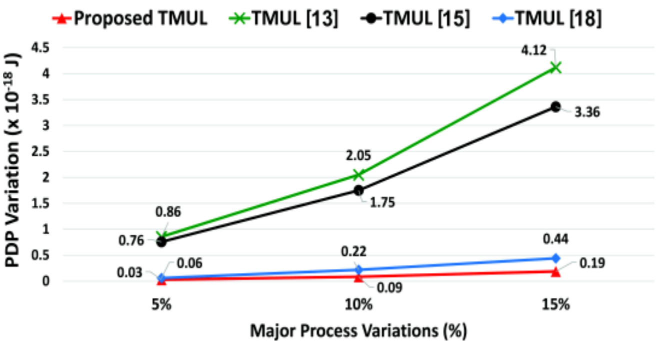


Fig. 24—TMUL Major Process Variations: TOX, CNT Diameter, CNT's Count, and Channel length.

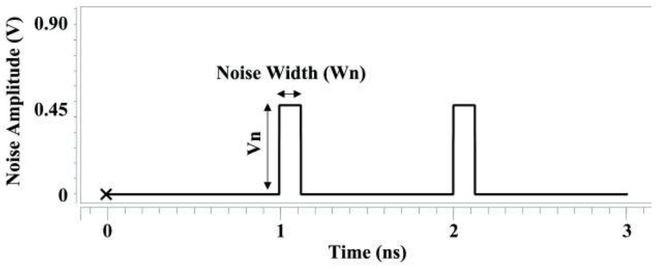


Fig. 25—Noise Signal.

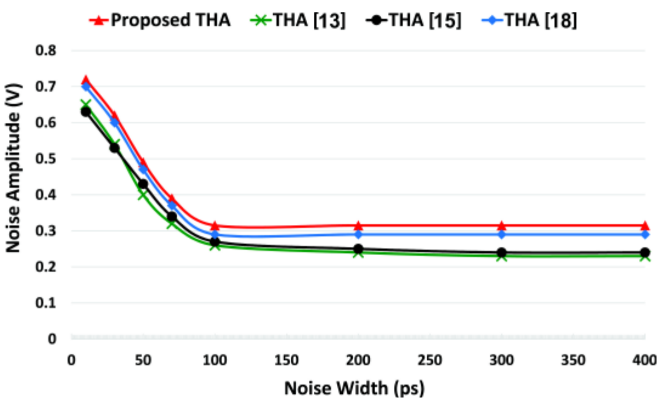


Fig. 26—THA Noise Immunity Curve (NIC).

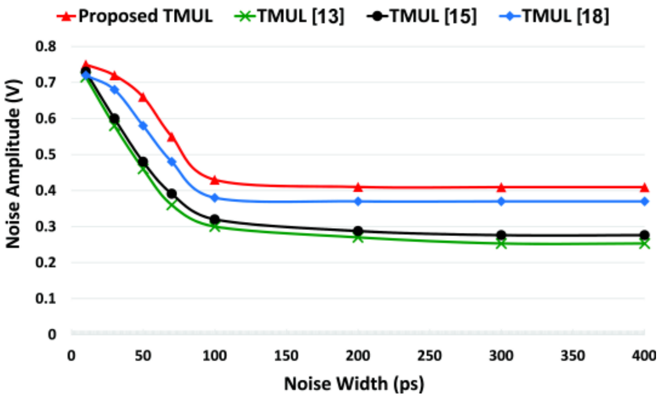


Fig. 27—TMUL Noise Immunity Curve (NIC).

## VI. Conclusion

This paper proposed new designs of five Unary Operators combined with Ternary Multiplexer to design a Ternary Half Adder and Ternary Multiplier, using 32 nm channel CNFET, which aims to optimize the trade-off between performance and energy efficiency.

The design process utilizes different techniques in terms of transistor arrangement, two supply voltages (Vdd, Vdd/2), transistor count reduction to reach the final target.

The comparison of the proposed approach to existing designs shows significant performance gains for different simulation environments using HSPICE simulator with voltage variation, temperature variation, and frequency variation. Moreover, Monte Carlo analysis for major process variations (TOX, CNT Diameter, CNT's Count, and Channel length) was studied. The results confirmed that the proposed circuits had higher robustness, among other designs. In addition, the noise immunity curve (NIC) showed that the proposed circuits had a higher noise tolerance than other models.

Therefore, the proposed circuits can be implemented in low-power portable electronics and embedded systems to preserve battery consumption.

## References

[1] J. Liang, L. Chen, J. Han, F. Lombardi, Design and evaluation of multiple valued logic gates using pseudo N-Type carbon nanotube FETs, IEEE Trans. Nanotechnology 13 (4) (2014) 695-708, https://doi.org/10.1109/TNANO.2014.2316000.

[2] S.L. Hurst, Multiple-valued logic its status and its future, IEEE Transactions on Computers 133 (1984) 1160–1179, https://doi.org/10.1109/TC.1984.1676392.

[3] T. Lengauer, S. Niiher, An analysis of ternary simulation as a tool for race detection in digital MOS circuits, Integration, the VLSI Journal 4 (4) (1986) 309 –30. https://doi.org/10.1016/0167-9260(86)90012-X.

[4] S.D. Mahya, F.M. Reza, N. Keivan, B. Nader. High-performance ternary operators for scrambling. Integration, the VLSI Journal 59 (1) (2017) 1–9. https://doi.org/10.1016/j.vlsi.2017.03.010.

[5] N. Saleh, A. Kassem, A.M. Haidar, Energy-efficient architecture for wireless sensor networks in healthcare applications, IEEE Access 6 (2018) 6478 - 6486. https://doi.org/10.1109/ACCESS.2018.2789918.

[6] Q. Yang, B. Zhu, S. Wu, An architecture of cloud-assisted information dissemination in vehicular networks, IEEE Access 4 (2016) 2764-2770. https://doi.org/10.1109/ACCESS.2016.2572206.

[7] M. Abdelaziz, T.A. Gulliver, Ternary trellis coded modulation, IEEE Access 7 (2019) 49027-49038. https://doi.org/10.1109/ACCESS.2019.2909707.

[8] I. Bayram, Y. Chen, NV-TCAM: Alternative designs with NVM devices, Integration, the VLSI Journal 62 (2018) 114-122. https://doi.org/10.1016/j.vlsi.2018.02.003.
[9] C. Geunho, F. Lombardi, Design and process variation analysis of CNFET based ternary memory cells, Integration, the VLSI Journal 54 (2016) 97–108. https://doi.org/10.1016/j.vlsi.2016.02.003.
[10] N. Soliman, M.E. Fouda, A.G. Alhurbi, L.A. Said, A.H. Madian, A.G. Radwan, Ternary functions design using memristive threshold logic, IEEE Access 7 (2019) 48371-48381. https://doi.org/10.1109/ACCESS.2019.2909500.
[11] R.A. Jaber, A.M. El-Hajj, L.A. Nimri, A.M. Haidar, A Novel implementation of ternary decoder using CMOS DPL binary gates, 2018 Int. Arab Conf. on Information Technology (ACIT) (2018) 1-3, Lebanon. https://doi.org/10.1109/ACIT.2018.8672698.
[12] D. Kundu, S. Guin, G.N. Jyothi, S. Sridevi, High Speed FinFET Traff Comparator Based Function Generator, 2018 International Conference on Computation of Power, Energy, Information and Communication (ICCPEIC) (2018), India. https://doi.org/10.1109/ICCPEIC.2018.8525184.
[13] S. Lin, Y.B. Kim, F. Lombardi, CNTFET-based design of ternary logic gates and arithmetic circuits, IEEE Transactions on Nanotechnology 10 (2011) 217-225. https://doi.org/10.1109/TNANO.2009.2036845.
[14] H. Samadi, A. Shahhoseini, F. Aghaei-liavali, A New method on designing and simulating CNTFET-based ternary gates and arithmetic circuits, Microelectronics Journal 63 (2017) 41-48. https://doi.org/10.1016/j.mejo.2017.02.018.
[15] R.A. Jaber, A. Kassem, A.M. ElHajj, L.A. Nimri, A.M. Haidar, High-Performance and Energy-Efficient CNFET-Based Designs for Ternary Logic Circuits, IEEE Access 7 (2019) 93871-93886. https://doi.org/10.1109/ACCESS.2019.2928251.
[16] S. Tabrizchi, A. Panahi, F. Sharifi, K. Navi, N. Bagherzadeh, Method for designing ternary adder cells based on CNFETs, IET Circuits, Devices & Systems 11 (2017) 465-470. https://doi.org/10.1049/iet-cds.2016.0443.
[17] D. Das, A. Banerjee, V. Prasad, Design of ternary logic circuits using CNTFET, 2018 Int. Symp. On Devices, Circuits and Systems (ISDCS) (2018), India. https://doi.org/10.1109/ISDCS.2018.8379661
[18] B. Srinivasu, K. Sridharan, A synthesis methodology for ternary logic circuits in emerging device technologies, IEEE Transactions on Circuits and Systems I: Regular Papers 64 (8) (2017) 2146–2159, https://doi.org/10.1109/TCSI.2017.2686446.
[19] G. Hills, M.G. Bardon, G. Doornbos, D. Yakimets, P. Schuddinck, R. Baert, D. Jang, L. Mattii, S.Y. Sherazi, D. Rodopoulos, R. Ritzenthaler, C.-S. Lee, A. Thean, I. Radu, A. Spessot, P. Debacker, F. Catthoor, P. Raghavan, M. Shulaker, H.-S. Philip Wong, S. Mitra, Understanding energy efficiency benefits of carbon nanotube field-effect transistors for digital VLSI, IEEE Transactions on Nanotechnology 17 (6) (2018) 1259-1269. https://doi.org/10.1109/TNANO.2018.2871841.
[20] E. Shahrom, S. A. Hosseini, A new low power multiplexer based ternary multiplier using CNTFETs, AEU - International Journal of Electronics and Communications 93 (2018) 191-207. https://doi.org/10.1016/j.aeue.2018.06.011.
[21] Stanford University CNFET model Website. http://nano.stanford.edu/model.php?id = 23, (accessed 5 Dec. 2019).
[22] J. Deng, H.-S. P. Wong, A compact SPICE model for carbon-nanotube field-effect transistors including nonidealities and its application - Part I: model of the intrinsic channel region, IEEE Trans. Electron Devices 54 (12) (2007) 3186-3194. https://doi.org/10.1109/TED.2007.909030.
[23] J. Deng, H.-S. P. Wong, A compact SPICE model for carbon-nanotube field-effect transistors including nonidealities and its application - Part II: full device model and circuit performance benchmarking, IEEE Trans. Electron Devices 54 (12) (2007) 3195-3205. https://doi.org/10.1109/TED.2007.909043.
[24] D. M. Miller, M. A. Thornton, Multiple Valued Logic: Concepts and Representations, San Rafael, CA, USA: Morgan & Claypool, 2008, pp. 32. https://doi.org/10.2200/S00065ED1V01Y200709DCS012.
[25] S.A. Ebrahimi, M.R. Reshadinezhad, A. Bohlooli, A new design method for imperfection-immune CNFET-based circuit design, Microelectronics Journal 85 (2019) 62-71. https://doi.org/10.1016/j.mejo.2019.01.013.
[26] G. Balamurugan, N.R. Shanbhag, The Twin-Transistor Noise-Tolerant Dynamic Circuit Technique, IEEE Journal of Solid-State Circuits 36 (2) (2001) 273-280. https://doi.org/10.1109/4.902768.
