# Supplementary material for: Multiple-Valued Logic Circuit Design and Data Transmission Intended for Embedded Systems
Source: arXiv:2211.04542 source file (2022-11-08)
Supplement: Supplementary file 5 [file BTC_DPL.pdf]

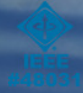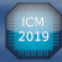

**ICM 2019**

[ABOUT](#) ▾

[CALL FOR  
CONTRIBUTIONS](#) ▾

[COMMITTEE](#)

[IMPORTANT  
DATES](#)

[REGISTRATION](#)

[TRAVEL &  
ACCOMMODATION](#)

# *The 31st International Conference on Microelectronics*

*(ICM 2019) December 15-18*

[CALL FOR PAPER pdf](#)

[SUBMISSION](#)

# A Novel Binary to Ternary Converter using Double Pass-Transistor Logic

Ramzi A. Jaber\*, Ahmad M. El-Hajj, Ali M. Haidar  
*Depart. of Electrical & Computer Engineering*  
*Beirut Arab University (BAU)*  
Debbieh, Lebanon  
{r.jaber\*, a.elhajj, ari}@bau.edu.lb

Abdallah Kassem  
*Depart. of Electrical & Computer Engineering*  
*Notre Dame University (NDU)*  
Louaize, Lebanon  
akassem@ndu.edu.lb

Lina A. Nimri  
*Department of Business Computer*  
*Lebanese University*  
Beirut, Lebanon  
lnimri@ul.edu.lb

**Abstract**—The ternary circuit has an advantage over the binary circuit concerning interconnect complexity, propagation delay, and energy consumption. This paper proposes a novel binary-to-ternary converter using Double Pass-Transistor (DPL) with four bits as input and three trits as output. The importance of this work is gained through its potential to increase the data rate, and reduce power consumption. Also, the proposed converter can be used as a bridge between binary and ternary circuits. The proposed circuit is simulated and tested using Micro-Cap V10 PSPICE simulator with CMOS process technology. It is then compared to different binary-to-ternary converters to conclude that significant improvement achieved.

**Index Terms**—CMOS, Double Pass-Transistor Logic (DPL), Logic circuit, Multi-Valued Logic (MVL), Ternary system.

## I. INTRODUCTION

The limitations in binary circuits are mainly due to a large number of connections, thus requiring a big chip area and a notable increase in energy consumption. Whereas, Multiple-Valued Logic (MVL), has more than two values, helps in reducing the interconnections and the chip area, and energy consumption [1].

For the past decade, MVL has attracted researchers' attention over binary logic, and it has been used in several modern application areas such as Electronic Design Automation (EDA) tools to solve binary logic problems [2]. Moreover, MVL can be implemented in communication system [3], cloud vehicular networks [4], wireless sensor networks [5], circuit designs such as Logic Gates, Memory, Memristor circuit [6]–[10], and software (algorithm) [11].

Also, It has proven that radix three (ternary logic) is the most efficient radix in providing less complexity and cost efficiency as compared to other radices [12]. In addition two logic systems are available in ternary logic: balanced ternary logic (-1, 0, 1) correspond to (-V<sub>dd</sub>, 0, V<sub>dd</sub>), and simple ternary logic (0, 1, 2) correspond to (0, V<sub>dd</sub>/2, V<sub>dd</sub>). MVL enables much more data to store in a single digit, such as the decimal number 15 needs four binary digits (bits) to store

while four ternary digits (trits) are enough to store up to decimal number 80 ( $3^4-1$ ).

The design of binary-to-ternary converters has recently constituted an active area of research, and important papers are selected.

To illustrate, in [13], [14], a novel circuit that converts two binary bits to one ternary digit (trit) was proposed. In [15], the authors proposed a novel binary-to-ternary converter based on the Josephson junction (JJ). In [16], the designed converter circuit is characterized by a dual supply operation while in [17] the proposed circuit tailored in the context of Quantum-dot Cellular Automata. Finally, in [18], the authors proposed a novel binary-to-ternary converter based on DPL, which gives the best performance than all mentioned papers above.

All the aforementioned binary-to-ternary converters suffer from high power consumption [15], [16], large propagation delay [16], [18], complex circuit [16], [17] or even errors in the output when two binary inputs are set as high level voltage [13], [14].

Therefore, this paper proposes a novel binary-to-ternary converter which provides a drastic reduction in power consumption compared to circuits employing CMOS technology; also it lowers the propagation delay and provides a small, simple and error-free circuit implementation (for all possible inputs).

The proposed circuit converts four binary bits to three ternary trits by using Double Pass-Transistor Logic (DPL), and it is simulated using Micro-Cap V10 PSPICE simulator, demonstrates a notable reduction in devices count, propagation delay, and energy consumption.

The rest of the paper is organized as follows: A background of DPL presented in Section II. The proposed conversion approach described in Section III, Simulation results, and comparisons discussed in Section IV, followed by concluding remarks in section V.

## II. DOUBLE PASS-TRANSISTOR LOGIC (DPL)

As shown in Fig.1, DPL [19] is a modified version of complementary pass-transistor logic (CPL) by adding PMOS transistors in parallel with the NMOS transistors to eliminate the problems of noise margin and speed degradation at reduced supply voltages associated in CPL circuits. Besides, basic logic gates using DPL ideally have identical propagation delay so that it can use for time-equalized applications such as wave pipelining.

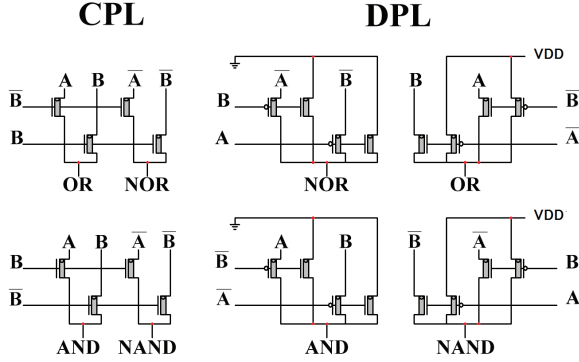

Fig. 1. DPL Gates Design [19]

## III. PROPOSED CONVERSION CIRCUIT

A novel four to three binary-to-ternary converter model is designed Fig.2.

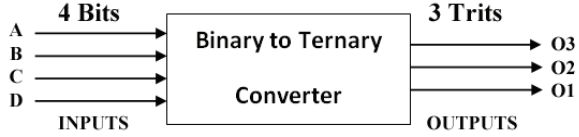

Fig. 2. binary-to-ternary model

As shown in Fig.2, four binary bits provide as input (A, B, C, D). The input “A” is the most significant bit (MSB), and the input “D” is the least significant bit (LSB). Three trits provided as output (O3, O2, O1). The output “O3” is the most significant trit (MST), and “O1” is the least significant trit (LST), using simple ternary logic (0, 1, 2).

Among the 27 trits combinations, only 16 used to represent all the four-bit combinations while the remaining 11 could be used for additional features such as error detection.

The 16 combinations that could produce in the converter circuit are shown in Table I. The voltage supply used in the proposed circuit is 1.8V to decrease power consumption. Therefore, DPL is used to eliminate the noise, as described in Section II.

Binary digits are (0: Low, and 1: High) and Ternary trits are (0: Low, 1: Medium, and 2: High). This paper will use, “0” represents low-level voltage (0V), “1” represents medium-level voltage (0.9V), and “2” represents high-level voltage (1.8V) for the both binary and ternary system.

TABLE I  
BINARY-TO-TERNARY TRUTH TABLE

| Decimal | Binary Inputs |   |   |   | Ternary Outputs |    |    |
|---------|---------------|---|---|---|-----------------|----|----|
|         | A             | B | C | D | O3              | O2 | O1 |
| 0       | 0             | 0 | 0 | 0 | 0               | 0  | 0  |
| 1       | 0             | 0 | 0 | 2 | 0               | 0  | 1  |
| 2       | 0             | 0 | 2 | 0 | 0               | 0  | 2  |
| 3       | 0             | 0 | 2 | 2 | 0               | 1  | 0  |
| 4       | 0             | 2 | 0 | 0 | 0               | 1  | 1  |
| 5       | 0             | 2 | 0 | 2 | 0               | 1  | 2  |
| 6       | 0             | 2 | 2 | 0 | 0               | 2  | 0  |
| 7       | 0             | 2 | 2 | 2 | 0               | 2  | 1  |
| 8       | 2             | 0 | 0 | 0 | 0               | 2  | 2  |
| 9       | 2             | 0 | 0 | 2 | 1               | 0  | 0  |
| 10      | 2             | 0 | 2 | 0 | 1               | 0  | 1  |
| 11      | 2             | 0 | 2 | 2 | 1               | 0  | 2  |
| 12      | 2             | 2 | 0 | 0 | 1               | 1  | 0  |
| 13      | 2             | 2 | 0 | 2 | 1               | 1  | 1  |
| 14      | 2             | 2 | 2 | 0 | 1               | 1  | 2  |
| 15      | 2             | 2 | 2 | 2 | 1               | 2  | 0  |

The procedure to build the proposed circuit starts with a novel technique by decomposition each ternary output in Table I to two intermediate binary outputs, as shown in Table II and Table III.

TABLE II

| Decomposition O1 to two intermediate Binary Outputs |                             |     |
|-----------------------------------------------------|-----------------------------|-----|
| Ternary Output                                      | Intermediate Binary Outputs |     |
| O1                                                  | O1a                         | O1b |
| Logic 0 (0V)                                        | 0                           | 0   |
| Logic 1 (0.9V)                                      | 0                           | 2   |
| Logic 2 (1.8V)                                      | 2                           | 0   |

TABLE III  
DECOMPOSITION OF THE THREE TERNARY OUTPUTS

| Binary Inputs |   |   |   | Ternary Outputs as Intermediate Binary |     |     |     |     |
|---------------|---|---|---|----------------------------------------|-----|-----|-----|-----|
| A             | B | C | D | O3b                                    | O2a | O2b | O1a | O1b |
| 0             | 0 | 0 | 0 | 0                                      | 0   | 0   | 0   | 0   |
| 0             | 0 | 0 | 2 | 0                                      | 0   | 0   | 0   | 2   |
| 0             | 0 | 2 | 0 | 0                                      | 0   | 0   | 2   | 0   |
| 0             | 0 | 2 | 2 | 0                                      | 0   | 2   | 0   | 0   |
| 0             | 2 | 0 | 0 | 0                                      | 0   | 2   | 0   | 2   |
| 0             | 2 | 0 | 2 | 0                                      | 0   | 2   | 2   | 0   |
| 0             | 2 | 2 | 0 | 0                                      | 2   | 0   | 0   | 0   |
| 0             | 2 | 2 | 2 | 0                                      | 2   | 0   | 0   | 2   |
| 2             | 0 | 0 | 0 | 0                                      | 2   | 0   | 2   | 0   |
| 2             | 0 | 0 | 2 | 2                                      | 0   | 0   | 0   | 0   |
| 2             | 0 | 2 | 0 | 2                                      | 0   | 0   | 0   | 2   |
| 2             | 0 | 2 | 2 | 2                                      | 0   | 0   | 2   | 0   |
| 2             | 2 | 0 | 0 | 2                                      | 0   | 2   | 0   | 0   |
| 2             | 2 | 0 | 2 | 2                                      | 0   | 2   | 0   | 2   |
| 2             | 2 | 2 | 0 | 2                                      | 0   | 2   | 2   | 0   |
| 2             | 2 | 2 | 2 | 2                                      | 2   | 0   | 0   | 0   |

The second step involves using Karnaugh maps to get an optimized circuit for each intermediate outputs in Table III. The minimization process results in equations 1- 5.

$$O1a = \overline{A} \overline{B} \overline{C} \overline{D} + \overline{A} \overline{B} \overline{C} D + \overline{A} \overline{B} \overline{C} \overline{D} + \overline{A} \overline{B} C \overline{D} + A \overline{B} C \overline{D} \quad (1)$$

$$O1b = \overline{A} \overline{B} \overline{C} D + \overline{A} \overline{B} \overline{C} \overline{D} + \overline{A} \overline{B} C D + \overline{A} \overline{B} C \overline{D} + A \overline{B} \overline{C} D \quad (2)$$

$$O2a = \bar{A}BC + \bar{A}B\bar{C}D + BCD + \bar{A}\bar{B}\bar{C}\bar{D} \quad (3)$$

$$O2b = B\bar{C} + A\bar{B}D + \bar{A}\bar{B}CD \quad (4)$$

$$O3b = AB + AC + AD \quad (5)$$

The resulting equations are implemented in the binary-to-ternary converter circuit shown in Fig. 3.

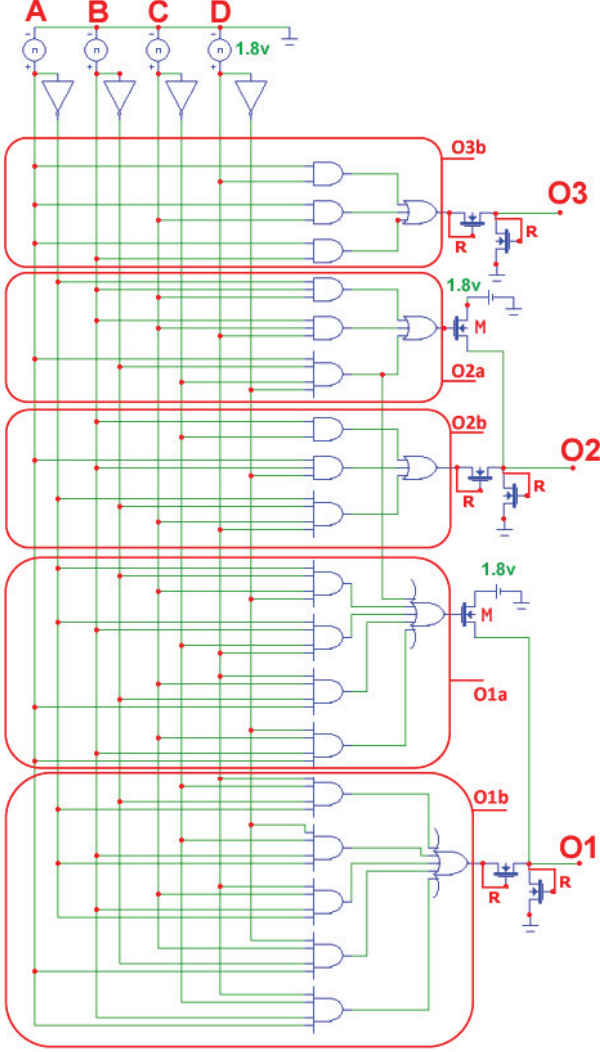

Fig. 3. Proposed binary-to-ternary Converter Circuit

Fig.3 represents the binary-to-ternary converter with four binary inputs (A, B, C, D) and three ternary outputs (O1, O2, O3). The intermediate binary outputs labeled as O1a, O1b, O2a, O2b, and O3b.

An enhancement MOSFET (M) used as a switch with its input (O1a or O2a). When O1a or O2a is at high-level voltage, then the transistor M will be turned “ON” to pass the 1.8 volts to final output O1, and it will be “OFF” when the O1a or O1b is a low-level voltage.

Similarly, two transistors (R) added after intermediate outputs (O1b, O2b, O3b), that act as a voltage divider. For

TABLE IV  
COMBINATION OF TERNARY OUTPUT O1

| O1a  | O1b  | Transistor (M)                                                                   | (2 Rs)  | O1             |
|------|------|----------------------------------------------------------------------------------|---------|----------------|
| 0V   | 0V   | OFF                                                                              | Req     | 0V (Logic 0)   |
| 0V   | 1.8V | OFF                                                                              | Divider | 0.9V (Logic 1) |
| 1.8V | 0V   | ON                                                                               | Req     | 1.7V (Logic 2) |
| 1.8V | 1.8V | <b>This Case Does Not Exist*</b><br><b>Whereas, in [13] and [14] have errors</b> |         |                |

example, when O1b is equal to 1.8V, then the output O1 is equal to 0.9V. When O1b is equal to 0V and O1a is equal to 1.8V, then the two transistors (Rs) will become two parallel resistors with equivalent resistance (Req) which will drop the output voltage O1 to 1.7V, as described in Table IV.

The same procedure will be done for output (O2) and (O3).

\* The proposed design has a notable advantage over previous converter designs in [13] and [14] since no error occurs for any input combination. As demonstrated in Tables III and IV, the intermediate binary outputs Oia, and Oib (i=1, 2) cannot be high at the same time which offers a significant advantage in simplifying the circuit.

The numbers count of devices in the proposed circuit calculated in Table V.

TABLE V  
DEVICE COUNT IN PROPOSED CIRCUIT (FIG.3)

| Device Name                                   | No. of devices | No. of Transistors | Subtotal   |
|-----------------------------------------------|----------------|--------------------|------------|
| Inverter Gate                                 | 4              | 1 input *2 =2      | 8          |
| 2 inputs AND Gate                             | 2              | 2 inputs *2 = 4    | 8          |
| 3 inputs AND Gate                             | 3              | 3 inputs *2 = 6    | 18         |
| 4 inputs AND Gate                             | 11             | 4 inputs *2 = 8    | 88         |
| 3 inputs OR Gate                              | 3              | 3 inputs *2 = 6    | 18         |
| 5 inputs OR Gate                              | 2              | 5 inputs *2 = 10   | 20         |
| MOSFET                                        | 8              | 1                  | 8          |
| Internal Resistor (one per each gate Fig.1)   |                |                    | 25         |
| Internal Capacitor (one per each gate Fig. 1) |                |                    | 25         |
| <b>Total No. of Devices</b>                   |                |                    | <b>218</b> |

#### IV. SIMULATION RESULTS AND COMPARISONS

In [18], the authors proposed a novel binary-to-ternary converter based on DPL, which gives the best performance than binary-to-ternary converters in [13]–[17].

Therefore, the proposed converter will be compared to the latest converter circuit designs described in [18].

For fair comparisons, both circuits are implemented, simulated, and analyzed using the same software Micro-Cap V10 PSpice Simulator with CMOS technology 0.18  $\mu\text{m}$ .

The simulated circuits utilize an implementation of the AND and OR DPL gates as previously described in [19] and shown in Fig.1. With a temperature of 25°C, average propagation delay (42.56 ps), and the average power (4.08  $\mu\text{W}$ ), as states in [20].

Fig.4 shows the simulation transient analysis of the proposed circuit with a temperature of 25°C, power supply (1.8V), and frequency (5GHz).

The following performance metrics will be used to compare to [18]: the frequency, the device count inside the circuit, the



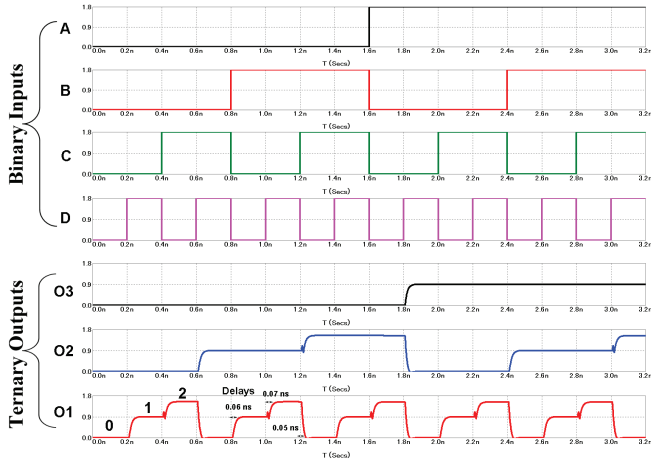

Fig. 4. The simulation transient analysis of proposed circuit

maximum propagation delay, the average power consumption, the maximum energy consumption, and the type of used logic gates.

The propagation delays in the proposed circuit are: From ternary “0” to “1” is 0.06 ns, from “1” to “2” is 0.07 ns and from “2” to “0” is 0.05 ns.

From the simulator, the average power consumption of the proposed circuit is 349.9  $\mu$ w.

Table VI summarizes that comparison.

TABLE VI  
COMPARISON TO THE LATEST NOVEL CONVERTER IN [18]

|                    | Converter [18]         | Proposed          | Improvement     |
|--------------------|------------------------|-------------------|-----------------|
| Frequency          | 0.33 GHz               | 5 GHz             | 1415%           |
| Device Count       | 426                    | 218               | 48.83%          |
| MAX. Delay         | 0.91 ns                | 0.07 ns           | 92.31%          |
| Avg. Power         | 270.42 $\mu$ w         | 349.9 $\mu$ w     | -29.4%          |
| MAX. Energy        | 246 $10^{-18}$ J       | 24.5 $10^{-18}$ J | 90%             |
| Type of used gates | Ternary & binary gates | binary gates      | Faster, as [21] |

The proposed (4:3) converter is bigger than the latest (3:2) converter in [18]. Despite that, the proposed converter gets better results compared to [18], as shown in Table VI.

## V. CONCLUSION

This paper proposes a binary-to-ternary converter with novel techniques. The proposed approach takes four bits and produces three trits using Double Pass-Transistor (DPL). The circuit designed and simulated using Micro-Cap V10 PSPICE simulator. Finally, logical analysis and simulation results demonstrate the merits of the approach in terms of reduced latency and energy consumption compared to other converters.

## REFERENCES

- [1] S. Hosseini, S. Etezadi, A novel very low-complexity multi-valued logic comparator in nanoelectronics, Springer Circuits, Systems, and Signal Processing 2 (June 2019) 1 – 22, <https://doi.org/10.1007/s00034-019-01158-2>.
- [2] D. Miller, M. Thornton, Multiple Valued Logic: Concepts and Representations., 12, Morgan & Claypool, San Rafael, CA, USA, 2008.
- [3] M. Abdelaziz, T. Gulliver, Ternary trellis coded modulation, IEEE Access 7 (April 2019) 49027 – 49038, <https://doi.org/10.1109/ACCESS.2019.2909707>.
- [4] Q. Yanq, B. Zhu, S. Wu, An architecture of cloud-assisted information dissemination in vehicular networks, IEEE Access 4 (May 2016) 2764 – 2770, <https://doi.org/10.1109/ACCESS.2016.2572206>.
- [5] N. Saleh, A. Kassem, A. Haidar, Energy-efficient architecture for wireless sensor networks in healthcare applications, IEEE Access 6 (Jan. 2018) 6478 – 6486, <https://doi.org/10.1109/ACCESS.2018.2789918>.
- [6] R. Jaber, A. El-Hajj, L. Nimri, A. Haidar (Eds.), A Novel implementation of ternary decoder using CMOS DPL binary gates, 2018 Int. Arab Conf. on Information Technology (ACIT), IEEE, Werdanye, Lebanon, 2018, <https://doi.org/10.1109/ACIT.2018.8672698>.
- [7] R. Jaber, A. Kassem, A. El-Hajj, L. Nimri, A. Haidar, High-performance and energy-efficient cnfet-based designs for ternary logic circuits, IEEE Access 7 (July 2019) 93871 – 93886, <https://doi.org/10.1109/ACCESS.2019.2928251>.
- [8] L. Sardinha, D. Silva, M. Vieira, L. Vieira, O. Neto, Tcam/cam-qca: (ternary) content addressable memory using quantum-dot cellular automata, Microelectronics Journal 46 (7) (July 2015) 563–571, <https://doi.org/10.1016/j.mejo.2015.03.020>.
- [9] N. Soliman, M. Fouda, A. Alhurb, L. Said, A. Madian, A. Radwan, Ternary functions design using memristive threshold logic, IEEE Access 7 (April 2019) 48371–48381, <https://doi.org/10.1109/ACCESS.2019.2909500>.
- [10] N. Soliman, M. Fouda, A. Radwan, Memristor-cntfet based ternary logic gates, Microelectronics Journal 72 (Feb. 2018) 74–85, <https://doi.org/10.1016/j.mejo.2017.12.008>.
- [11] D. Miller, M. Soeken (Eds.), A spectral algorithm for ternary function classification, Vol. 1 of 1, IEEE 48th Int. Symp. on Multiple-Valued Logic (ISMVL), IEEE, Linz, Austria, 2018.
- [12] S. Hurst, S. Etezadi, Multiple-valued logic its status and its future, IEEE Transactions on Computers 133 (1) (Dec. 1984) 1160 – 1179, <https://doi.org/10.1109/TC.1984.1676392>.
- [13] T. Kurt M, “binary to ternary converter”, US Patent 3,217,316, <https://patents.google.com/patent/US3217316A/en> (12 1961).
- [14] Y. Nakanishi, T. Kawaguchi, M. Sekiya, “pulse synthesizing circuit”, US Patent 9,287,867, <https://patents.google.com/patent/US9287867B2/en> (2016).
- [15] F. Li, M. Morisue, T. Ogata, “a proposal of josephson binary-to-ternary converter”, IEEE Transactions on Applied Superconductivity Vol.5 (2) (1995) 2632–2635.
- [16] B. Zlatko, D. Bundalo, F. Softic, M. Kostadinovic (Eds.), “Interconnection of binary and ternary CMOS digital circuits and systems”, Vol. 1 of 1, The 33rd International Convention MIPRO, IEEE, Opatija, Croatia, 24–28 May 2010.
- [17] A. Mohsen M., M. Soryani, K. Navi, M. Tehrani (Eds.), “A novel ternary-to-binary converter in quantum-dot cellular automata”, Vol. 1 of 1, 2012 IEEE Computer Society Annual Symposium on VLSI, IEEE, Amherst, MA, USA, 19–21 Aug. 2012.
- [18] S. Aloke, P. Dipankar, “dpl-based novel binary-to-ternary converter on cmos technology”, AEU - International Journal of Electronics and Communications Vol.92 (1) (August 2018) 69–73.
- [19] M. Suzuk, N. Ohkubo, T. Shinbo, T. Yamanaka, K. Shimizu, Y. Nakagome (Eds.), “A 1.5 ns 32 b CMOS ALU in double pass-transistor logic”, Vol. 1 of 1, 1993 IEEE International Solid-State Circuits Conference Digest of Technical Papers, IEEE, San Francisco, CA, USA, 24–26 Feb. 1993.
- [20] S. Aloke, D. Pal, M. Chandra, “benchmarking of dpl-based 8b  $\times$  8b novel wave-pipelined multiplier”, International Journal of Electronics Letters Vol.5 (1) (2017) 115–128.
- [21] E. Danial, I. Michel, “implementation of ternary circuits with binary integrated circuits”, IEEE Transactions on Computers Vol.26 (12) (1977) 291 – 300.
