# Supplementary material for: Multiple-Valued Logic Circuit Design and Data Transmission Intended for Embedded Systems
Source: arXiv:2211.04542 source file (2022-11-08)
Supplement: Supplementary file 6 [file High-Performance.pdf]

Received May 14, 2019, accepted July 2, 2019, date of publication July 11, 2019, date of current version July 30, 2019.

Digital Object Identifier 10.1109/ACCESS.2019.2928251

# High-Performance and Energy-Efficient CNFET-Based Designs for Ternary Logic Circuits

**RAMZI A. JABER**<sup>1</sup>, (Student Member, IEEE), **ABDALLAH KASSEM**<sup>2</sup>, (Senior Member, IEEE), **AHMAD M. EL-HAJJ**<sup>1</sup>, (Member, IEEE), **LINA A. EL-NIMRI**<sup>3</sup>, AND **ALI MASSOUD HAIDAR**<sup>1</sup>

<sup>1</sup>Department of Computer and Electrical Engineering, Beirut Arab University, Beirut 11072809, Lebanon

<sup>2</sup>Department of Electrical and Computer Engineering, Notre Dame University-Louaize, Zouk Mikael, Lebanon

<sup>3</sup>Department of Business Computer, Lebanese University, Beirut, Lebanon

Corresponding author: Ramzi A. Jaber (r.jaber@bau.edu.lb)

**ABSTRACT** Recently, the demand for portable electronics and embedded systems has increased. These devices need low-power circuit designs because they depend on batteries as an energy resource. Moreover, multi-valued logic (MVL) circuits provide notable improvements over binary circuits in terms of interconnect complexity, chip area, propagation delay, and energy consumption. Therefore, this paper proposes new ternary circuits aiming to lower the power delay product (PDP) to save battery consumption. The proposed designs include new ternary gates [standard ternary inverter (STI) and ternary nand (TNAND)] and combinational circuits [ternary decoder (TDecoder), ternary half-adder (THA), and ternary multiplier (TMUL)] using carbon nano-tube field-effect transistors (CNFETs). This paper employs the best trade-off between reducing the number of used transistors, utilizing energy-efficient transistor arrangement such as transmission gate, and applying the dual supply voltages ( $V_{dd}$  and  $V_{dd}/2$ ). The five proposed designs are compared with the latest 15 ternary circuits using the HSPICE simulator for different supply voltages, different temperatures, and different frequencies; 180 simulations are performed to prove the efficiency of the proposed designs. The results show the advantage of the proposed designs in reduction over 43% in terms of transistors' count for the ternary decoder and over 88%, 99%, 98%, 86%, and 78% in energy consumption (PDP) for the STI, TNAND, TDecoder, THA, and TMUL, respectively.

**INDEX TERMS** Carbon nano-tube field effect transistors (CNFET), ternary combinational circuits, ternary logic gates, multi-valued logic (MVL), power delay product.

## I. INTRODUCTION

The limitation in the binary circuit is due to a large number of connections thus requiring a big chip area and a notable increase in energy consumption. Whereas, Multi-Valued Logic (MVL) system has more than two-valued logic to lower interconnections, chip area of up to 70% [1], and energy consumption by more than 50% [2]. Moreover, the authors of [3] has proved mathematically that ternary logic is the most efficient in circuit complexity and cost compared to other bases. Ternary logic systems can be represented in two ways: balanced ternary logic ( $-1, 0, 1$ ) corresponding to

( $-V_{dd}, 0, V_{dd}$ ), and standard (unbalanced) ternary logic ( $0, 1, 2$ ) corresponding to ( $0, V_{dd}/2, V_{dd}$ ).

For the past decade, MVL has attracted researchers' attention over binary logic. MVL can be implemented in software (algorithm) and circuit design such as logic gates, combinational circuits, memory circuits, programmable logic arrays (PLAs), MV-Quantum Logic, and wireless sensor networks [4]–[10].

Different transistor technologies have been used such as CMOS [11], FinFet [12], and CNFET [13]–[18]. Among the mentioned techniques, CNFET provides the best trade-off in terms of energy efficiency and circuit speed [19].

Therefore, this paper uses CNFET technology in the design of the ternary circuits. The proposed designs will compare to the latest CNFET-based designs in [13]–[18], which are

The associate editor coordinating the review of this manuscript and approving it for publication was Bora Onat.

known to provide efficient circuit designs in terms of transistor count, power and PDP. In particular, [13] presents the *STI*, *TNAND*, *TNOR*, *TDecoder*, *THA*, and *TMUL* using CNFET. In [14] and [17], a ternary decoder design described in replacing the *TNOR* with a binary *NOR*. In [15], [16], [18], improved circuit designs for the *STI*, *TNAND*, *THA*, and *TMUL*, are presented.

This paper proposes new designs for the *STI*, *TNAND*, *TDecoder*, *THA*, and *TMUL* by reducing the number of used transistors, utilizing energy-efficient transistor arrangement such as transmission gate and applying the dual supply voltages  $V_{dd}$  (0.9 V), and  $V_{dd}/2$  (0.45 V) from the same power supply [18].

The new designs provide a considerable gain in terms of system performance which they have the lowest PDP compared to the designs in [13]–[18] as demonstrated in the HSPICE-based simulation results. Therefore, the proposed circuits can be implemented in low-power portable electronics and embedded systems to save battery consumption.

The rest of the paper is organized as follows: Section II provides a background of CNFETs and existing ternary logic gates, while the proposed new ternary logic gates are described in section III, and the proposed combinational circuits in section IV. Simulation results and comparisons are discussed in section V followed by the Conclusion.

## II. BACKGROUND

### A. CNFET DESIGN

Full details about the Stanford CNFET model found at [20]–[22], but it is worth mentioning that the CNFETs use a semiconducting single-walled CNT as a channel for conduction with high drive current  $35 \mu\text{A}$  when the supply voltage  $V_{dd}$  is equal to 0.9 V. The improvement of intrinsic CNFET over bulk MOSFET device is about 13 times better. The angle of atom arrangement along the tube in a single-walled CNT (SWCNT) is chirality vector which is represented by the integer pair  $(n, m)$ . This chirality vector determines if the CNT is metallic or semiconducting; if  $n = m$  or  $n - m = 3j$ , where  $j$  is an integer, then the nanotube is metallic else it is semiconducting. The CNFET diameter can be calculated from the equation in (1):

$$D_{\text{cnt}} = \frac{\sqrt{3} \cdot a_0}{\pi} \sqrt{n^2 + m^2 + nm} \quad (1)$$

where  $a_0 = 0.142 \text{ nm}$  is the inter-atomic distance between each carbon atom and its neighbor, and the integer pair  $(n, m)$  represents the chirality vector. The characteristics of the CNFET model are similar to traditional MOSFETs. Except for the threshold voltage which is calculated by the following equation (2):

$$V_{\text{th}} = \frac{E_g}{2 \cdot e} = \frac{\sqrt{3}}{3} \frac{a \cdot V\pi}{e \cdot D_{\text{cnt}}} \quad (2)$$

where  $a = 2.49 \text{ \AA}$  is the carbon to carbon atom distance,  $V\pi = 3.033 \text{ eV}$  is the carbon bond energy in the tight binding

**TABLE 1.** The relation between the chirality, diameter, and threshold voltage.

| Chirality | CNT diameter | Threshold voltage |          |
|-----------|--------------|-------------------|----------|
|           |              | N-CNFET           | P-CNFET  |
| (19,0)    | 1.487nm      | 0.289V            | - 0.289V |
| (13,0)    | 1.018nm      | 0.428V            | - 0.428V |
| (10,0)    | 0.783nm      | 0.559V            | - 0.559V |

**TABLE 2.** The truth table for the three ternary inverters.

| Ternary Input    | STI | NTI | PTI |
|------------------|-----|-----|-----|
| Logic 0 (0 V)    | 2   | 2   | 2   |
| Logic 1 (0.45 V) | 1   | 0   | 2   |
| Logic 2 (0.9 V)  | 0   | 0   | 0   |

**TABLE 3.** The truth table for Two-inputs *TNAND* and *TNOR* logic gates.

| Input |   | Output |      |
|-------|---|--------|------|
| A     | B | TNAND  | TNOR |
| 0     | 0 | 2      | 2    |
| 0     | 1 | 2      | 1    |
| 0     | 2 | 2      | 0    |
| 1     | 0 | 2      | 1    |
| 1     | 1 | 1      | 1    |
| 1     | 2 | 1      | 0    |
| 2     | 0 | 2      | 0    |
| 2     | 1 | 1      | 0    |
| 2     | 2 | 0      | 0    |

model,  $e$  is the electron charge unit, and  $D_{\text{cnt}}$  is the CNT diameter.

In general, three chiralities can be used in the ternary logic design. Table 1 shows the relationship between the chirality, diameter, and threshold voltage.

### B. EXISTING TERNARY LOGIC GATES

The basic ternary logic gates are *NOT*, *AND*, *OR*, *NAND* and *NOR*.  $A_i$  and  $B_j$  are the ternary inputs where  $i$  and  $j \in \{0, 1, 2\}$ . The ternary equations of the basic ternary logic gates are presented in (3):

$$\begin{aligned} \text{NOT: } \overline{A_i} &= 2 - A_i, \\ \text{AND: } A_i \cdot B_j &= \min\{A_i, B_j\}, \\ \text{OR: } A_i + B_j &= \max\{A_i, B_j\}, \\ \text{NAND: } \overline{A_i \cdot B_j} &= \overline{\min\{A_i, B_j\}}, \\ \text{NOR: } \overline{A_i + B_j} &= \overline{\max\{A_i, B_j\}}, \end{aligned} \quad (3)$$

In [13], the authors present three types of ternary inverters, *TNAND*, and *TNOR* logic gate using CNFET.

**TABLE 4.** The disadvantage of existing logic gates in [13], [16], and [18] and the advantage of proposed logic gates.

| Disadvantage                                                                                                                           | Advantage                                                                                         |
|----------------------------------------------------------------------------------------------------------------------------------------|---------------------------------------------------------------------------------------------------|
| Shown in Fig. 15 and 16 in the appendix<br>The existing designs suffer from<br>High power consumption due to:                          | Shown in Fig. 1 and 2<br>The proposed designs provide<br>Low power consumption due to:            |
| 1- Two transistors that act as resistors in <i>STI</i> (T2, T3) and in <i>TNAND</i> (T5, T6) [13].                                     | Eliminating these two transistors by applying dual supply voltages ( $V_{dd}$ and $V_{dd}/2$ ).   |
| 2- Two transistors that act as resistors in <i>STI</i> (T3, T6) and in <i>TNAND</i> (T5, T10) [16].                                    |                                                                                                   |
| 3- Two transistors that are always active in <i>STI</i> (T2, T3) and in <i>TNAND</i> (T5, T6) [18].                                    |                                                                                                   |
| 4- For <i>STI</i> [13], [18]: Four transistors (T1, T2, T3, T4) in series must be active to get logic 1.                               | For the proposed <i>STI</i> : Only one transistor (T3) must be active to get logic 1.             |
| 5- For <i>STI</i> [16]: Four transistors (T1, T3, T6, T5) in series must be active to get logic 1.                                     |                                                                                                   |
| 6- For <i>TNAND</i> [13], [18]: Five or Six transistors [(T1 or T2) or both, T5, T6, T7, T8)] in series must be active to get logic 1. | For the proposed <i>TNAND</i> : Two transistors (T5, T6) in series must be active to get logic 1. |
| 7- For <i>TNAND</i> [16]: Five or Six transistors [(T1 or T2) or both, T5, T10, T8, T9)] in series must be active to get logic 1.      |                                                                                                   |

The first inverter is a standard ternary inverter (*STI*), the second is a negative ternary inverter (*NTI*), and the third one is a positive ternary inverter (*PTI*). Table 2 shows the truth table for the three ternary inverters.

Table 3 shows the truth table for Two-inputs *TNAND* and *TNOR* logic gates.

### III. PROPOSED TERNARY LOGIC GATES

The existing *STI* and *TNAND* logic gates designs in [13], [16], and [18] are shown in Fig. 15 and 16 in the appendix.

This section proposes new designs of *STI* and *TNAND* logic gates as shown in Fig. 1 and Fig. 2.

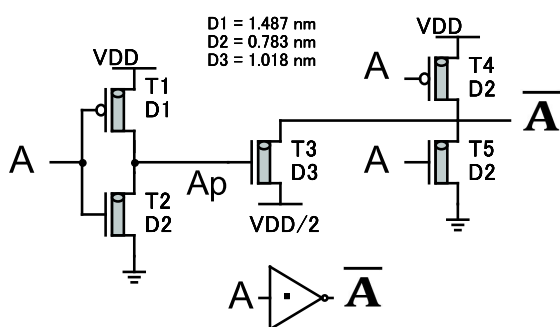**FIGURE 1.** Transistor level of the proposed *STI*.

Table 4 shows the disadvantage of the existing *STI* and *TNAND* in [13], [16], and [18] and the advantage of the proposed ternary logic gates.

#### A. PROPOSED STANDARD TERNARY INVERTER

Fig. 1 shows the transistor level design of the proposed *STI* where the chirality, diameter, and threshold voltage ( $V_{th}$ ) of the CNFETs used are shown in Table 5.

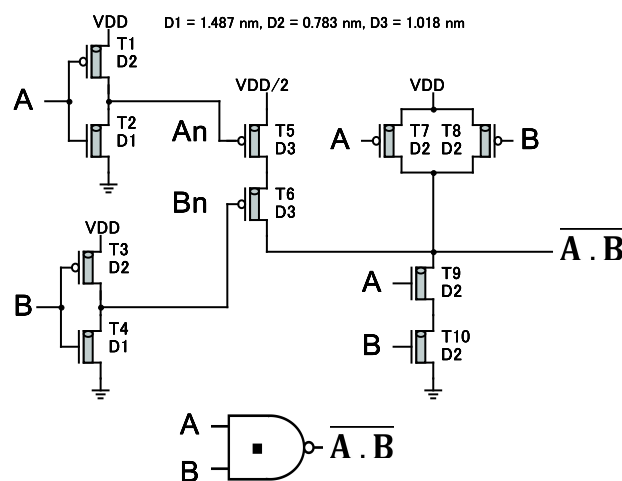**FIGURE 2.** Transistor level of the proposed *TNAND*.**TABLE 5.** The chirality, diameter, and threshold voltage of the CNTs used in the proposed *STI*.

| CNFET Type      | Chirality | Diameter | $V_{th}$ |
|-----------------|-----------|----------|----------|
| P-CNFET (T4)    | (10, 0)   | 0.783nm  | - 0.559V |
| P-CNFET (T1)    | (19, 0)   | 1.487nm  | - 0.289V |
| N-CNFET (T2,T5) | (10, 0)   | 0.783nm  | 0.559V   |
| N-CNFET (T3)    | (13, 0)   | 1.018nm  | 0.428V   |

Table 6 shows the detailed operation of the proposed *STI* circuit of Fig. 1.

When the input  $A$  is logic 0, then transistors (T1, and T4) are turned ON and (T2, and T5) are turned OFF. The output  $A_p$  is equal to logic 2, then transistor (T3) is turned ON. Therefore, the output  $\bar{A}$  is equal to logic 2.

**TABLE 6.** The detailed operation of *STI* of Fig. 1.

| Ternary Input <i>A</i> | 0 (0 V) | 1 (0.45 V) | 2 (0.9 V) |
|------------------------|---------|------------|-----------|
| P-CNFET T1             | ON      | ON         | OFF       |
| N-CNFET T2             | OFF     | OFF        | ON        |
| $A_p$                  | 2       | 2          | 0         |
| N-CNFET T3             | ON      | ON         | OFF       |
| P-CNFET T4             | ON      | OFF        | OFF       |
| N-CNFET T5             | OFF     | OFF        | ON        |
| Output $\bar{A}$       | 2       | 1          | 0         |

When the input *A* is logic 1, then transistor (T1) is turned ON, and (T2, T4, and T5) are turned OFF. The output  $A_p$  is equal to logic 2, then transistor (T3) is turned ON. Therefore, the output  $\bar{A}$  is equal to logic 1.

Finally, when the input *A* is logic 2, then transistors (T2, and T5) are turned ON and (T1, and T4) are turned OFF. The output  $A_p$  is equal to logic 0, then transistor (T3) is turned OFF. Therefore, the output  $\bar{A}$  is equal to logic 0.

### B. PROPOSED TERNARY NAND

Fig. 2 shows the transistor level design of the proposed two inputs *TNAND* where the chirality, diameter, and threshold voltage (*V<sub>th</sub>*) of the CNFETs used are shown in Table 7.

**TABLE 7.** The chirality, diameter, and threshold voltage of the CNTs used in the proposed *TNAND*.

| CNFET Type            | Chirality | Diameter | <i>V<sub>th</sub></i> |
|-----------------------|-----------|----------|-----------------------|
| P-CNFET (T1,T3,T7,T8) | (10, 0)   | 0.783nm  | - 0.559V              |
| P-CNFET (T5, T6)      | (13, 0)   | 1.018nm  | - 0.428V              |
| N-CNFET (T9, T10)     | (10, 0)   | 0.783nm  | 0.559V                |
| N-CNFET (T2, T4)      | (19, 0)   | 1.487nm  | 0.289V                |

Table 8 shows the selected combinations of two ternary inputs *A* and *B* to describe the operation of the proposed *TNAND* logic gate circuit of Fig. 2.

When the inputs (*A*, *B*) are (0 V, 0 V), then transistors (T1, T3, T7, and T8) are turned ON and (T2, T4, T9, and T10) are turned OFF. The outputs ( $A_n$ ,  $B_n$ ) are equal to (0.9 V, 0.9 V), then transistors (T5, and T6) are turned OFF. Therefore, the output is equal to 0.9 V.

When the inputs (*A*, *B*) are (0 V, 0.45 V), then transistors (T1, T4, and T7) are turned ON and (T2, T3, T8, T9, and T10) are turned OFF. The outputs ( $A_n$ ,  $B_n$ ) are equal to (0.9 V, 0 V), then transistor (T6) is turned ON and (T5) is turned OFF. Therefore, the output is equal to 0.9 V.

When the inputs (*A*, *B*) are (0.45 V, 0.45 V), then transistors (T2, and T4) are turned ON and (T1, T3, T7, T8, T9, and T10) are turned OFF. The outputs ( $A_n$ ,  $B_n$ ) are equal to (0 V, 0 V), then transistors (T5, and T6) are turned ON. Therefore, the output is equal to 0.45 V.

**TABLE 8.** The detailed operation of *TNAND* with selected inputs of Fig. 2.

| Ternary Inputs ( <i>A</i> , <i>B</i> ) | (0, 0) | (0, 1) | (1, 1) | (1, 2) |
|----------------------------------------|--------|--------|--------|--------|
| P-CNFET T1                             | ON     | ON     | OFF    | OFF    |
| N-CNFET T2                             | OFF    | OFF    | ON     | ON     |
| $A_n$                                  | 2      | 2      | 0      | 0      |
| P-CNFET T3                             | ON     | OFF    | OFF    | OFF    |
| N-CNFET T4                             | OFF    | ON     | ON     | ON     |
| $B_n$                                  | 2      | 0      | 0      | 0      |
| P-CNFET T5                             | OFF    | OFF    | ON     | ON     |
| P-CNFET T6                             | OFF    | ON     | ON     | ON     |
| P-CNFET T7                             | ON     | ON     | OFF    | OFF    |
| P-CNFET T8                             | ON     | OFF    | OFF    | OFF    |
| N-CNFET T9                             | OFF    | OFF    | OFF    | OFF    |
| N-CNFET T10                            | OFF    | OFF    | OFF    | ON     |
| Output <i>TNAND</i>                    | 2      | 2      | 1      | 1      |

Finally, when the inputs (*A*, *B*) are (0.45 V, 0.9 V), then transistors (T2, T4, and T10) are turned ON and (T1, T3, T7, T8, and T9) are turned OFF. The outputs ( $A_n$ ,  $B_n$ ) are equal to (0 V, 0 V), then transistors (T5, and T6) are turned ON. Therefore, the output is equal to 0.45 V.

## IV. PROPOSED COMBINATIONAL CIRCUITS

This section proposes some of the combinational circuits such as *TDecoder*, *THA*, and *TMUL*.

### A. PROPOSED TERNARY DECODER

The ternary decoder converts *n* trits information inputs to a maximum  $3^n$  unique outputs. It is used in many applications such as the ternary adder, ternary multiplier, ternary memory, and others.

Ternary decoder with one ternary input (*X*), and three binary outputs ( $X_0$ ,  $X_1$ ,  $X_2$ ) are described mathematically in equation (4) and its truth table is shown in Table 10.

$$X_{k,k \in \{0,1,2\}} = \begin{cases} 2, & \text{if } x = k \\ 0, & \text{if } x \neq k \end{cases} \quad (4)$$

The existing *TDecoders* in [13], [14], and [17] are shown in Fig. 17 in the appendix with 16, 10, and 11 transistors respectively.

This section proposes a new design of *TDecoder* with 9 transistors through replacing the *TNOR* and the second *NTI* with a novel sub-circuit and a binary inverter respectively as represented in Fig. 3.

Fig. 3 shows the transistor level design of the proposed *TDecoder*. It consists of one negative ternary inverter (NTI), one positive ternary inverter (PTI), one binary inverter, and a novel sub-circuit.

Table 9 shows the disadvantage of the existing *TDecoder* in [13], [14], and [17] and the advantage of the proposed *TDecoder*.

**TABLE 9.** The disadvantage of existing *TDecoder* in [13], [14], and [17] and the advantage of proposed *TDecoder*.

| Disadvantage                                                                                              | Advantage                                                                                                                                                                 |
|-----------------------------------------------------------------------------------------------------------|---------------------------------------------------------------------------------------------------------------------------------------------------------------------------|
| Shown in in Fig. 17 in the appendix<br>The existing design suffers from<br>High power consumption due to: | Shown in Fig. 3<br>The proposed design provides<br>Low power consumption due to:                                                                                          |
| 1- The Transistors' count of [13], [14], [17] equal to 16, 10, 11 respectively.                           | Transistors' count = 9.                                                                                                                                                   |
| 2- To get $X_1$ , [13] uses the Ternary <i>NOR</i> (10 transistors).                                      | To get $X_1$ , the design uses the novel sub-circuit (3 transistors) including the Transmission Gate (T7, T8) which provides low power consumption and propagation delay. |
| 3- To get $X_1$ , [14], [17] use the Binary <i>NOR</i> (4 transistors).                                   | Only the Transmission Gate (T7, T8) must be active to get logic $X_1$ equals to logic 2.                                                                                  |
| 4- Six transistors (T11, T12, T13, T14, T15, T16) must be active to get $X_1$ equals to logic 2 [13].     |                                                                                                                                                                           |
| 5- Two transistors (T9, T10) in series must be active to get logic $X_1$ equals to logic 2 [14], [17].    |                                                                                                                                                                           |

**TABLE 10.** Ternary decoder truth table.

| Input | Outputs |       |       |
|-------|---------|-------|-------|
| X     | $X_2$   | $X_1$ | $X_0$ |
| 0     | 0       | 0     | 2     |
| 1     | 0       | 2     | 0     |
| 2     | 2       | 0     | 0     |

**TABLE 11.** The chirality, diameter, and threshold voltage of the CNTs used in the proposed *TDecoder*.

| CNFET Type           | Chirality | Diameter | Vth      |
|----------------------|-----------|----------|----------|
| P-CNFET (T1, T5)     | (10, 0)   | 0.783nm  | - 0.559V |
| P-CNFET (T3, T8)     | (19, 0)   | 1.487nm  | - 0.289V |
| N-CNFET (T4, T6, T9) | (10, 0)   | 0.783nm  | 0.559V   |
| N-CNFET (T2, T7)     | (19, 0)   | 1.487nm  | 0.289V   |

**TABLE 12.** The detailed operation of the proposed *TDecoder* of Fig. 3.

| Ternary Input X                | 0 (0 V)  | 1 (0.45 V) | 2 (0.9 V)  |
|--------------------------------|----------|------------|------------|
| P-CNFET T1                     | ON       | OFF        | OFF        |
| N-CNFET T2                     | OFF      | ON         | ON         |
| <b>Output <math>X_0</math></b> | <b>2</b> | <b>0</b>   | <b>0</b>   |
| P-CNFET T3                     | ON       | ON         | OFF        |
| N-CNFET T4                     | OFF      | OFF        | ON         |
| <b>Intermediate Y</b>          | <b>2</b> | <b>2</b>   | <b>0</b>   |
| P-CNFET T5                     | OFF      | OFF        | ON         |
| N-CNFET T6                     | ON       | ON         | OFF        |
| <b>Output <math>X_2</math></b> | <b>0</b> | <b>0</b>   | <b>2</b>   |
| N-CNFET T7                     | OFF      | ON         | ON         |
| P-CNFET T8                     | OFF      | ON         | ON         |
| N-CNFET T9                     | ON       | OFF        | OFF        |
| <b>Output <math>X_1</math></b> | <b>0</b> | <b>Y=2</b> | <b>Y=0</b> |

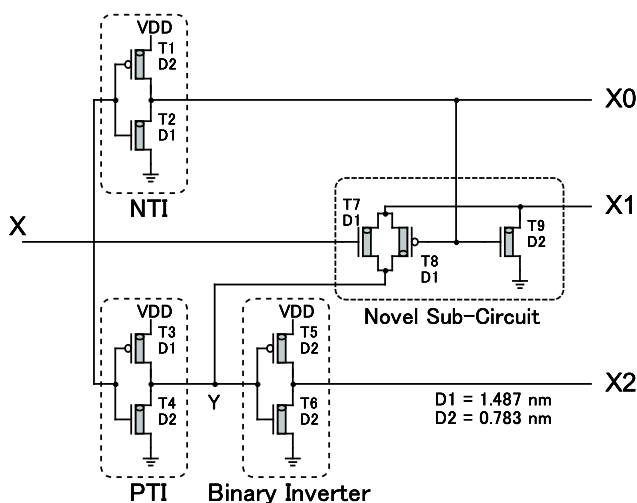**FIGURE 3.** Transistor level of the proposed *TDecoder* with 9 CNFETs.

The chirality, diameter, and threshold voltage ( $V_{th}$ ) of the CNFETs used are shown in Table 11, and the detailed operation of the proposed circuit described in Table 12.

When the input  $X$  is logic 0, then transistors (T1, and T3) are turned ON and (T2, T4, and T7) are turned OFF. The output  $X_0$  and the intermediate  $Y$  are equal to logic 2. Then (T5, and T8) are turned OFF and (T6, and T9) are turned ON. Therefore, the outputs  $X_1$  and  $X_2$  are equal to logic 0.

When the input  $X$  is logic 1, then transistors (T2, T3, and T7) are turned ON and (T1, and T4) are turned OFF.

The output  $X_0$  is equal to logic 0, and the intermediate  $Y$  is equal to logic 2. Then (T5, and T9) are turned OFF and (T6, and T8) are turned ON. Therefore, the output  $X_1$  is equal to the value of  $Y$  which is logic 2 and the output  $X_2$  is equal to logic 0.

Finally, when the input  $X$  is logic 2, then transistors (T2, T4, and T7) are turned ON and (T1, and T3) are turned OFF. The output  $X_0$  and the intermediate  $Y$  are equal to logic 0. Then (T6, and T9) are turned OFF and (T5, and T8)



**TABLE 13.** Karnaugh Map of *THA*.

| Sum                       |                           |                           |                           |
|---------------------------|---------------------------|---------------------------|---------------------------|
| <i>A/B</i>                | <i>B</i> <sub>0</sub> (0) | <i>B</i> <sub>1</sub> (1) | <i>B</i> <sub>2</sub> (2) |
| <i>A</i> <sub>0</sub> (0) | 0                         | 1                         | 2                         |
| <i>A</i> <sub>1</sub> (1) | 1                         | 2                         | 0                         |
| <i>A</i> <sub>2</sub> (2) | 2                         | 0                         | 1                         |

  

| Carry                     |                           |                           |                           |
|---------------------------|---------------------------|---------------------------|---------------------------|
| <i>A/B</i>                | <i>B</i> <sub>0</sub> (0) | <i>B</i> <sub>1</sub> (1) | <i>B</i> <sub>2</sub> (2) |
| <i>A</i> <sub>0</sub> (0) | 0                         | 0                         | 0                         |
| <i>A</i> <sub>1</sub> (1) | 0                         | 0                         | 1                         |
| <i>A</i> <sub>2</sub> (2) | 0                         | 1                         | 1                         |

are turned ON. Therefore, the output  $X_1$  is equal to the value of  $Y$  which is logic 0, and the output  $X_2$  is equal to logic 2.

### B. PROPOSED TERNARY HALF ADDER

Ternary half adder (*THA*) is able to add two ternary inputs and provides two outputs: the Sum and the Carry. Table 13 shows the Karnaugh map of *THA*. The equations of sum and carry derived from Table 13 are (5) and (6) as follow:

$$\text{Sum} = 2 \cdot (A_0B_2 + A_1B_1 + A_2B_0) + 1 \cdot (A_0B_1 + A_1B_0 + A_2B_2) \quad (5)$$

$$\text{Carry} = 1 \cdot (A_1B_2 + A_2B_1 + A_2B_2) \quad (6)$$

where  $A_k$  and  $B_k$ , are the outputs of the *TDecoder* from inputs  $A$  and  $B$  respectively.

The existing *THA* in [13], [15], and [16] are shown in Fig. 18 in the appendix with 136, 112, and 112 transistors respectively.

This section proposes a new design of *THA* with 85 transistors using De Morgan's Law and dual power supply ( $V_{dd}$  and  $V_{dd}/2$ ) to eliminate the encoder level shifter in [13], [15]. Also, it uses the proposed *TDecoder* of Fig. 3, the proposed *STI* of Fig. 1 and the proposed *TNAND* of Fig. 2, and removes one common *NAND* as illustrate in Fig. 4.

Fig. 4 shows the proposed *THA*. It consists of two proposed *TDecoders*, eight 2-inputs binary *NAND*, three 3-inputs binary *NAND*, one binary inverter, one proposed *TNAND*, and one proposed *STI*.

Table 14 shows the total transistors' count of the proposed *THA*.

The operation of the proposed *THA*: Two ternary inputs  $A$  and  $B$  fed to the proposed *TDecoder* and produce outputs as ( $A_2, A_1, A_0$ ) and ( $B_2, B_1, B_0$ ). These outputs will drive the eight 2-inputs binary *NAND*, the three 3-inputs binary *NAND* logic gates, the proposed *STI*, binary inverter, and the proposed *TNAND* to get the Sum and the Carry as final outputs.

### C. PROPOSED TERNARY MULTIPLIER

Ternary multiplier (*TMUL*) is able to multiply two ternary inputs and provides two outputs: the Product and the Carry. Table 15 shows the Karnaugh map of *TMUL*. The equations

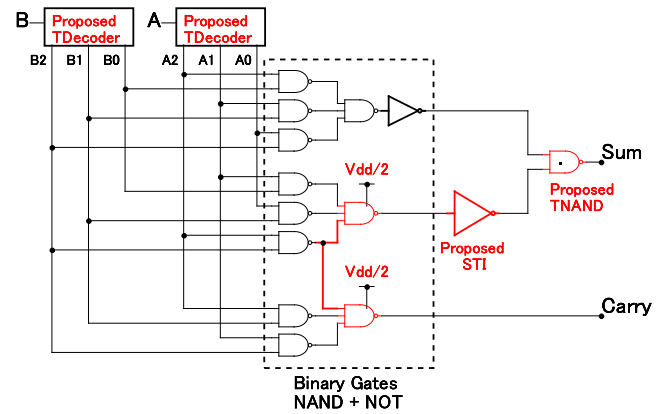**FIGURE 4.** Proposed *THA* with 85 transistors.**TABLE 14.** Total transistors' count of the proposed *THA*.

|                          | No. of Devices | No. of Transistors | Subtotal* |
|--------------------------|----------------|--------------------|-----------|
| Proposed <i>TDecoder</i> | 2              | 9                  | 18        |
| Binary 2- <i>NAND</i>    | 8              | 4                  | 32        |
| Binary 3- <i>NAND</i>    | 3              | 6                  | 18        |
| Binary Inverter          | 1              | 2                  | 2         |
| Proposed <i>STI</i>      | 1              | 5                  | 5         |
| Proposed <i>TNAND</i>    | 1              | 10                 | 10        |
| Total                    |                |                    | 85        |

\*Subtotal = No. of Devices x No. of Transistors

**TABLE 15.** Karnaugh Map of *TMUL*.

| Product                   |                           |                           |                           |
|---------------------------|---------------------------|---------------------------|---------------------------|
| <i>A/B</i>                | <i>B</i> <sub>0</sub> (0) | <i>B</i> <sub>1</sub> (1) | <i>B</i> <sub>2</sub> (2) |
| <i>A</i> <sub>0</sub> (0) | 0                         | 0                         | 0                         |
| <i>A</i> <sub>1</sub> (1) | 0                         | 1                         | 2                         |
| <i>A</i> <sub>2</sub> (2) | 0                         | 2                         | 1                         |

  

| Carry                     |                           |                           |                           |
|---------------------------|---------------------------|---------------------------|---------------------------|
| <i>A/B</i>                | <i>B</i> <sub>0</sub> (0) | <i>B</i> <sub>1</sub> (1) | <i>B</i> <sub>2</sub> (2) |
| <i>A</i> <sub>0</sub> (0) | 0                         | 0                         | 0                         |
| <i>A</i> <sub>1</sub> (1) | 0                         | 0                         | 0                         |
| <i>A</i> <sub>2</sub> (2) | 0                         | 0                         | 1                         |

of Product and Carry derived from Table 15 are (7) and (8) as follow:

$$\text{Product} = 2 \cdot (A_1B_2 + A_2B_1) + 1 \cdot (A_1B_1 + A_2B_2) \quad (7)$$

$$\text{Carry} = 1 \cdot A_2B_2 \quad (8)$$

where  $A_k$  and  $B_k$ , are the outputs of the *TDecoder* from inputs  $A$  and  $B$  respectively.

The existing *TMUL* in [13], [15], and [16] are shown in Fig. 19 in the appendix with 100, 86, and 76 transistors respectively.

This section proposes a new design of *TMUL* with 61 transistors using De Morgan's Law and the dual power supply ( $V_{dd}$  and  $V_{dd}/2$ ) to eliminate the encoder level shifter in

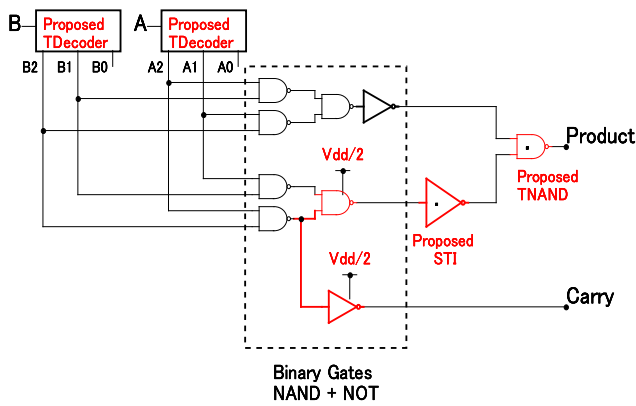

FIGURE 5. Proposed *TMUL* with 61 transistors.

[13], [15]. Also, it uses the proposed *TDecoder* of Fig. 3, the proposed *STI* of Fig. 1 and the proposed *NAND* of Fig. 2, and removes one common *NAND* as illustrate in Fig. 5.

Fig. 5 shows the proposed *TMUL*. It consists of two proposed *TDecoders*, six binary *NAND*, two binary inverters, one proposed *STI*, and one proposed *TNAND*.

TABLE 16. Total transistors' count of the proposed *TMUL*.

|                          | No. of<br>Devices | No. of<br>Transistors | Subtotal* |
|--------------------------|-------------------|-----------------------|-----------|
| Proposed <i>TDecoder</i> | 2                 | 9                     | 18        |
| Binary <i>NAND</i>       | 6                 | 4                     | 24        |
| Binary Inverter          | 2                 | 2                     | 4         |
| Proposed <i>STI</i>      | 1                 | 5                     | 5         |
| Proposed <i>TNAND</i>    | 1                 | 10                    | 10        |
| Total                    |                   |                       | 61        |

\*Subtotal = No. of Devices x No. of Transistors

Table 16 shows the total transistors' count of the proposed *TMUL*.

The operation of the proposed *TMUL*: Two ternary inputs *A* and *B* fed to the proposed *TDecoders* and produce outputs as ( $A_2, A_1, A_0$ ) and ( $B_2, B_1, B_0$ ). These outputs will drive the four 2-inputs binary *NAND*, the two 2-inputs binary *NAND* logic gates, the proposed *STI*, the two binary inverters, and the proposed *TNAND* to get the Product and the Carry as final outputs.

## V. SIMULATION RESULTS AND COMPARISONS

As mentioned in the Introduction that CNFET provides better energy efficiency compared to CMOS, FinFET, and other transistor technologies [19].

Therefore, the proposed *STI*, *TNAND*, *TDecoder*, *THA*, and *TMUL* are simulated and compared to CNFET-Based ternary circuits in [13]–[18].

All the twenty circuits are extensively simulated and tested using the HSPICE simulator with 32-nm channel length for different power supplies (0.8 V, 0.9 V, 1 V), different temperatures (10°C, 27°C, 70°C), and different frequencies (0.5 GHz, 1 GHz, 2 GHz).

One hundred eighty simulations are performed to study the performance and efficiency of the proposed five circuits in the separate sections below.

Although CNFET-based circuit may suffer performance changes due to device variability, this effect has not been considered in this work.

Table 17 shows some essential parameters of the CNFET model used in all the circuits with brief descriptions.

TABLE 17. Some of CNFET model parameters.

|                   | Description                                                                     | Value   |
|-------------------|---------------------------------------------------------------------------------|---------|
| $L_{ch}$          | Physical channel length                                                         | 32 nm   |
| $L_{geff}$        | The mean free path in the intrinsic CNT                                         | 100 nm  |
| $L_{ss} (L_{dd})$ | The length of doped CNT source-side (drain-side) extension region               | 10 nm   |
| $E_{fi}$          | The Fermi level of the doped S/D tube                                           | 0.6 eV  |
| $K_{gate}$        | The dielectric constant of high-k top gate dielectric material (planer gate)    | 4       |
| $T_{ox}$          | The thickness of the high-k top gate dielectric material (planer gate)          | 1 nm    |
| $C_{sub}$         | The coupling capacitance between the channel region and the substrate           | 10 pF/m |
| $C_{csd}$         | The coupling capacitance between the channel region and the source/drain region | 0 pF/m  |
| $Pitch$           | The distance between two adjacent CNTs within the same device                   | 20 nm   |
| $Tubes$           | The number of tubes in the device                                               | 1       |

All input signals have a rise and fall time of 20 ps. The propagation delay of the circuit is measured, for example, for  $t_1$  as shown in Fig. 8, when the input (*X*) is rising from 0 to 1, and the output ( $X_0$ ) is falling from 2 to 0. A similar procedure is done to get all possible rising and falling propagation delays for outputs of all studied circuits and find the maximum propagation delay for each circuit.

Then the average power consumption, maximum propagation delay, and maximum power delay product (PDP) are obtained for all circuits.

The performance of the five proposed circuits will be compared to other designs for the Power-Delay Product PDP (energy consumption).

### A. TRANSIENT ANALYSIS OF PROPOSED CIRCUITS

Fig. 6 – 10 illustrate the transient analysis of the proposed *STI*, *TNAND*, *TDecoder*, *THA*, and *TMUL* respectively.

### B. COMPARISON OF TRANSISTORS' COUNT

The minimization of transistors' count is not the only factor that affects the performance of the proposed circuits, but it is

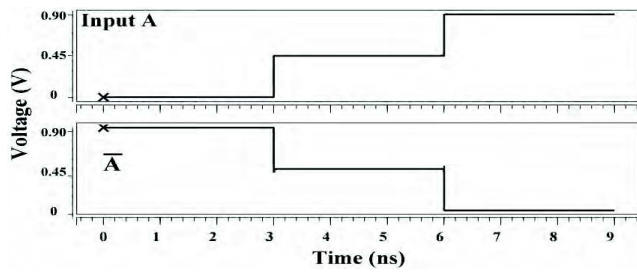FIGURE 6. Transient analysis of the proposed *STI*.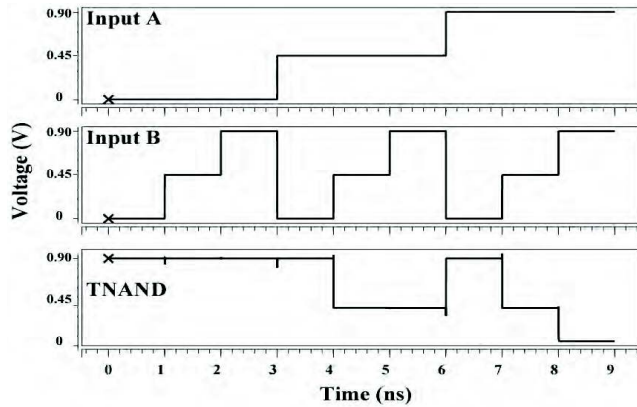FIGURE 7. Transient analysis of the proposed *TNAND*.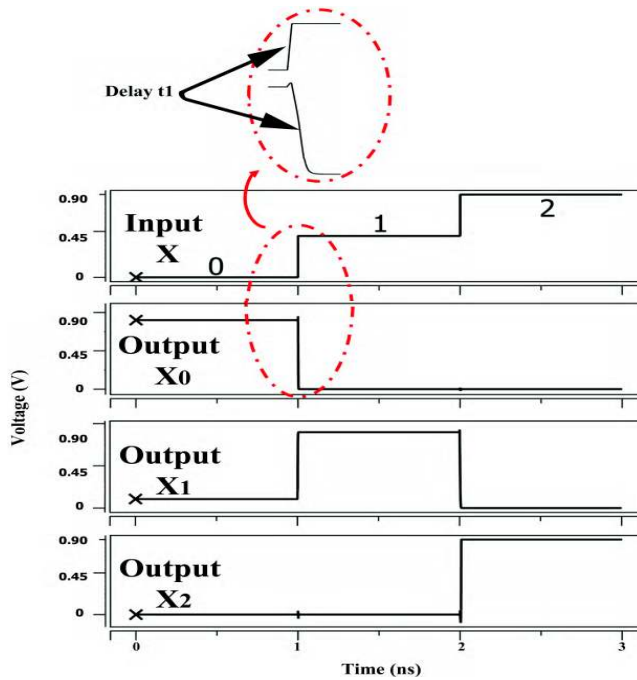FIGURE 8. Transient analysis of the proposed *TDecoder*.

a good factor. The other factors are described in the following subsections.

Table 18 shows the comparison of transistors' count for *STI*, *TNAND*, *TDecoder*, *THA*, and *TMUL* compared to [13]–[18].

This comparison of the proposed circuits demonstrates a notable reduction in transistors' count. For *STI*, around 16.67% compared to *STI* in [13], [16], and [18]. For *TNAND*,

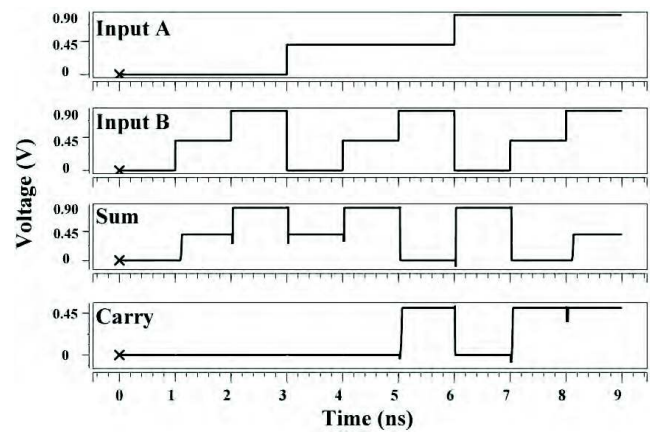FIGURE 9. Transient analysis of the proposed *THA*.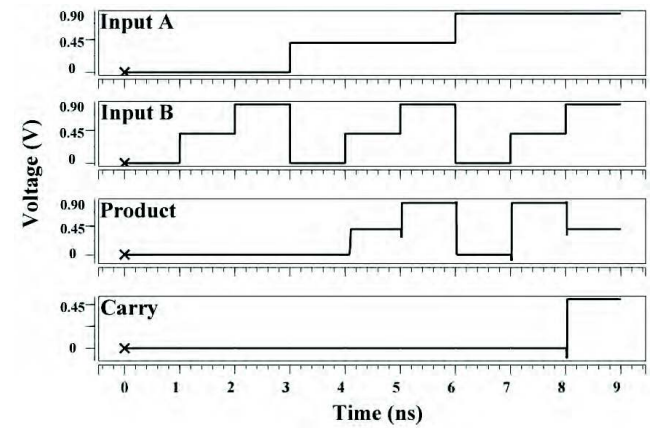FIGURE 10. Transient analysis of the proposed *TMUL*.

TABLE 18. Comparison of transistors' count of all circuits.

|                 | [13] | [16] | [15] | [18] | [17] | [14] | Proposed  |
|-----------------|------|------|------|------|------|------|-----------|
| <i>STI</i>      | 6    | 6    | –    | 6    | –    | –    | <b>5</b>  |
| <i>TNAND</i>    | 10   | 10   | –    | 10   | –    | –    | <b>10</b> |
| <i>TDecoder</i> | 16   | –    | –    | –    | 11   | 10   | <b>9</b>  |
| <i>THA</i>      | 136  | 112  | 112  | –    | –    | –    | <b>85</b> |
| <i>TMUL</i>     | 100  | 76   | 86   | –    | –    | –    | <b>61</b> |

around 0% compared to *TNAND* in [13], [16], and [18]. For *TDecoder*, around 43.75%, 10%, and 18.18% compared to *TDecoder* in [13], [14], and [17] respectively. For *THA*, around 37.5%, 24.11%, and 24.11% compared to *THA* in [13], [15], and [16] respectively. For *TMUL*, around 39%, 29.07%, and 19.74% compared to *TMUL* in [13], [15], and [16] respectively.

### C. COMPARISON OF DIFFERENT *STI* CIRCUITS

Fig. 11 shows the PDP Comparison of the investigated *STI* for (a) Different Power Supplies, (b) Different Temperatures, and (c) Different Frequencies.

#### 1) IMPACT OF DIFFERENT POWER SUPPLIES

The effect of different power supplies (0.8 V, 0.9 V, 1 V) on the performance metrics of all proposed circuits is studied.



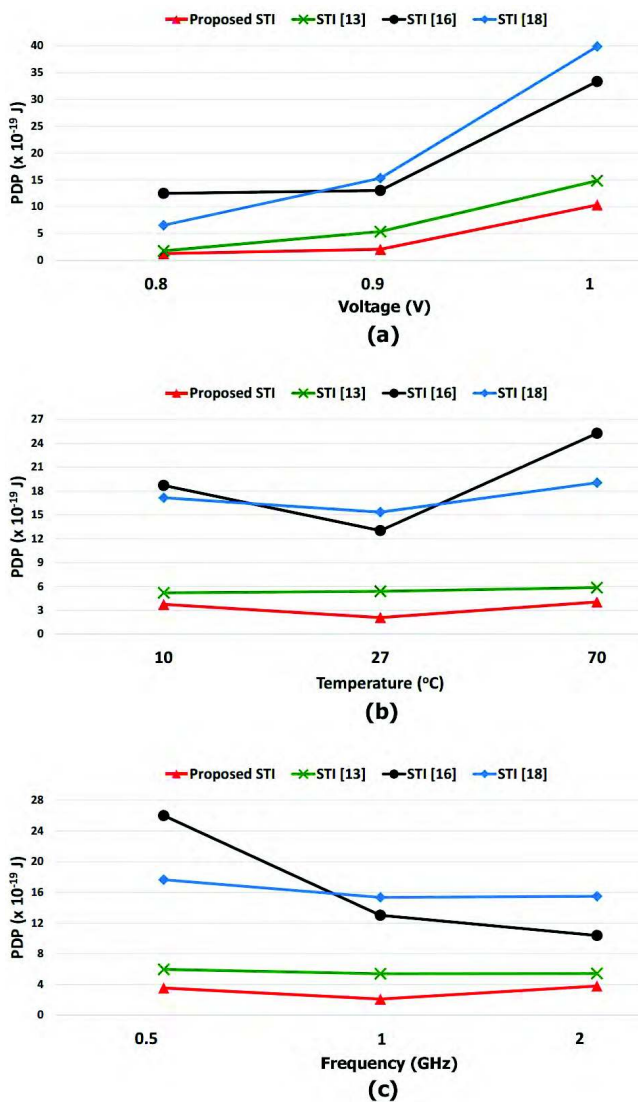

**FIGURE 11.** PDP Comparison of the investigated *STI* for: (a) different power supplies, (b) different temperatures, and (c) different frequencies.

Simulation is done at 1 GHz operating frequency and room temperature at 27°C as illustrated in Fig. 11 (a).

The comparison of the proposed *STI* demonstrates a notable reduction in PDP as shown in Fig. 11 (a). For  $V_{dd}=0.8$  V, around 28.33%, 88.68%, and 80.37% compared to [13], [16], and [18] respectively. For  $V_{dd}=0.9$  V, around 61.22%, 83.95%, and 86.38% compared to [13], [16], and [18] respectively. For  $V_{dd}=1$  V, around 30.42%, 68.98%, and 74.05% compared to [13], [16], and [18] respectively.

## 2) IMPACT OF DIFFERENT TEMPERATURES

Temperature noise is one of the most critical issues which negatively affect the performance of the circuit.

The effect of different temperatures (10°C, 27°C, 70°C) on the performance metrics of all proposed circuits is studied. Simulation is done at 1 GHz operating frequency, and power supply  $V_{dd}$  equals 0.9 V as illustrated in Fig. 11 (b).

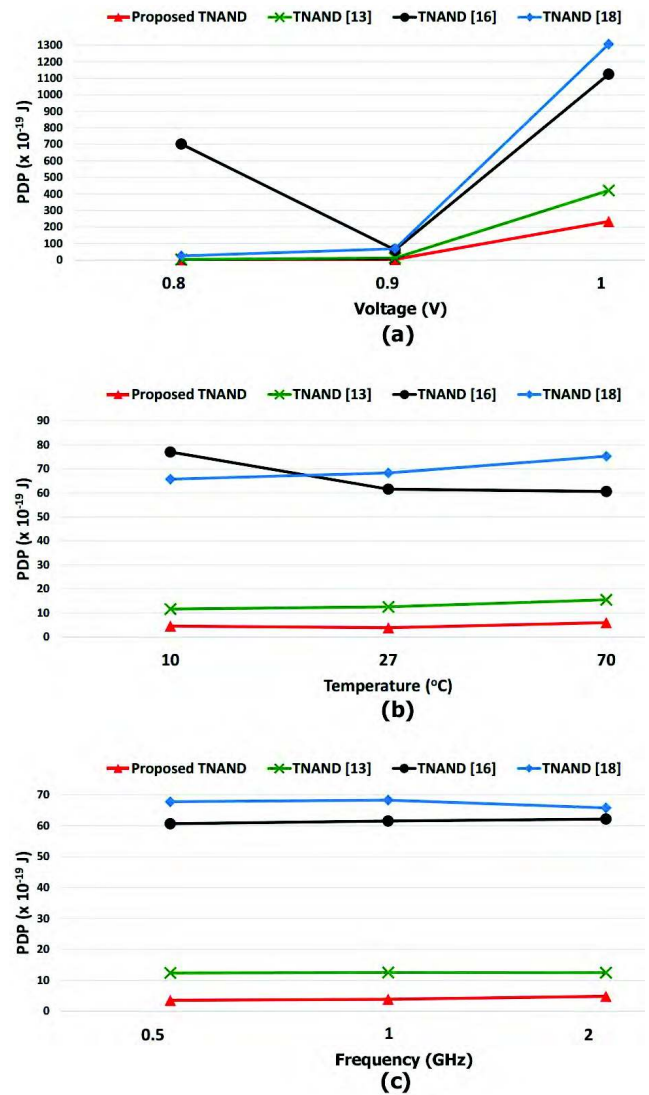

**FIGURE 12.** PDP Comparison of the investigated *TNAND* for: (a) different power supplies, (b) different temperatures, and (c) different frequencies.

The comparison of the proposed *STI* demonstrates a notable reduction in PDP as shown in Fig. 11 (b). For Temperature = 10°C, around 27.88%, 79.95%, and 78.15% compared to [13], [16], and [18] respectively. For Temperature = 27°C, around 61.22%, 83.95%, and 86.38% compared to [13], [16], and [18] respectively. For Temperature = 70°C, around 30.89%, 83.96%, and 78.73% compared to [13], [16], and [18] respectively.

## 3) IMPACT OF DIFFERENT FREQUENCIES

Electronic circuits behave very differently at high frequencies because due to a change in the behavior of passive components (resistors, inductors, and capacitors) and parasitic effects on active components, PCB tracks and grounding patterns at high frequencies.

Recently, High-frequency operation is a demand for electronic devices.

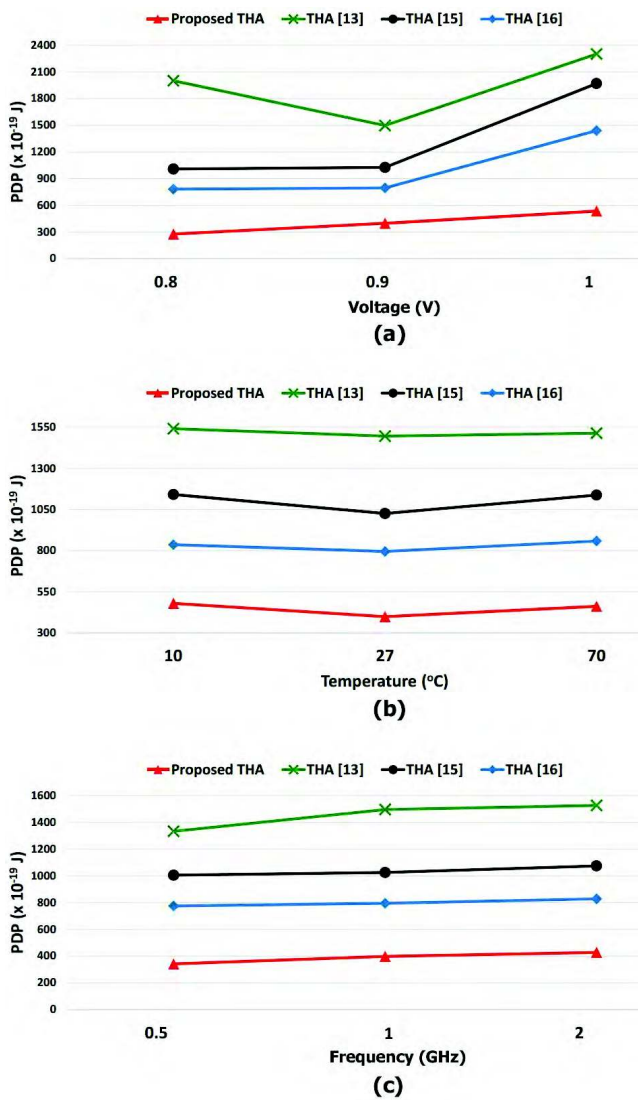

**FIGURE 13.** PDP Comparison of the investigated *THA* for: (a) different power supplies, (b) different temperatures, and (c) different frequencies.

The effect of different frequencies (0.5 GHz, 1 GHz, 2 GHz) on the performance metrics of all proposed circuits is studied. Simulation is done at power supply  $V_{dd}$  equals 0.9 V, and temperature equals 27°C as illustrated in Fig. 11(c).

The comparison of the proposed *STI* demonstrates a notable reduction in PDP as shown in Fig. 11 (c). For frequency = 0.5 GHz, around 40.60%, 86.38%, and 79.93% compared to [13], [16], and [18] respectively. For frequency = 1 GHz, around 61.22%, 83.95%, and 86.38% compared to [13], [16], and [18] respectively. For frequency = 2 GHz, around 30.20%, 63.45%, and 75.52% compared to [13], [16], and [18] respectively.

#### D. COMPARISON OF DIFFERENT *TNAND* CIRCUITS

Fig. 12 shows the PDP Comparison of the investigated *TNAND* for (a) Different Power Supplies, (b) Different Temperatures, and (c) Different Frequencies.

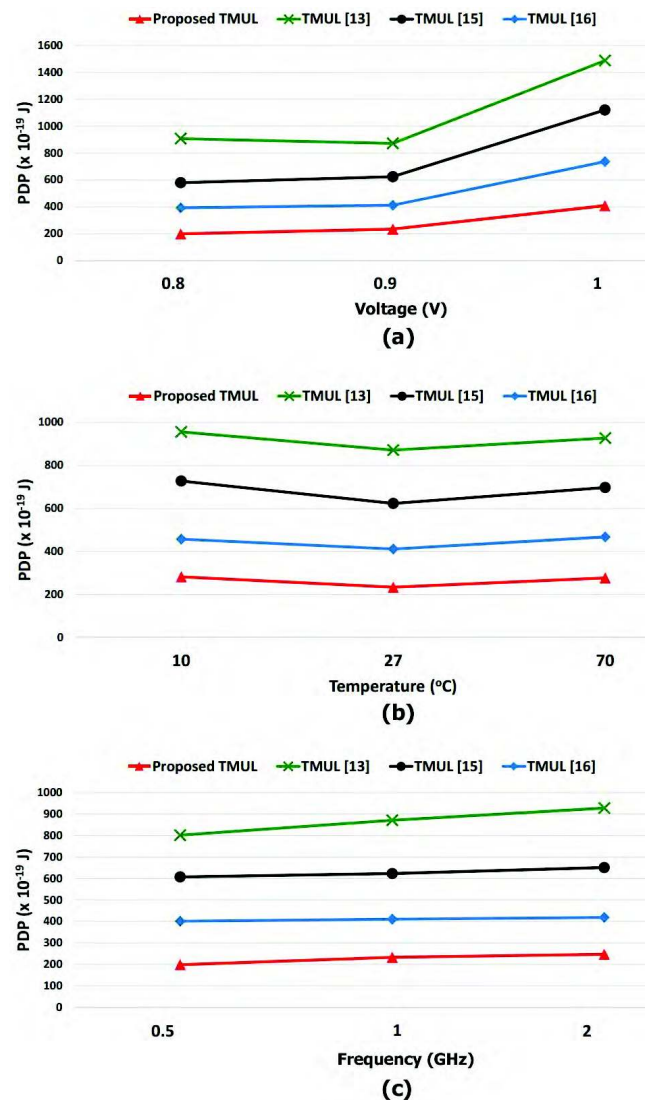

**FIGURE 14.** PDP Comparison of the investigated *TMUL* for: (a) different power supplies, (b) different temperatures, and (c) different frequencies.

#### 1) IMPACT OF DIFFERENT POWER SUPPLIES

Simulation is done at 1 GHz operating frequency and room temperature at 27°C as illustrated in Fig. 12 (a).

The comparison of the proposed *TNAND* demonstrates a notable reduction in PDP as shown in Fig. 12 (a). For  $V_{dd}=0.8$  V, around 32.53%, 99.64%, and 90.07% compared to [13], [16], and [18] respectively. For  $V_{dd}=0.9$  V, around 69.22%, 93.73%, and 94.35% compared to [13], [16], and [18] respectively. For  $V_{dd}=1$  V, around 44.6%, 79.27%, and 98.3% compared to [13], [16], and [18] respectively.

#### 2) IMPACT OF DIFFERENT TEMPERATURES

The effect of different temperatures (10°C, 27°C, 70°C) on the performance metrics of all proposed circuits is studied.

Simulation is done at 1 GHz operating frequency, and power supply  $V_{dd}$  equals 0.9 V as illustrated in Fig. 12 (b).

The comparison of the proposed *TNAND* demonstrates a notable reduction in PDP as shown in Fig. 12 (b).

**TABLE 19.** Comparison of average power ( $\mu\text{W}$ ), maximum delay (ps), and maximum PDP ( $\times 10^{-19}$  J) of 4 TDecoders with  $T = 27^\circ\text{C}$ ,  $F = 1$  GHz, and for different supply voltages.

|                          | Vdd=0.8 V  |             |             | Vdd=0.9 V  |             |             | Vdd=1 V    |             |             |
|--------------------------|------------|-------------|-------------|------------|-------------|-------------|------------|-------------|-------------|
|                          | Power      | Delay       | PDP         | Power      | Delay       | PDP         | Power      | Delay       | PDP         |
| TDecoder [13]            | 2.6        | 10.4        | 2.74        | 3.5        | 8.91        | 3.11        | 11.8       | 8.24        | 9.72        |
| TDecoder [14]            | 1.9        | 8.50        | 1.65        | 2.7        | 7.50        | 2.02        | 10.4       | 7.06        | 7.37        |
| TDecoder [17]            | 126        | 8.67        | 109.24      | 185        | 7.68        | 142.08      | 250        | 7.18        | 168.73      |
| <b>Proposed TDecoder</b> | <b>1.9</b> | <b>6.59</b> | <b>1.26</b> | <b>2.6</b> | <b>6.26</b> | <b>1.62</b> | <b>9.1</b> | <b>4.18</b> | <b>3.82</b> |

**TABLE 20.** Comparison of average power ( $\mu\text{W}$ ), maximum delay (ps), and maximum PDP ( $\times 10^{-19}$  J) of 4 TDecoders with Vdd=0.9 V,  $F = 1$  GHz, and for different temperatures.

|                          | Temp.=10°C |            |             | Temp.=27°C |             |             | Temp.=70°C |             |             |
|--------------------------|------------|------------|-------------|------------|-------------|-------------|------------|-------------|-------------|
|                          | Power      | Delay      | PDP         | Power      | Delay       | PDP         | Power      | Delay       | PDP         |
| TDecoder [13]            | 5.1        | 9.18       | 4.72        | 3.5        | 8.91        | 3.11        | 4.4        | 8.31        | 3.68        |
| TDecoder [14]            | 4.3        | 7.7        | 3.33        | 2.7        | 7.50        | 2.02        | 3.5        | 7.05        | 2.50        |
| TDecoder [17]            | 184        | 7.89       | 145.17      | 185        | 7.68        | 142.08      | 189        | 7.20        | 136.72      |
| <b>Proposed TDecoder</b> | <b>4</b>   | <b>6.4</b> | <b>2.51</b> | <b>2.6</b> | <b>6.26</b> | <b>1.62</b> | <b>3.5</b> | <b>5.85</b> | <b>2.05</b> |

**TABLE 21.** Comparison of average power ( $\mu\text{W}$ ), maximum delay (ps), and maximum PDP ( $\times 10^{-19}$  J) of 4 TDecoders with  $T = 27^\circ\text{C}$ , Vdd=0.9 V, and for different frequencies.

|                          | f= 2 GHz |             |             | f= 1 GHz   |             |             | f= 0.5 GHz |             |             |
|--------------------------|----------|-------------|-------------|------------|-------------|-------------|------------|-------------|-------------|
|                          | Power    | Delay       | PDP         | Power      | Delay       | PDP         | Power      | Delay       | PDP         |
| TDecoder [13]            | 6.0      | 8.93        | 5.17        | 3.5        | 8.91        | 3.11        | 2.3        | 8.91        | 2.11        |
| TDecoder [14]            | 4.1      | 7.54        | 3.12        | 2.7        | 7.50        | 2.02        | 2.0        | 7.5         | 1.46        |
| TDecoder [17]            | 185      | 7.7         | 142.24      | 185        | 7.68        | 142.08      | 184        | 7.68        | 142.08      |
| <b>Proposed TDecoder</b> | <b>4</b> | <b>6.25</b> | <b>2.44</b> | <b>2.6</b> | <b>6.26</b> | <b>1.62</b> | <b>1.8</b> | <b>6.26</b> | <b>1.17</b> |

For Temperature =  $10^\circ\text{C}$ , around 60.88%, 94.09%, and 93.08% compared to [13], [16], and [18] respectively. For Temperature =  $27^\circ\text{C}$ , around 69.22%, 93.73%, and 94.35% compared to [13], [16], and [18] respectively. For Temperature =  $70^\circ\text{C}$ , around 61.34%, 90.13%, and 92.06% compared to [13], [16], and [18] respectively.

### 3) IMPACT OF DIFFERENT FREQUENCIES

The effect of different frequencies (0.5 GHz, 1 GHz, 2 GHz) on the performance metrics of all proposed circuits is studied.

Simulation is done at power supply Vdd equals 0.9 V, and temperature equals  $27^\circ\text{C}$  as illustrated in Fig. 12 (c).

The comparison of the proposed TNAND demonstrates a notable reduction in PDP as shown in Fig. 12 (c). For frequency = 0.5 GHz, around 71.46%, 94.18%, and 94.79% compared to [13], [16], and [18] respectively. For frequency = 1 GHz, around 69.22%, 93.73%, and 94.35% compared to [13], [16], and [18] respectively. For frequency = 2 GHz, around 61.27%, 92.23%, and 92.66% compared to [13], [16], and [18] respectively.

## E. COMPARISON OF DIFFERENT TDECODER CIRCUITS

### 1) IMPACT OF DIFFERENT POWER SUPPLIES

Table 19 shows the comparison to the existing Ternary Decoder in [13], [14], and [17] in terms of the average power consumption, maximum propagation delay, and maximum energy (PDP) for different supply voltages (0.8 V, 0.9 V, 1 V), same temperature ( $27^\circ\text{C}$ ), and same frequency (1 GHz). The boldface values are the best values among others.

The comparison of the proposed Ternary Decoder demonstrates a notable reduction in PDP as shown in Table 19. For Vdd=0.8 V, around 54.01%, 23.64%, and 98.85% compared to [13], [14], and [17] respectively. For Vdd=0.9 V, around 47.91%, 19.8%, and 98.86% compared to [13], [14], and [17] respectively. For Vdd=1 V, around 60.7%, 48.17%, and 97.74% compared to [13], [14], and [17] respectively.

### 2) IMPACT OF DIFFERENT TEMPERATURES

Table 20 shows the comparison to the existing Ternary Decoder in [13], [14], and [17] in terms of the average power consumption, maximum propagation delay, and maximum energy (PDP) for different temperatures ( $10^\circ\text{C}$ ,  $27^\circ\text{C}$ ,  $70^\circ\text{C}$ ), same supply voltage Vdd (0.9 V), and same frequency (1 GHz).

The comparison of the proposed Ternary Decoder demonstrates a notable reduction in PDP as shown in Table 20. For Temperature =  $10^\circ\text{C}$ , around 46.82%, 24.62%, and 98.27% compared to [13], [14], and [17] respectively. For Temperature =  $27^\circ\text{C}$ , around 47.91%, 19.8%, and 98.86% compared to [13], [14], and [17] respectively. For Temperature =  $70^\circ\text{C}$ , around 44.29%, 18%, and 98.5% compared to [13], [14], and [17] respectively.

### 3) IMPACT OF DIFFERENT FREQUENCIES

Table 21 shows the comparison to the existing Ternary Decoder in [13], [14], and [17] in terms of the average power consumption, maximum propagation delay, and maximum energy (PDP) for different frequencies (0.5 GHz, 1 GHz,

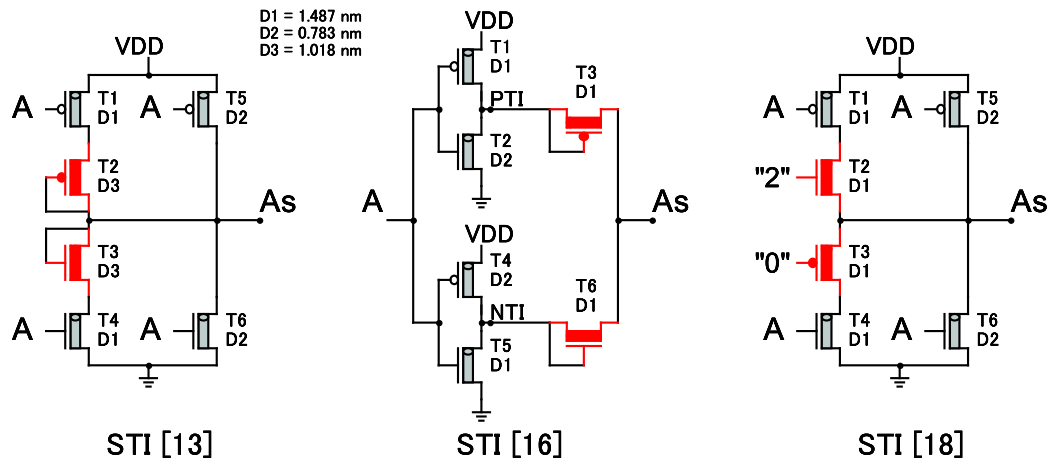

FIGURE 15. Existing STI in (a) [13], (b) [16], and (c) [18].

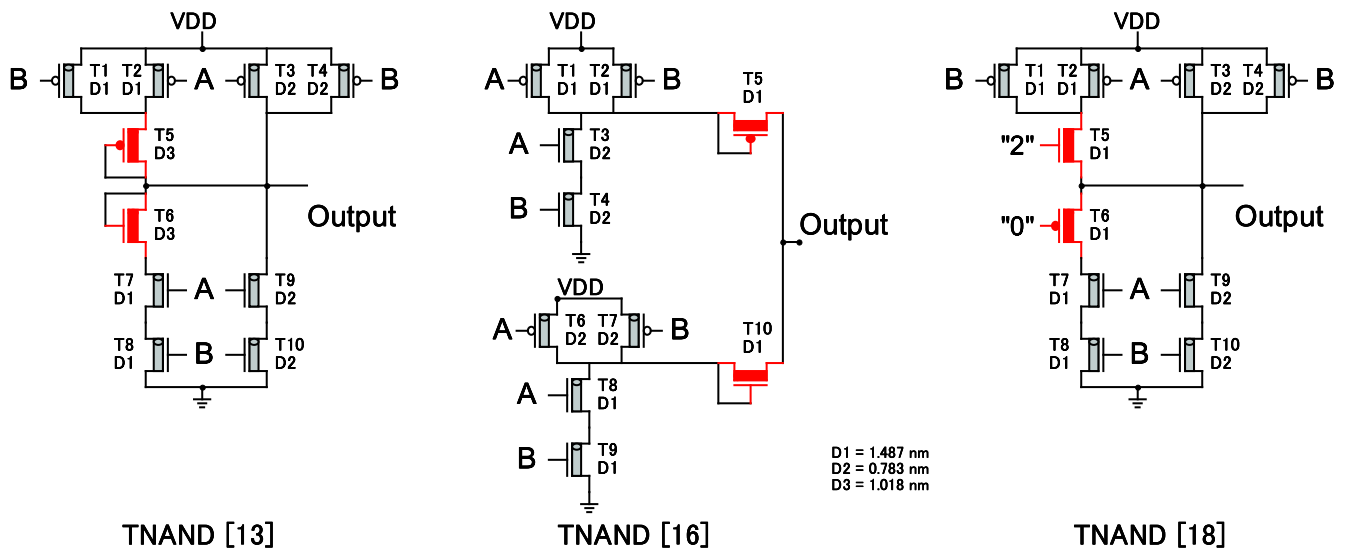

FIGURE 16. Existing TNAND in (a) [13], (b) [16], and (c) [18].

2 GHz), same temperatures (27°C), and same supply voltage Vdd (0.9 V).

The comparison of the proposed Ternary Decoder demonstrates a notable reduction in PDP as shown in Table 21. For frequency = 2 GHz, around 52.8%, 21.79%, and 98.28% compared to [13], [14], and [17] respectively. For frequency = 1 GHz, around 47.91%, 19.8%, and 98.86% compared to [13], [14], and [17] respectively. For frequency = 0.5 GHz, around 44.55%, 19.86%, and 99.18% compared to [13], [14], and [17] respectively.

#### F. COMPARISON OF DIFFERENT THA CIRCUITS

Fig. 13 shows the PDP Comparison of the investigated THA for (a) Different Power Supplies, (b) Different Temperatures, and (c) Different Frequencies.

##### 1) IMPACT OF DIFFERENT POWER SUPPLIES

Simulation is done at 1 GHz operating frequency and room temperature at 27°C as illustrated in Fig. 13 (a).

The comparison of the proposed THA demonstrates a notable reduction in PDP as shown in Fig. 13 (a). For Vdd=0.8 V, around 86.16%, 72.53%, and 64.55% compared to [13], [15], and [16] respectively. For Vdd=0.9 V, around 73.43%, 61.24%, and 49.97% compared to [13], [15], and [16] respectively. For Vdd=1 V, around 76.75%, 72.82%, and 62.85% compared to [13], [15], and [16] respectively.

##### 2) IMPACT OF DIFFERENT TEMPERATURES

The effect of different temperatures (10°C, 27°C, 70°C) on the performance metrics of all proposed circuits is studied.

Simulation is done at 1 GHz operating frequency, and power supply Vdd equals 0.9 V as illustrated in Fig. 13 (b).

The comparison of the proposed THA demonstrates a notable reduction in PDP as shown in Fig. 13 (b). For Temperature = 10°C, around 68.97%, 58.08%, and 42.78% compared to [13], [15], and [16] respectively. For Temperature = 27°C, around 73.43%, 61.24%, and 49.97% compared to [13], [15], and [16] respectively.



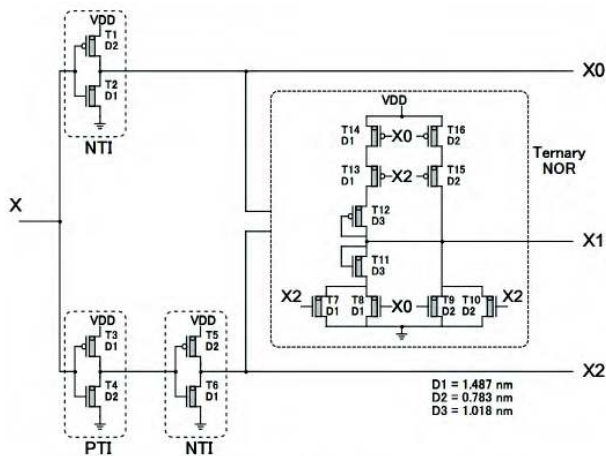

(a) TDECODER [13] with 16 Transistors

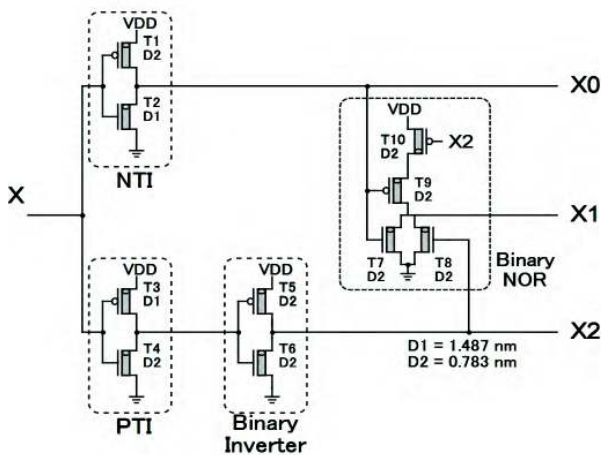

(b) TDECODER [14] with 10 Transistors

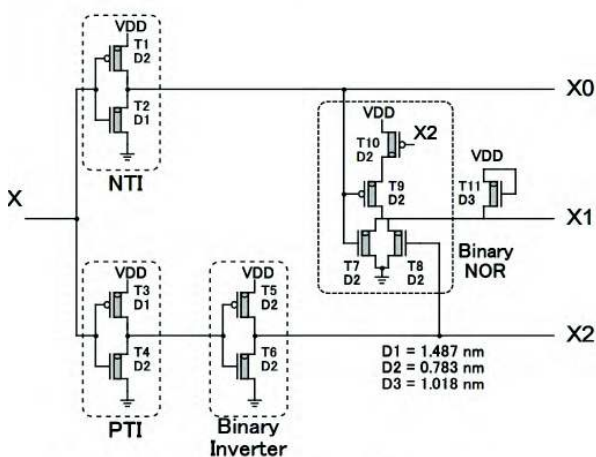

(c) TDECODER [17] with 11 Transistors

FIGURE 17. Existing TDecoder in (a) [13], (b) [14], and (c) [17].

to [13], [15], and [16] respectively. For Temperature = 70°C, around 69.58%, 59.51%, and 46.28% compared to [13], [15], and [16] respectively.

### 3) IMPACT OF DIFFERENT FREQUENCIES

The effect of different frequencies (0.5 GHz, 1 GHz, 2 GHz) on the performance metrics of all proposed circuits is studied.

Simulation is done at power supply Vdd equals 0.9 V, and temperature equals 27°C as illustrated in Fig. 13 (c).

The comparison of the proposed *THA* demonstrates a notable reduction in PDP as shown in Fig. 13 (c). For frequency = 0.5 GHz, around 74.4%, 66.04%, and 55.94% compared to [13], [15], and [16] respectively. For frequency = 1 GHz, around 73.43%, 61.24%, and 49.97% compared to [13], [15], and [16] respectively. For frequency = 2 GHz, around 72.01%, 60.22%, and 48.4% compared to [13], [15], and [16] respectively.

### G. COMPARISON OF DIFFERENT TMUL CIRCUITS

Fig. 14 shows the PDP Comparison of the investigated *TMUL* for (a) Different Power Supplies, (b) Different Temperatures, and (c) Different Frequencies.

#### 1) IMPACT OF DIFFERENT POWER SUPPLIES

Simulation is done at 1 GHz operating frequency and room temperature at 27°C as illustrated in Fig. 14 (a).

The comparison of the proposed *TMUL* demonstrates a notable reduction in PDP as shown in Fig. 14 (a). For Vdd=0.8 V, around 78.16%, 65.77%, and 49.49% compared to [13], [15], and [16] respectively. For Vdd=0.9 V, around 73.19%, 62.52%, and 43.19% compared to [13], [15], and [16] respectively. For Vdd=1 V, around 72.58%, 63.58%, and 44.55% compared to [13], [15], and [16] respectively.

#### 2) IMPACT OF DIFFERENT TEMPERATURES

The effect of different temperatures (10°C, 27°C, 70°C) on the performance metrics of all proposed circuits is studied.

Simulation is done at 1 GHz operating frequency, and power supply Vdd equals 0.9 V as illustrated in Fig. 14 (b).

The comparison of the proposed *TMUL* demonstrates a notable reduction in PDP as shown in Fig. 14 (b). For Temperature = 10°C, around 70.51%, 61.25%, and 38.36% compared to [13], [15], and [16] respectively. For Temperature = 27°C, around 73.19%, 62.52%, and 43.19% compared to [13], [15], and [16] respectively. For Temperature = 70°C, around 70.17%, 60.32%, and 40.82% compared to [13], [15], and [16] respectively.

#### 3) IMPACT OF DIFFERENT FREQUENCIES

The effect of different frequencies (0.5 GHz, 1 GHz, 2 GHz) on the performance metrics of all proposed circuits is studied.

Simulation is done at power supply Vdd equals 0.9 V, and temperature equals 27°C as illustrated in Fig. 14 (c).

The comparison of the proposed *TMUL* demonstrates a notable reduction in PDP as shown in Fig. 14 (c). For frequency = 0.5 GHz, around 75.15%, 67.2%, and 50.38% compared to [13], [15], and [16] respectively. For frequency = 1 GHz, around 73.19%, 62.52%, and 43.19% compared to [13], [15], and [16] respectively.



For frequency = 2 GHz, around 73.31%, 61.97%, and 40.91% compared to [13], [15], and [16] respectively.

The **advantage** of all proposed circuits is that they have the lowest PDP among all investigated circuits for different supply voltages, temperatures, and frequencies. Therefore, they are more suitable for low-power portable electronics and embedded systems to save battery consumption.

## VI. CONCLUSION

This paper proposed new designs for the Standard Ternary Inverter, Ternary NAND, Ternary Decoder, Ternary Half Adder, and Ternary Multiplier that aim to keep high-performance levels and energy efficiency.

The design process tried to optimize several circuit techniques such as reducing the number of used transistors,

utilizing energy-efficient transistor arrangements, and applying the dual supply voltages ( $V_{dd}$  and  $V_{dd}/2$ ).

The proposed ternary circuits are compared to the latest fifteen ternary circuits, simulated and tested using HSPICE simulator under various operating conditions with different supply voltages, different temperatures, and different frequencies.

One hundred eighty simulations are performed to prove the efficiency of the proposed designs. The results prove the merits of the approach in terms of reduced energy consumption (PDP) compared to other existing designs.

Therefore, the proposed circuits can be implemented in low-power portable electronics and embedded systems to save battery consumption.

## APPENDIX

### INVESTIGATED CIRCUITS FROM THE LITERATURE

See Figs. 15–19.

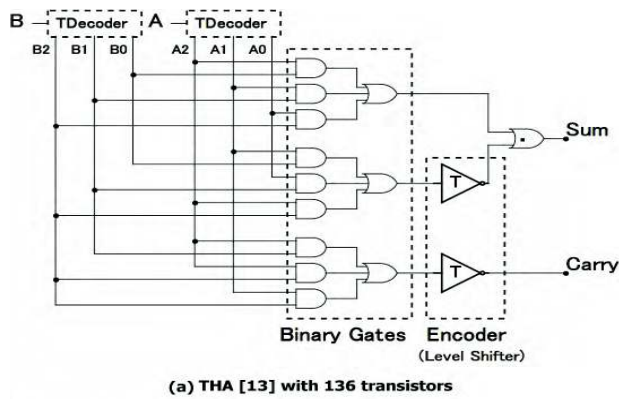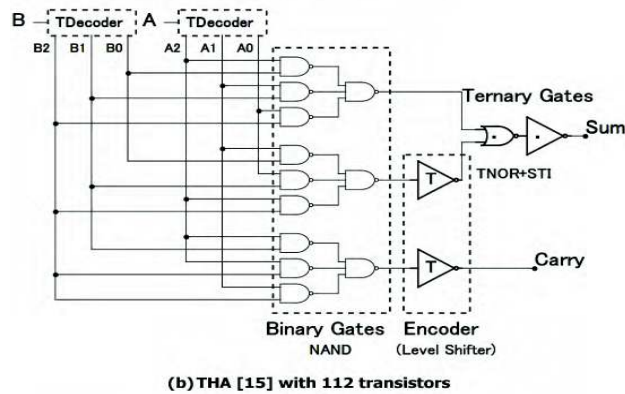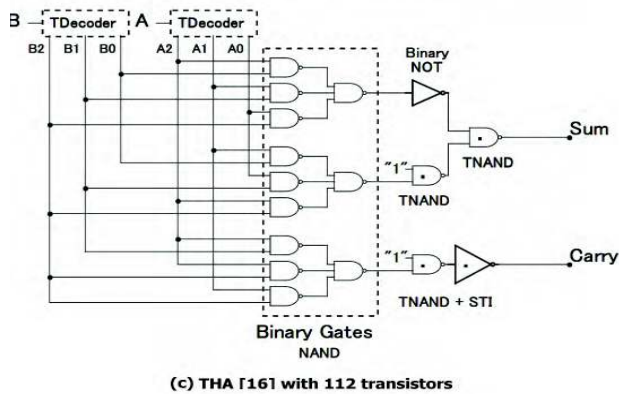

FIGURE 18. Existing THA in (a) [13], (b) [15], and (c) [16].

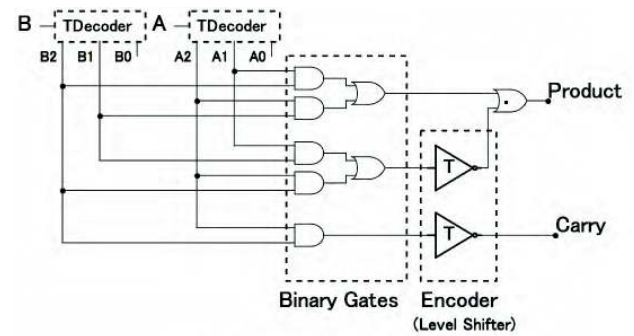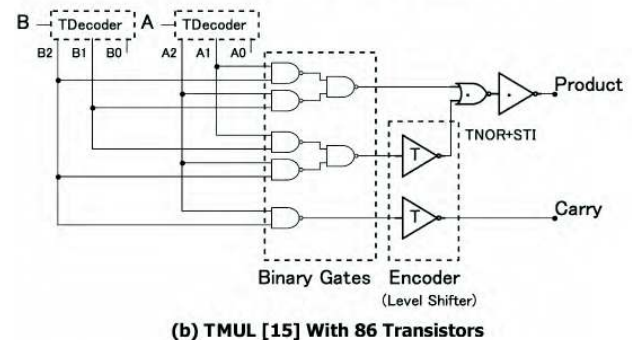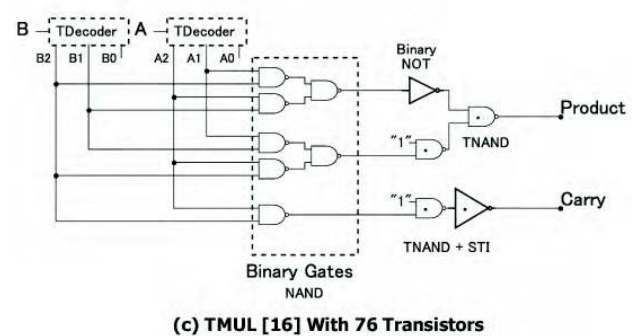

FIGURE 19. Existing TMUL in (a) [13], (b) [15], and (c) [16].

## REFERENCES

- [1] K. You and K. Nepal, "Design of a ternary static memory cell using carbon nanotube-based transistors," *IET Micro Nano Lett.*, vol. 6, no. 6, pp. 381–385, Jun. 2011. doi: [10.1049/mnl.2011.0168](https://doi.org/10.1049/mnl.2011.0168).
- [2] J.-M. Philippe, E. Kinvi-Boh, S. Pillement, and O. Sentieys, "An energy-efficient ternary interconnection link for asynchronous systems," in *Proc. IEEE Int. Symp. Circuits Syst. (ISCAS)*, Island of Kos, Greece, May 2006, pp. 1011–1014.
- [3] S. L. Hurst, "Multiple-valued logic—Its status and its future," *IEEE Trans. Comput.*, vol. C-33, no. 12, pp. 1160–1179, Dec. 1984. doi: [10.1109/TC.1984.1676392](https://doi.org/10.1109/TC.1984.1676392).
- [4] D. M. Miller and M. Soeken, "A spectral algorithm for ternary function classification," in *Proc. IEEE 48th Int. Symp. Multiple-Valued Log. (ISMVL)*, Linz, Austria, May 2018, pp. 198–203.
- [5] P. Reviriego, S. Pontarelli, and A. Ullah, "Error detection and correction in SRAM emulated TCAMs," *IEEE Trans. Very Large Scale Integr. (VLSI) Syst.*, vol. 27, no. 2, pp. 486–490, Feb. 2019. doi: [10.1109/TVLSI.2018.2877131](https://doi.org/10.1109/TVLSI.2018.2877131).
- [6] M. R. Khezeli, M. H. Moaiyeri, and A. Jalali, "Comparative analysis of simultaneous switching noise effects in MWCNT bundle and Cu power interconnects in CNTFET-based ternary circuits," *IEEE Trans. Very Large Scale Integr. (VLSI) Syst.*, vol. 27, no. 1, pp. 37–46, Jan. 2019. doi: [10.1109/TVLSI.2018.2869761](https://doi.org/10.1109/TVLSI.2018.2869761).
- [7] H. Oseily and A. M. Haidar, "Hexadecimal to binary conversion using multi-input floating gate complementary metal oxide semiconductors," in *Proc. Int. Conf. Appl. Res. Comput. Sci. Eng. (ICAR)*, Beirut, Lebanon, Oct. 2015, pp. 1–6.
- [8] A. I. Khan, N. Nusrat, S. M. Khan, and M. Hasan, "Novel realization of quantum ternary Mux and Demux," in *Proc. Int. Conf. Elect. Comput. Eng., Dhaka, Bangladesh*, Dec. 2006, pp. 153–156.
- [9] N. Saleh, A. Kassem, and A. M. Haidar, "Energy-Efficient architecture for wireless sensor networks in healthcare applications," *IEEE Access*, vol. 6, pp. 6478–6486, 2018. doi: [10.1109/ACCESS.2018.2789918](https://doi.org/10.1109/ACCESS.2018.2789918).
- [10] M. Irfan and Z. Ullah, "G-AETCAM: Gate-based area-efficient ternary content-addressable memory on FPGA," *IEEE Access*, vol. 5, pp. 20785–20790, 2017. doi: [10.1109/ACCESS.2017.2756702](https://doi.org/10.1109/ACCESS.2017.2756702).
- [11] R. Jaber, A. El-hajj, L. Nimri, and A. Haidar, "A Novel implementation of ternary decoder using CMOS DPL binary gates," in *Proc. Int. Arab Conf. Inf. Technol. (ACIT)*, Werdanyeh, Lebanon, Nov. 2018, pp. 1–3.
- [12] K. Jyoti and S. Narkhede, "An approach to ternary logic gates using FinFET," in *Proc. Int. Conf. Adv. Inf. Commun. Technol. Comput. (AICTC)*, Bikaner, India, 2016, p. 59.
- [13] S. Lin, Y. B. Kim, and F. Lombardi, "CNTFET-based design of ternary logic gates and arithmetic circuits," *IEEE Trans. Nanotechnol.*, vol. 10, no. 2, pp. 217–225, Mar. 2011. doi: [10.1109/TNANO.2009.2036845](https://doi.org/10.1109/TNANO.2009.2036845).
- [14] K. Sridharan, S. Gurindagunta, and V. Pudi, "Efficient multiterinary digit adder design in CNTFET technology," *IEEE Trans. Nanotechnol.*, vol. 12, no. 3, pp. 283–287, Mar. 2013. doi: [10.1109/TNANO.2013.2251350](https://doi.org/10.1109/TNANO.2013.2251350).
- [15] M. Muglikar, R. Sahoo, and S. K. Sahoo, "High performance ternary adder using CNTFET," in *Proc. 3rd Int. Conf. Devices, Circuits Syst. (ICDCS)*, Coimbatore, India, Mar. 2016, pp. 236–239.
- [16] H. Samadi, A. Shahhoseini, and F. Aghaei-liavali, "A new method on designing and simulating CNTFET\_based ternary gates and arithmetic circuits," *Microelectron. J.*, vol. 63, pp. 41–48, May 2017. doi: [10.1016/j.mejo.2017.02.018](https://doi.org/10.1016/j.mejo.2017.02.018).
- [17] P. Wang, D. Gong, Y. Zhang, and Y. Kang, "Ternary 2-9 line address decoder realized by CNFET," U.S. Patent 20180182450 A1, Jun. 28, 2018.
- [18] S. Tabrizchi, M. R. Taheri, K. Navi, and N. Bagherzadeh, "Novel CNFET ternary circuit techniques for high-performance and energy-efficient design," *IET Circuits, Devices Syst.*, vol. 13, no. 2, pp. 193–202, Mar. 2019. doi: [10.1049/iet-cds.2018.5036](https://doi.org/10.1049/iet-cds.2018.5036).
- [19] G. Hills et al., "Understanding energy efficiency benefits of carbon nanotube field-effect transistors for digital VLSI," *IEEE Trans. Nanotechnol.*, vol. 17, no. 6, pp. 1259–1269, Nov. 2018. doi: [10.1109/TNANO.2018.2871841](https://doi.org/10.1109/TNANO.2018.2871841).
- [20] Stanford, CA, USA. *Stanford University CNFET Model Website*. Accessed: May 1, 2019. [Online]. Available: <http://nano.stanford.edu/model.php?id=23>
- [21] J. Deng and H.-S. P. Wong, "A compact SPICE model for carbon-nanotube field-effect transistors including nonidealities and its application—Part I: Model of the intrinsic channel region," *IEEE Trans. Electron Devices*, vol. 54, no. 12, pp. 3186–3194, Dec. 2007. doi: [10.1109/TED.2007.909030](https://doi.org/10.1109/TED.2007.909030).
- [22] J. Deng and H.-S. P. Wong, "A compact SPICE model for carbon-nanotube field-effect transistors including nonidealities and its application—Part II: Full device model and circuit performance benchmarking," *IEEE Trans. Electron Devices*, vol. 54, no. 12, pp. 3195–3205, Dec. 2007. doi: [10.1109/TED.2007.909043](https://doi.org/10.1109/TED.2007.909043).

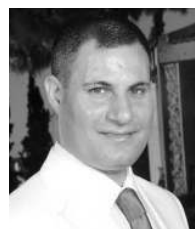

**RAMZI A. JABER** (S'19) received the B.E. degree (Hons.) in computer and electrical engineering and the master's degree in computer engineering and informatics from Beirut Arab University (BAU), in 2001 and 2010, respectively, where he is currently pursuing the Ph.D. degree in computer and electrical engineering.

From 2002 to 2006, he taught at different high schools at Lebanon. From 2006 to 2010, he taught as a Lab Instructor in the Faculty of Computer Sciences, Lebanese University. From 2006 to 2019, he taught as a Lab Instructor and Lecturer in the Computer and Electrical Engineering Department, Beirut Arab University (BAU). He has been a Cisco Certified Network Associate (CCNA) Instructor, since 2011. His current research interests include high-performance and energy-efficient digital circuit design, as well as high-speed low-power very large-scale integrated (VLSI) circuit design and multiple-valued logic (MVL).

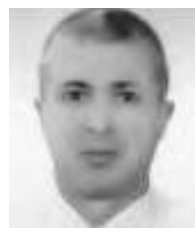

**ABDALLAH KASSEM** (S'98–M'02–SM'11) received the B.S. degree in microelectronics from the University of Quebec in Montreal, in 1992, and the M.Sc. and Ph.D. degrees in microelectronics from the École Polytechnique de Montréal, in 1996 and 2004, respectively. From 1996 to 2000, he taught some courses and laboratories as an Instructor in his field at AUB, LAU, Lebanon. He joined the Electrical and Computer Engineering Department, Notre Dame University, Lebanon,

as an Assistant Professor, where he was promoted to Associate Professor, in 2011. His research interests include microelectronics design and testing, VLSI, semiconductor device modeling and simulation, microprocessors, engineering education/management, ultrasonic applications, healthcare applications, biomedical system design, smart medical devices e-Health, and m-Health. He has published approximately 60 papers in reviewed journals and conference proceedings in Lebanon and around the world. He is an Associate Editor of the IEEE Access and a Guest Editor *AEU—International Journal of Electronics and Communications* (Elsevier). He was a member of the organizing committee of many international conferences sponsored or technically co-sponsored by IEEE (DINWC 2018, EBECEGC 2018, ICM, ICABME, MECBME, ACTEA, ICDIPC 2016, EECEA 2016, DICTAP 2015, TAECE 2015, ICABME 2015, ICeND2014, and MELECON). He was invited as a keynote speaker in some conferences and workshops.

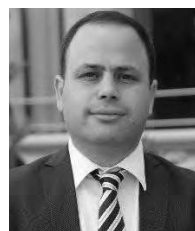

**AHMAD M. EL-HAJJ** (S'05–M'16) received the B.E., M.E., and Ph.D. degrees in electrical and computer engineering from the American University of Beirut, in 2007, 2009, and 2014, respectively. He is currently an Assistant Professor in the communications and electronics program and the Coordinator of the biomedical engineering program with Beirut Arab University. His research interests include wireless network optimization, radio network planning, game theory, neuro-engineering, biomimetics, and bioinformatics. He serves as a member of the Executive Committee of the IEEE-Lebanon Section and the Local Chapter of the IEEE Communications Society (IEEE ComSoc).

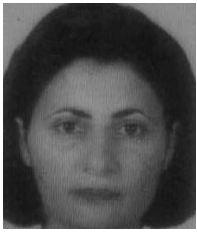

**LINA A. EL-NIMRI** received the Diploma degree in computer engineering from the Leningrad Electrotechnical Institute (LETI), in 1983, and the Ph.D. degree in technical sciences “computers, complexes, and systems” from Saint-Petersburg Electrotechnical University (ETU), in 1994. From 1983 to 1989, she was an Analyst, a Programmer, and a System Administrator in several companies, where she developed business applications and applications for production and analysis purposes.

While conducting her Ph.D. research, she was also working at the university’s computer laboratory, where she designed and programmed a parametric system for the simulation of processes and their interactions.

She has taught in Beirut Arab University (BAU), the Institut Supérieur des Sciences Appliquées et Économiques (ISAE-Cnam Liban), and the Islamic University of Lebanon (IUL), and since 1999, she has been, and continues to be, an Associate Professor with Lebanese University.

Her scientific interests and teaching experiences are focused on the following areas: simulation, logic design, operating systems, compilation theory, database theory, programming languages, system analysis and design, web development, web services, multimedia, big data, and information retrieval. Besides teaching, she has advised and supervised many students in their graduation projects and master’s theses.

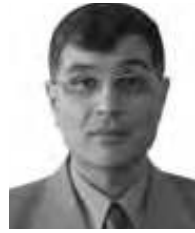

**ALI MASSOUD HAIDAR** received the B.S. degree in electrical engineering (electronics and telecommunications) from Beirut Arab University, in 1986, the M.E. degree in computer and information engineering from the Faculty of Engineering, University of the Ryukyus, Japan, in 1992, and the Ph.D. degree in computer engineering from the Department of Computer and Information Engineering, Faculty of Engineering, Saitama University, Japan, in 1995. He joined Hiroshima City

University, in 1995, as an Assistant Professor. Then, he joined Beirut Arab University, in 1997, where he is currently a Professor with the Department of Electrical and Computer Engineering. His scientific interests include logic theory and its applications, neural networks, Petri nets, cloud computing, digital communication, and smart grids. He published approximately 100 papers in reviewed journals and conference proceedings. He has supervised around 25 graduate students (master’s and Ph.D.).

...
